# Supplementary material for: RoSplat: Robust Feed-Forward Pixel-wise Gaussian Splatting for Varying Input Views and High-Resolution Rendering
Source: arXiv:2605.13093 source file (2026-05-13)
Supplement: Supplementary file 1 [file more_analysis.tex]

\section{More Analysis on the Over-Brightness Issue}
\label{sec:more_analysis_overbrightness}

To provide further evidence for the over-brightness analysis in the main paper, examine how the following three quantities produced by existing works~\cite{chen2024mvsplat, zhang2025transplat, xu2025depthsplat} vary with the number of input views: (i) the pixel intensity of the rendered image, (ii) the accumulated compositing weight $W=\sum_j w_j(\mathbf{p})$, and (iii) the rendering quality measured by PSNR. Specifically, for each method and input-view count in Fig.~\ref{fig:alpha_norm_curve}, we compute pixel-wise statistics on a rendered target image and summarize them using the median over all pixels. For the first row in the figure, we convert the rendered image to grayscale, then compute the median grayscale intensity. We then evaluate the accumulated compositing weight at each pixel as $W(\mathbf p)=\sum_j w_j(\mathbf p)$, and report its median value across all pixels (second row). PSNR is computed between the rendered image and the ground-truth target image (third row). Finally, we count the number of Gaussians contributing to each pixel and report the median count (fourth row). 

The figure reveals a consistent pattern across all three methods. As the number of input views increases, the number of contributing Gaussians also increases (last row of Fig.~\ref{fig:alpha_norm_curve}), indicating that more Gaussians overlap on the same underlying scene regions. This increase in overlap is accompanied by a monotonic increase in the accumulated compositing weight $W$ (second row of Fig.~\ref{fig:alpha_norm_curve}), leading to a monotonic increase in the pixel intensity (first row of Fig.~\ref{fig:alpha_norm_curve}), a degradation in the image quality~(third row of Fig.~\ref{fig:alpha_norm_curve}). Moreover, the largest PSNR drop is consistently observed when the increase in $W$ is the most pronounced, while the degradation becomes less severe once $W$ saturates near $1$. These observations provide strong empirical support for the analysis in the main paper (Sec. 4.1): the over-brightness issue mainly arises because increasing the number of input views produces more overlapping Gaussians, which increases the accumulated compositing weight and leads to degraded rendering quality.

In contrast, after applying our alpha normalization, the accumulated compositing weight remains much more stable across different input-view counts. As a result, the rendered pixel intensity also stays more consistent, and the rendering quality is significantly improved compared to without alpha normalization. This demonstrates that stabilizing the accumulated compositing weight is an effective way to mitigate the over-brightness issue and improve robustness under varying input-view counts.

\begin{table}[t]
\centering
\footnotesize
\caption{\textbf{Cross-dataset evaluation}. Both methods are trained on the RealEstate dataset with two input images of $256\times 448$ resolution. We evaluate the models on the DL3DV dataset using (1) the same configuration as training, (2) increase the number of input views to 6, (3) increase the rendering resolution to $2048\times 3584$ resolution.}
% \resizebox{\textwidth}{!}{
\begin{tblr}{
  colsep  = 1.5pt,
  rowsep  = 1pt,
  % 1 left-aligned column for methods, 9 fixed-width centered columns for metrics
  colspec = {l *{9}{Q[c, wd=4em]}}, 
  % Define column spans for the group headers
  cell{1}{2} = {c=3}{c},
  cell{1}{5} = {c=3}{c},
  cell{1}{8} = {c=3}{c},
  % Solid vertical lines to separate the method column and the three main groups
  vline{2,5,8} = {solid},
  % Solid horizontal lines for clean structure
  hline{3,5} = {solid},   % Top border, under headers, and bottom border
  % hline{2} = {1-10}{solid}, % Border exactly underneath the view count headers
}
& 2 views, $256 \times 448$ & & & 6 views, $256 \times 448$ & & & 6 views, $2048 \times 3584$ & & \\

& PSNR $\uparrow$  & SSIM $\uparrow$  & LPIPS $\downarrow$ & PSNR $\uparrow$  & SSIM $\uparrow$  & LPIPS $\downarrow$ & PSNR $\uparrow$  & SSIM $\uparrow$ & LPIPS $\downarrow$\\

DepthSplat & 17.50 & 0.562 & \textbf{0.360} & 19.64 & 0.670 & 0.287 & 16.80 & 0.600 & 0.543 \\

Ours & \textbf{17.51} & \textbf{0.567} & 0.362 & \textbf{20.64} & \textbf{0.708} & \textbf{0.27} & \textbf{17.58} & \textbf{0.686} & \textbf{0.521} \\

& \textcolor{Green}{+0.01} & \textcolor{Green}{+0.005} & \textcolor{orange}{+0.002} & \textcolor{Green}{+1.00} & \textcolor{Green}{+0.038} & \textcolor{Green}{-0.017} & \textcolor{Green}{+0.78} & \textcolor{Green}{+0.086} & \textcolor{Green}{-0.022} \\
\end{tblr}
% }
\label{tab:cross_dataset_evaluation}
\end{table}

\begin{table}[t]
\centering
\scriptsize
\caption{\textbf{Comparison on the DL3DV dataset under zoom-in rendering}. Our method significantly outperforms DepthSplat, and the performance gaps increases as the zoom-in factor increases.}
\resizebox{\textwidth}{!}{%
\begin{tblr}{
  colsep  = 1.5pt,
  rowsep  = 1pt,
  column{even} = {c},
  column{3} = {c},
  column{5} = {c},
  column{7} = {c},
  column{9} = {c},
  column{11} = {c},
  column{13} = {c},
  cell{1}{2} = {c=3}{},
  cell{1}{6} = {c=3}{},
  cell{1}{9} = {c=3}{},
  cell{1}{12} = {c=3}{},
  cell{3}{2} = {font=\bfseries},
  cell{3}{3} = {font=\bfseries},
  cell{3}{4} = {font=\bfseries},
  cell{4}{6} = {font=\bfseries},
  cell{4}{7} = {font=\bfseries},
  cell{4}{8} = {font=\bfseries},
  cell{4}{9} = {font=\bfseries},
  cell{4}{10} = {font=\bfseries},
  cell{4}{11} = {font=\bfseries},
  cell{4}{12} = {font=\bfseries},
  cell{4}{13} = {font=\bfseries},
  cell{4}{14} = {font=\bfseries},
  vline{2} = {1}{Black},
  vline{3,6-7,10,13} = {1}{},
  vline{2,5-6,9,12} = {1-5}{Black},
  hline{3} = {1,4,6,8,11,14}{},
  hline{3} = {2-3,7,9-10,12-13}{Black},
  hline{5} = {1,4,6,8,11,14}{},
  hline{5} = {2-3,7,9-10,12-13}{Black}
}
           & $1\times$ zoom-in &        &       &   & $2\times$ zoom-in  &       &        & $4\times$ zoom-in  &       &        & $8\times$ zoom-in  &       &        \\
           & PSNR $\uparrow$        & SSIM $\uparrow$  & LPIPS $\downarrow$ & ~ & PSNR $\uparrow$           & SSIM $\uparrow$ & LPIPS $\downarrow$ & PSNR $\uparrow$            & SSIM $\uparrow$ & LPIPS $\downarrow$ & PSNR $\uparrow$           & SSIM $\uparrow$  & LPIPS  $\downarrow$  \\
DepthSplat & 24.17 & 0.819 & 0.145 & & 19.95 & 0.676 & 0.272 & 17.05 & 0.528 & 0.436 & 16.07 & 0.512 & 0.511  \\
Ours        & 24.10 & 0.818 & 0.147 & & 20.84 & 0.692 & 0.263 & 18.79 & 0.587 & 0.398 & \textbf{18.19} & \textbf{0.586} & \textbf{0.477}  \\
~           & \textcolor{orange}{-0.07} & \textcolor{orange}{-0.001} & \textcolor{orange}{+0.002} & & \textcolor{Green}{+0.89} & \textcolor{Green}{+0.016} & \textcolor{Green}{-0.009} & \textcolor{Green}{+1.74} & \textcolor{Green}{+0.059} & \textcolor{Green}{-0.038} & \textcolor{Green}{+2.12} & \textcolor{Green}{+0.074} & \textcolor{Green}{-0.034} 
\end{tblr}
}
\label{tab:zoomed_in_comparision}
\end{table}

\begin{figure}[t]
\centering

    \begin{tabular}{ccc}
    \multicolumn{1}{c}{{MVSplat~\cite{chen2024mvsplat}}} &
    \multicolumn{1}{c}{{TranSplat~\cite{zhang2025transplat}}} &
    \multicolumn{1}{c}{{DepthSplat~\cite{xu2025depthsplat}}} \\
    
    \includegraphics[width=0.32\linewidth]{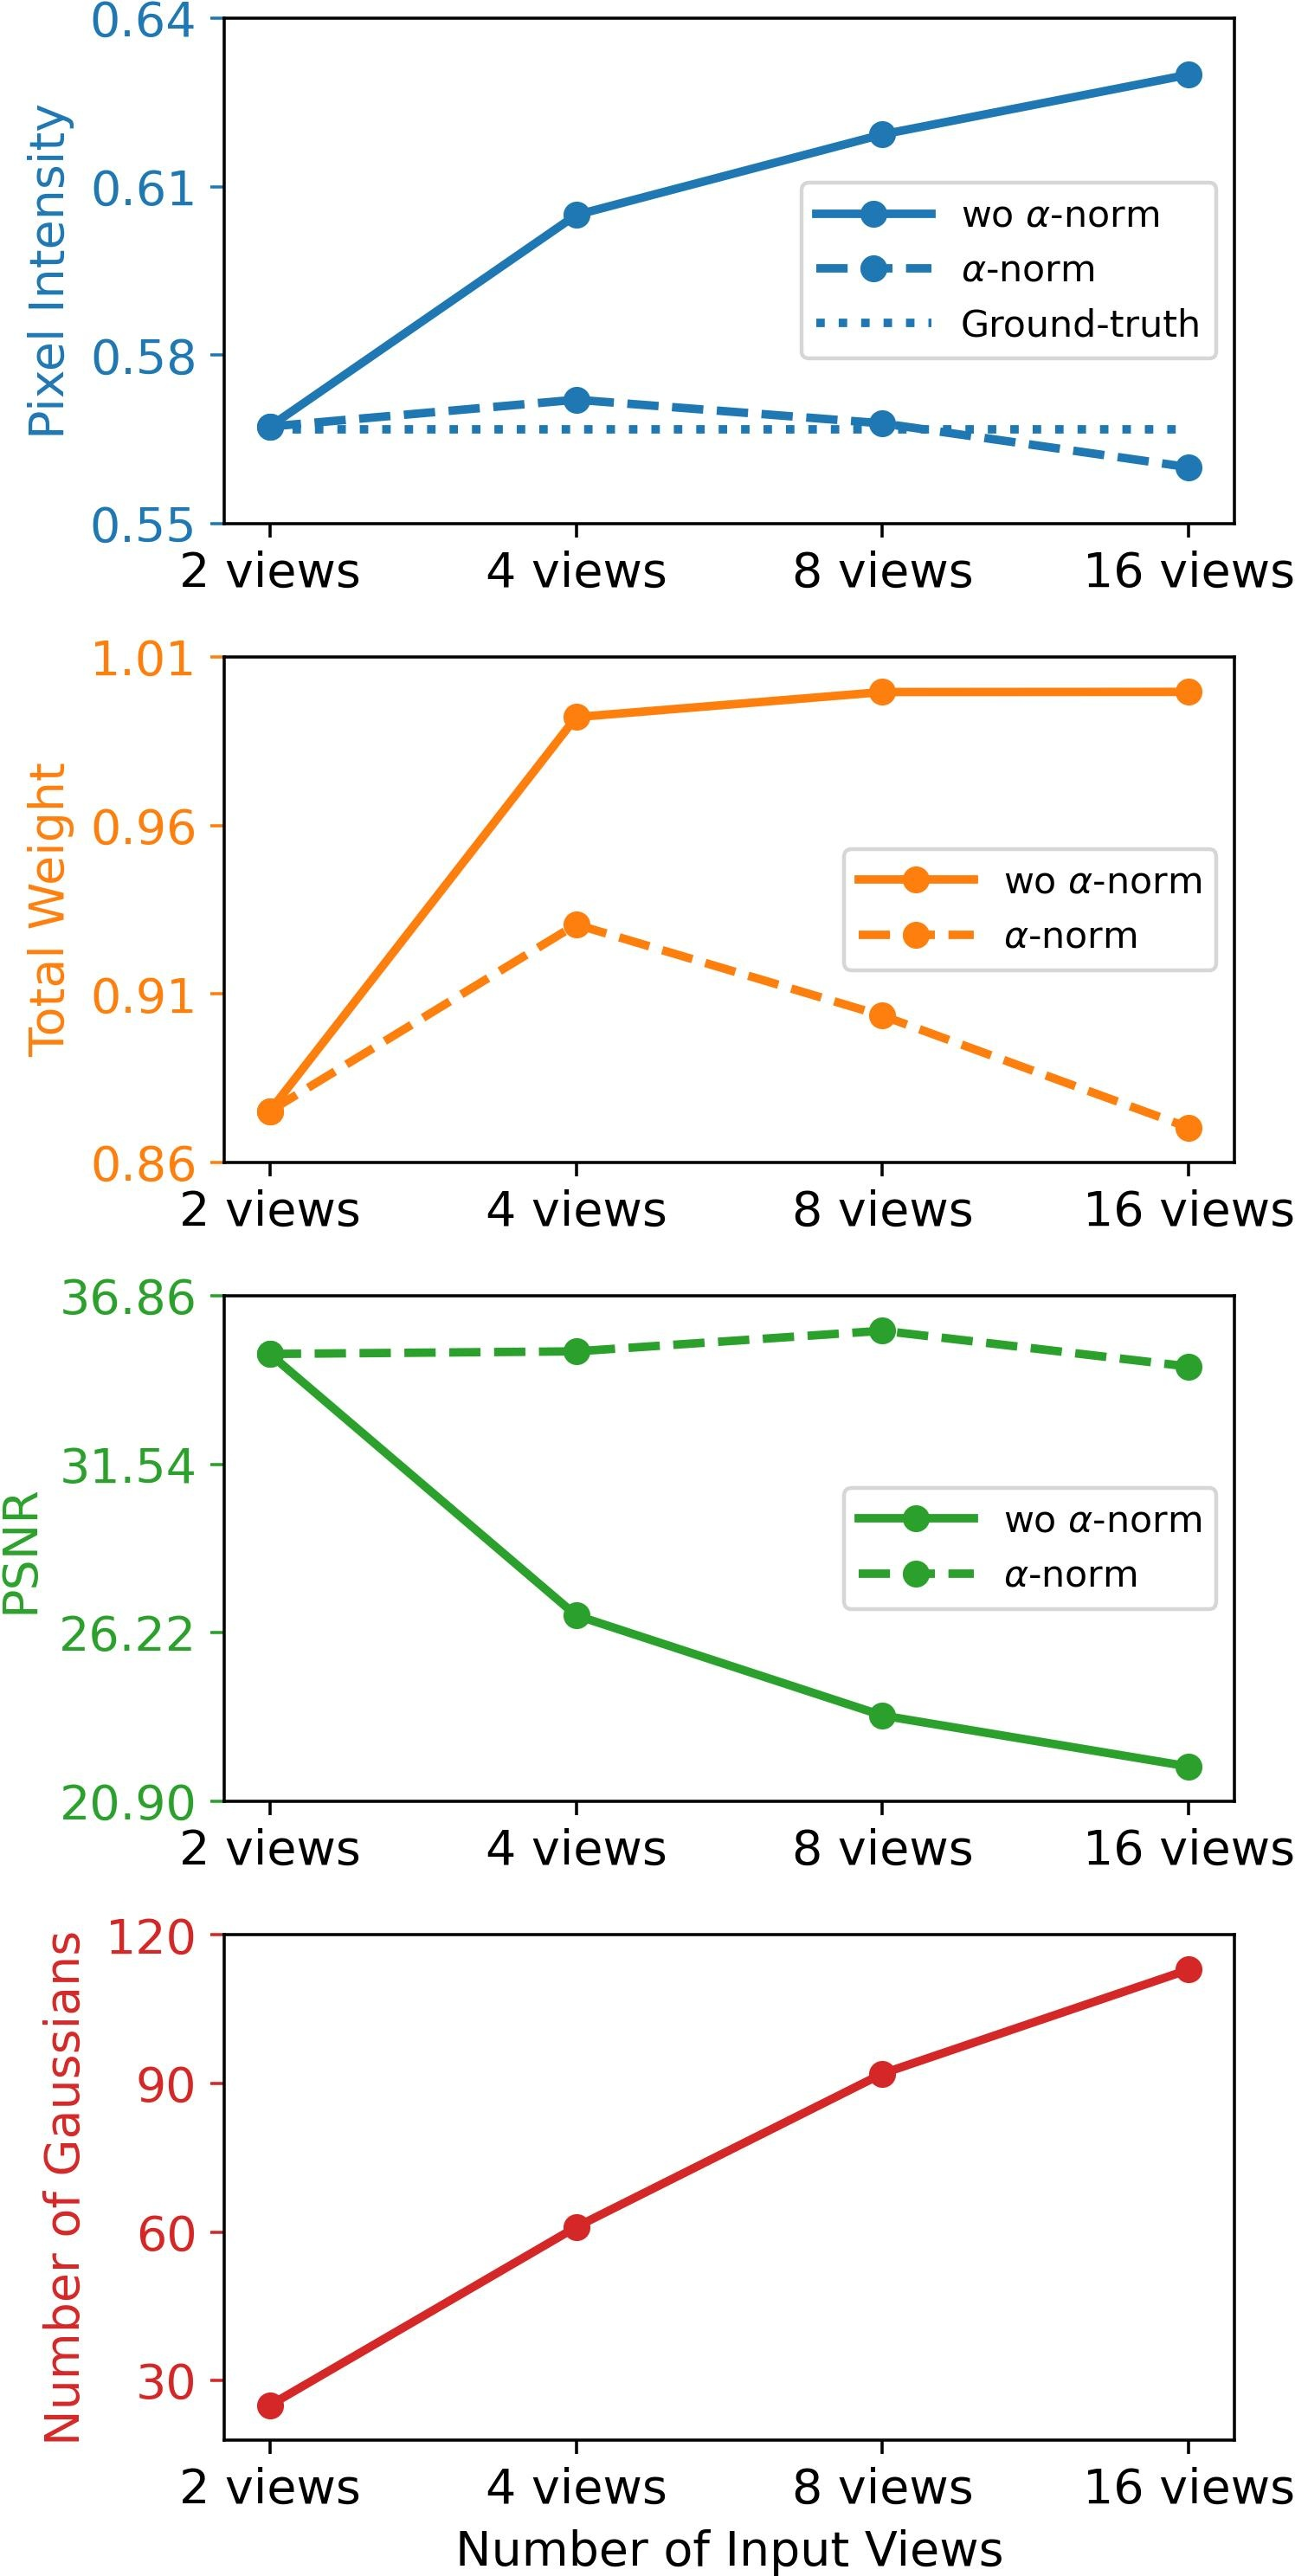} &
    \includegraphics[width=0.32\linewidth]{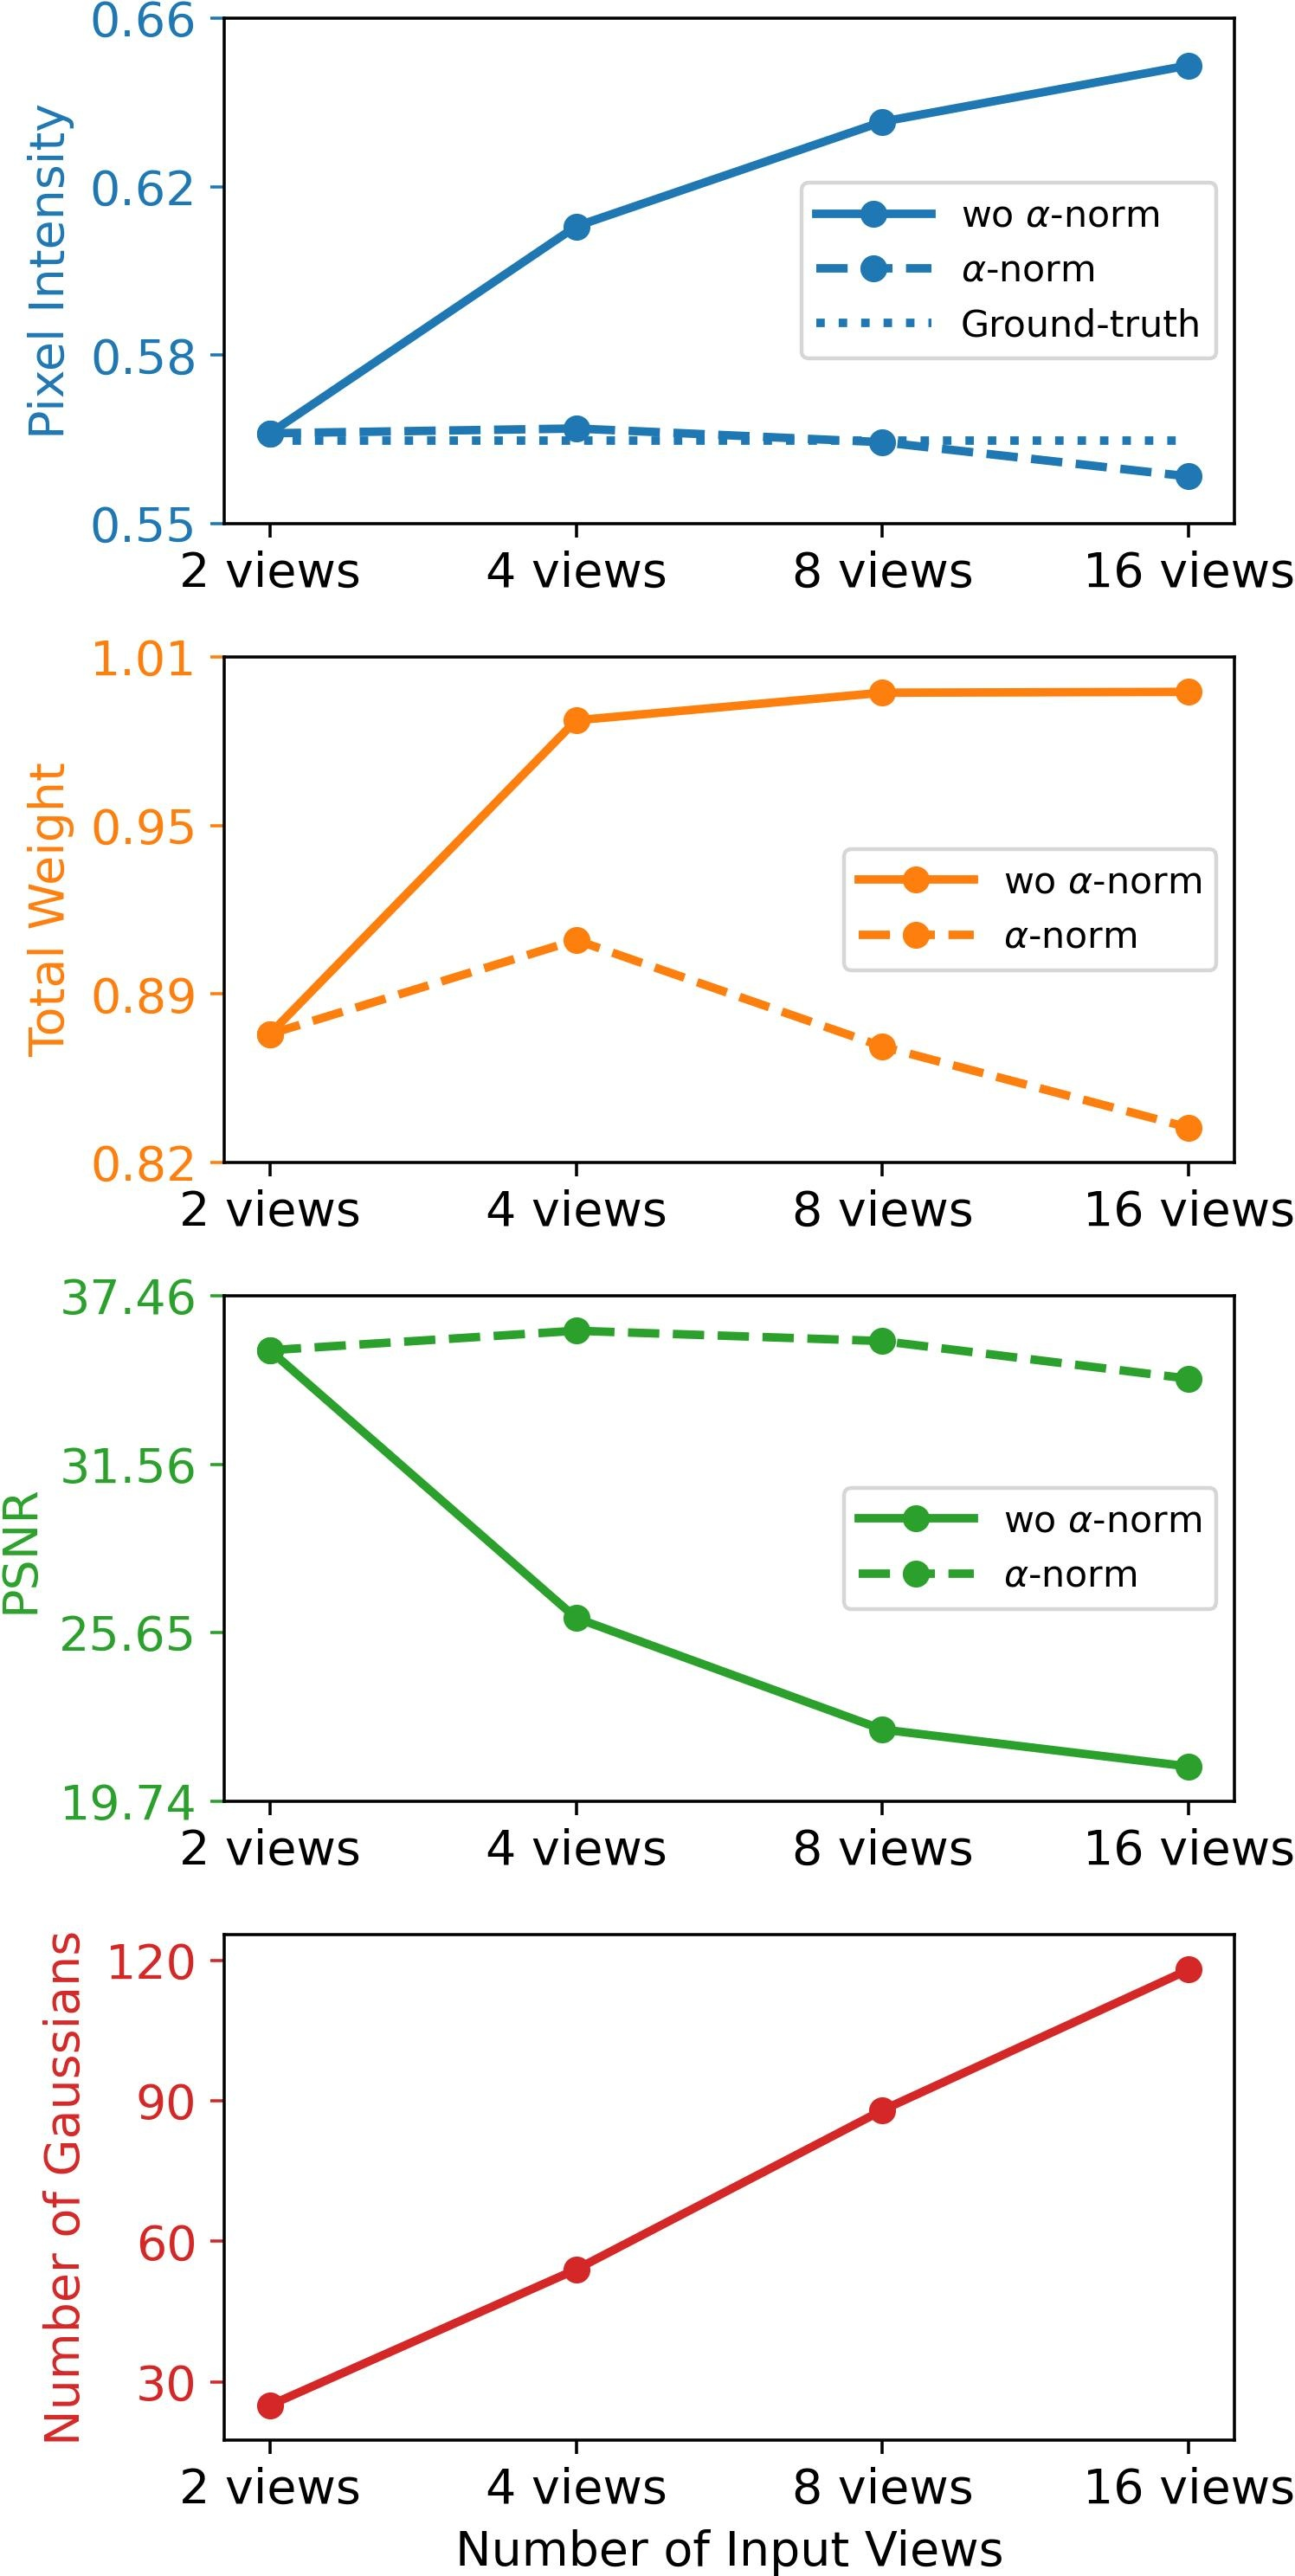} &
    \includegraphics[width=0.32\linewidth]{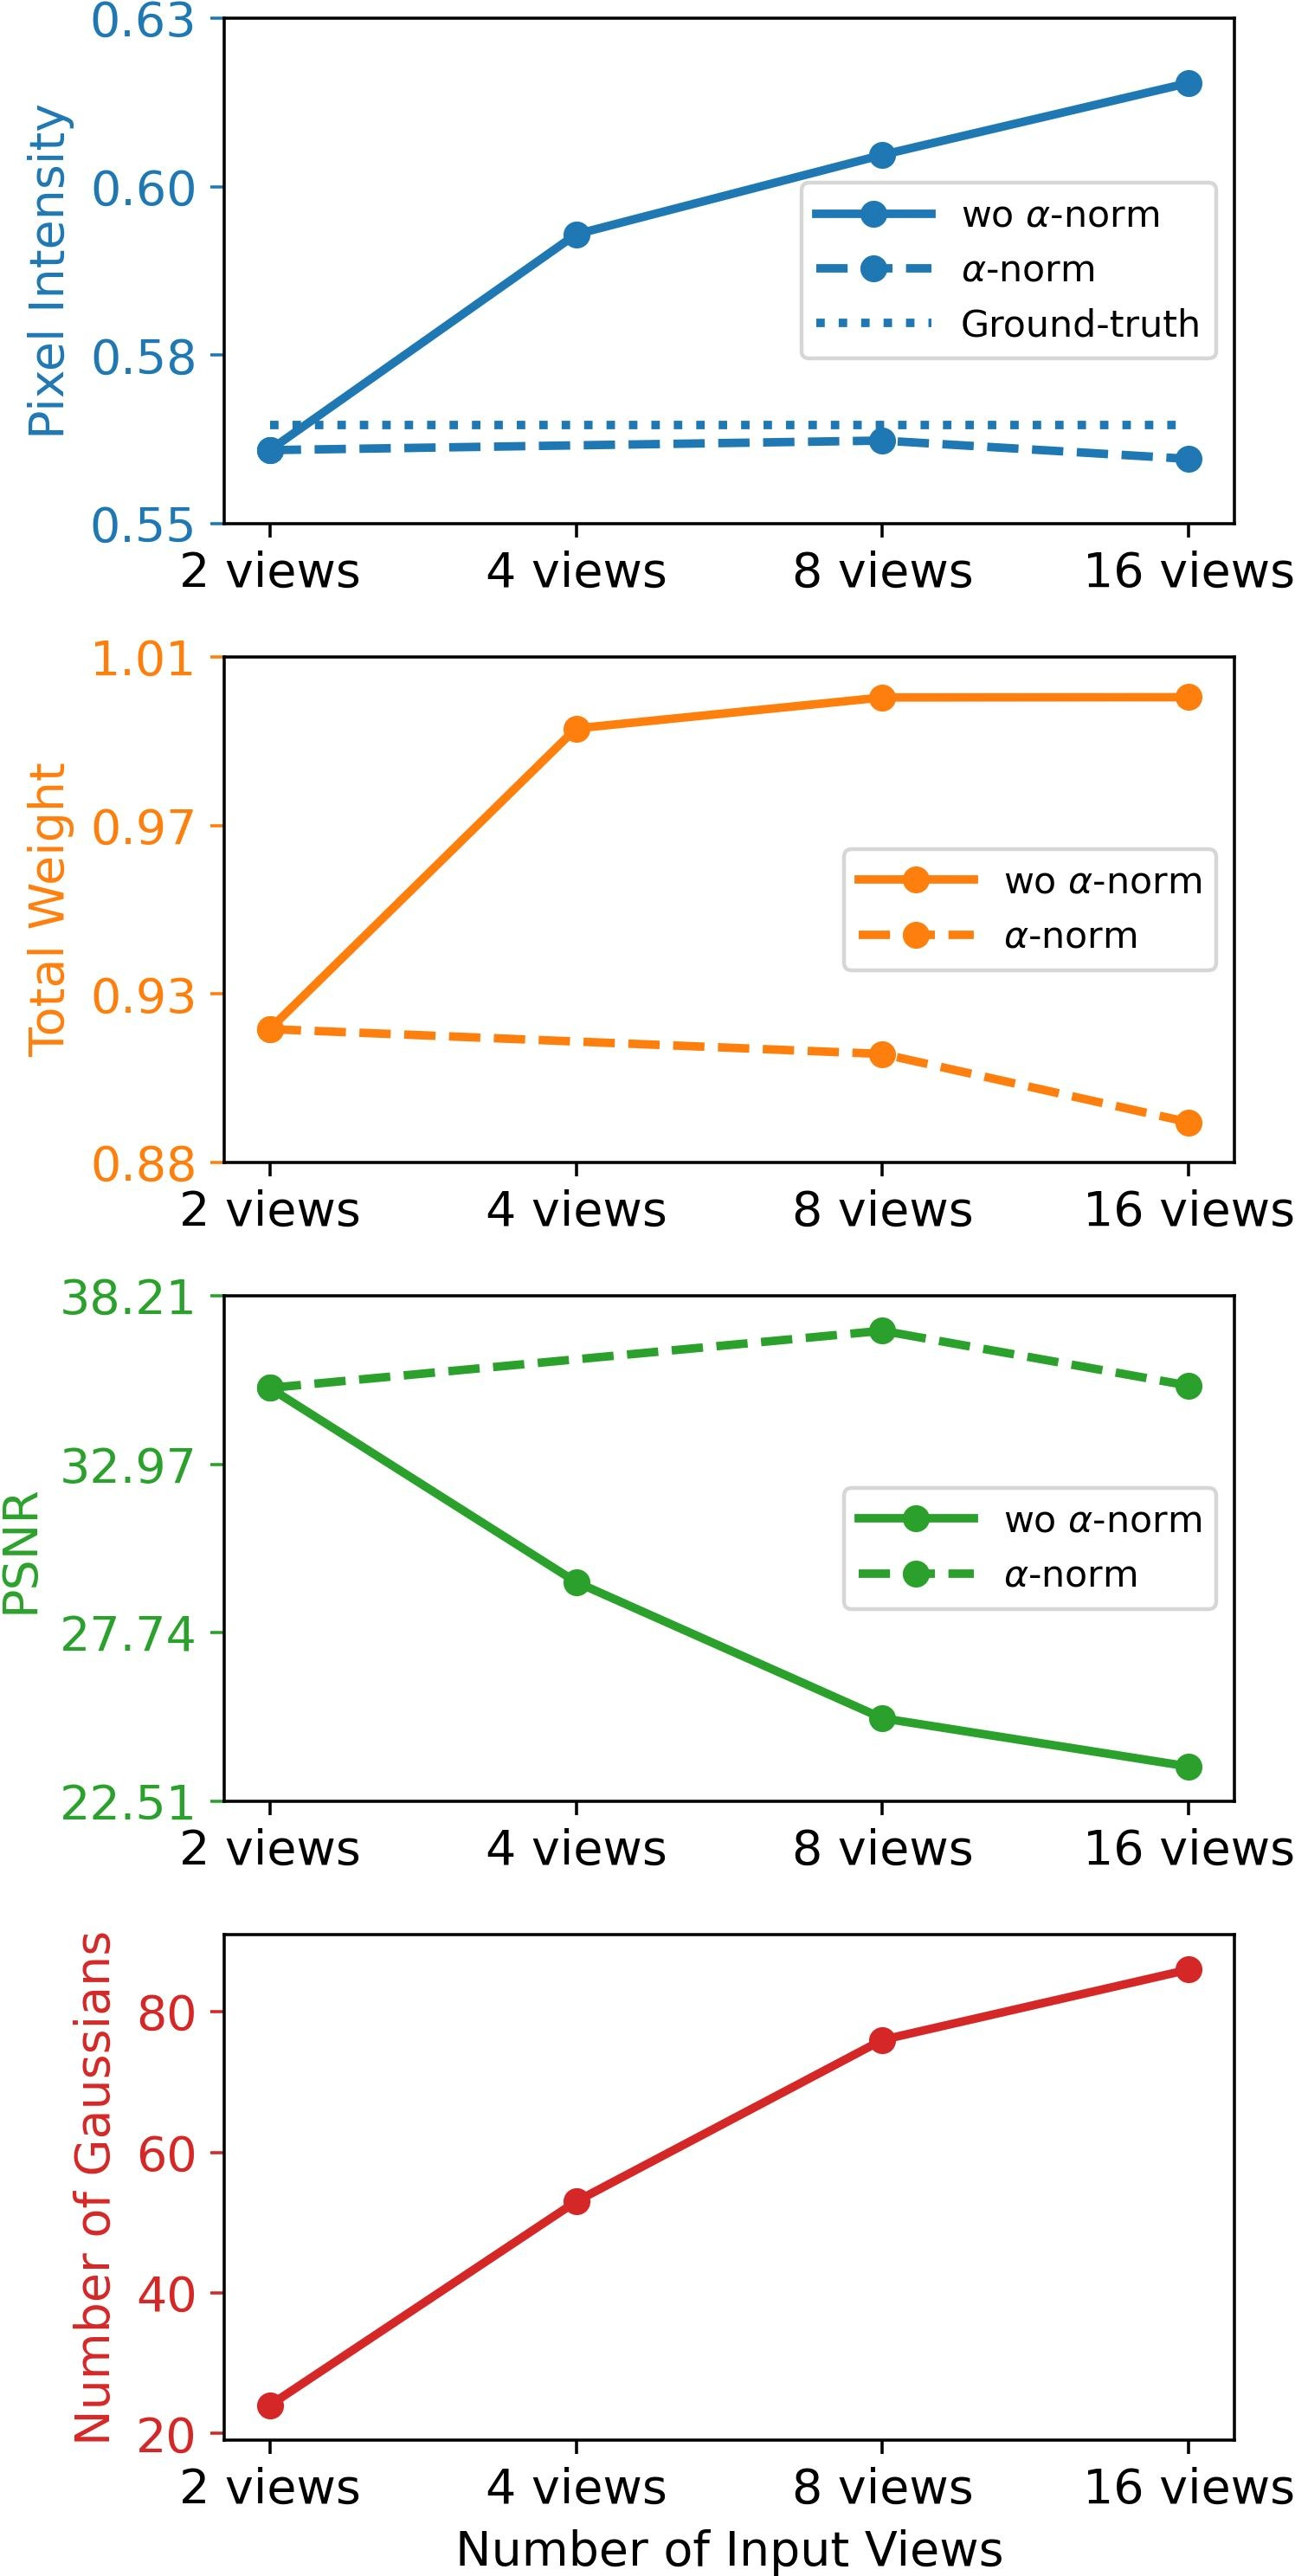} \\
    \end{tabular}
    
    \caption{Pixel intensity, accumulated compositing weight, image quality (PSNR), and number of predicted Gaussians under varying input-view counts. \textbf{First row}: Median gray-scale pixel intensity across the whole image. \textbf{Second row}: Median total accumulated weight across the whole image. \textbf{Third row}: Image quality measured via PSNR. \textbf{Last row}: Median number of Gaussians used for rendering. To compute this, we first obtain the number of Gaussians involve in the rendering process for each pixel, then compute the median value across all pixels. \textbf{Analysis}: Increasing the number of input views causes existing feed-forward Gaussian Splatting methods~\cite{chen2024mvsplat, zhang2025transplat, xu2025depthsplat} to predict more overlapping Gaussians (last row), which increases the accumulated compositing weight $W$ (second row), raises pixel intensity (first row), leading to overbright images and PSNR degradation (third row). Our alpha normalization mitigates this effect by stabilizing $W$, leading to more consistent brightness and improved rendering quality.}
    \label{fig:alpha_norm_curve}
\end{figure}

\section{Sensitivity to Depth Error Threshold}

\begin{figure}[t]
    \centering
    \includegraphics[width=\textwidth]{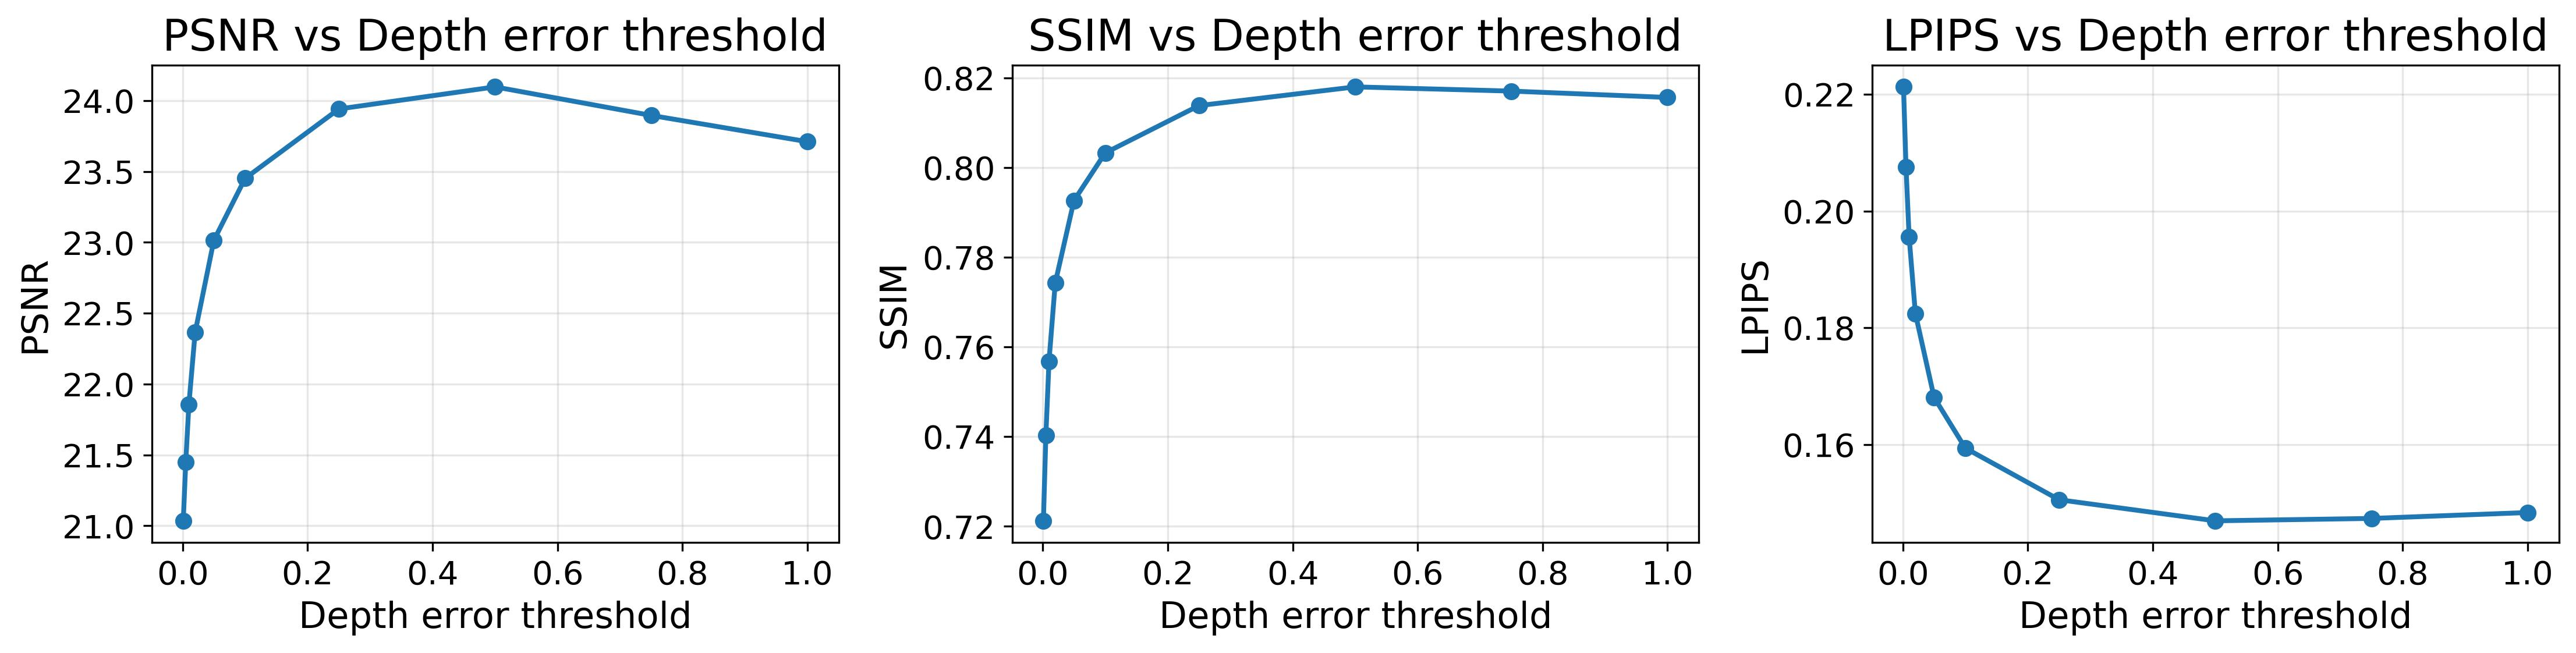}
    \caption{\textbf{Sensitivity to depth error threshold}. Using a threshold of 0.5 results in the best image quality across all metrics.}
    \label{fig:depth_sensitivity}
\end{figure}

Fig~\ref{fig:depth_sensitivity} show the performance of our method with different depth error thresholds. The plot reveals that setting the threshold to 0.5 shows the best performance across all metrics. On the other hand, threshold higher than 0.5 lead to minor drop in the image quality, while thresholds below 0.5 result in higher degradation.
