# Supplementary material for: RoSplat: Robust Feed-Forward Pixel-wise Gaussian Splatting for Varying Input Views and High-Resolution Rendering
Source: arXiv:2605.13093 source file (2026-05-13)
Supplement: Supplementary file 2 [file more_qualitative_result_alpha_norm.tex]

\section{More Qualitative Results}
Fig.~\ref{fig:gaussian_visualization} visualizes the Gaussians predicted by our method and DepthSplat. It shows that our method produces Gaussians with larger scales, leading to better coverage of the 3D scene. In contrast, DepthSplat~\cite{xu2025depthsplat} tends to predict overly small-scale Gaussians, which results in hole artifacts.

In Figs.~\ref{fig:qualitative_result_alpha_norm_1} and \ref{fig:qualitative_result_alpha_norm_2}, we provide additional qualitative comparisons to show the effect of applying alpha normalization to existing methods~\cite{chen2024mvsplat, zhang2025transplat, xu2025depthsplat}. Moreover, Fig.~\ref{fig:qualitative_result_high_resolution} presents further visual comparisons between our method and DepthSplat~\cite{xu2025depthsplat} for high-resolution rendering. The results show that our method mitigates the over-brightness and hole artifacts exhibited by existing methods.

\begin{figure}
    \centering
    \includegraphics[width=0.78\textwidth]{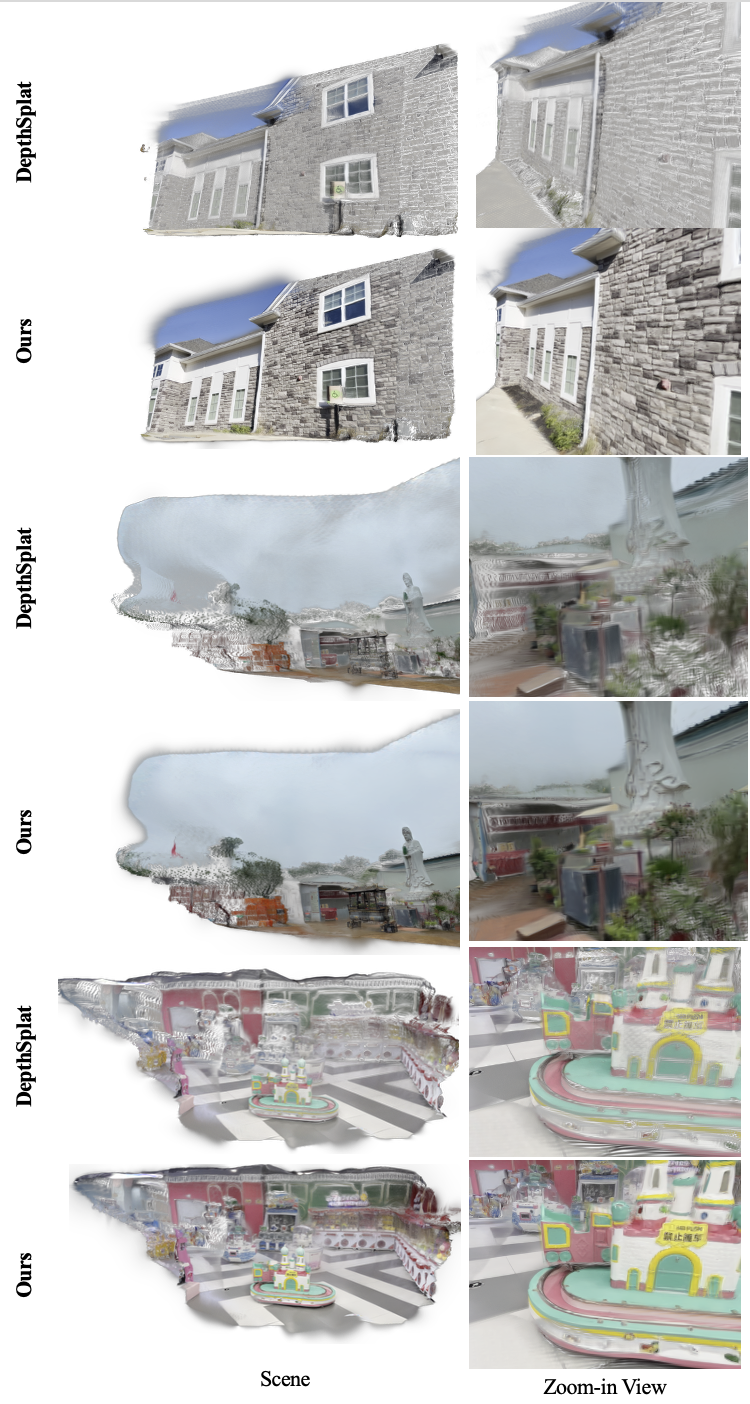}
    \caption{\textbf{Gaussians visualizations on the DL3DV dataset}. We can see that scenes reconstructed by DepthSplat~\cite{xu2025depthsplat} show many hole artifacts in zoom-in views, while ours shows few or even no hole artifacts (white cracked areas in above figures).}
    \label{fig:gaussian_visualization}
\end{figure}

\begin{figure}
\centering
\footnotesize

\begin{tblr}[]{
  width = 0.95\linewidth,
  colsep = 1pt,
  rowsep = 0.0pt, % Set explicitly to 0pt
  stretch = 0.25,  % Turns off default line stretching
  row{2-Z} = {abovesep=0pt, belowsep=0pt}, % Kills inner cell padding for all image rows
  colspec = {Q[wd=4mm,c,m] X[c,m] X[c,m] X[c,m] X[c,m]},
  row{1} = {abovesep=2pt, belowsep=2pt}, % Keeps a normal gap for your text header
  cell{1-Z}{1} = {halign=c, valign=m}, 
  % hline{5} = {dashed, abovesep=0pt, belowsep=0pt},
}

 & 2 views & 4 views & 8 views & 16 views \\

% \smash{\rotatebox[origin=c]{90}{2 views}} &  
% \includegraphics[width=\linewidth]{supps/Figures/alpha_norm_vis/mvsplat_rendered_2views_TrueAlpha.png} &
% \includegraphics[width=\linewidth]{supps/Figures/alpha_norm_vis/depthsplat_rendered_2views_TrueAlpha.png} &
% \includegraphics[width=\linewidth]{supps/Figures/alpha_norm_vis/transplat_rendered_2views_TrueAlpha.png} &
% \includegraphics[width=\linewidth]{supps/Figures/alpha_norm_vis/gt.png} \\

\raisebox{35pt}{\smash{\rotatebox[origin=c]{90}{Ground-truth}}} &  
\includegraphics[width=\linewidth]{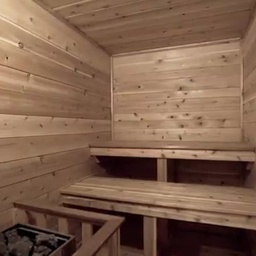} &
\includegraphics[width=\linewidth]{supps/Figures/alpha_norm_vis/09b505bb829c1d12/gt.jpg} &
\includegraphics[width=\linewidth]{supps/Figures/alpha_norm_vis/09b505bb829c1d12/gt.jpg} &
\includegraphics[width=\linewidth]{supps/Figures/alpha_norm_vis/09b505bb829c1d12/gt.jpg} \\

% --- REMOVED BLANK LINES HERE ---
\raisebox{35pt}{\smash{\rotatebox[origin=c]{90}{DepthSplat~\cite{xu2025depthsplat}}}} &
\includegraphics[width=\linewidth]{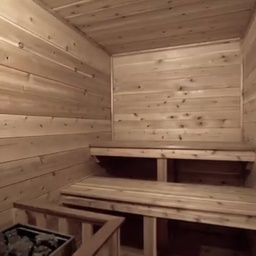} &
\includegraphics[width=\linewidth]{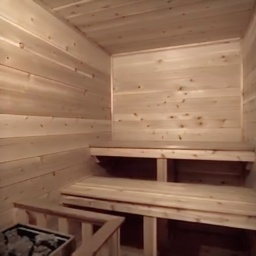} &
\includegraphics[width=\linewidth]{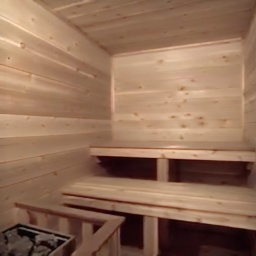} & 
\includegraphics[width=\linewidth]
{supps/Figures/alpha_norm_vis/09b505bb829c1d12/depthsplat_rendered_16views_FalseAlpha.jpg} \\

% --- REMOVED BLANK LINES HERE ---
\SetRow{abovesep=2pt}
\raisebox{35pt}{\smash{\rotatebox[origin=c]{90}{\cite{xu2025depthsplat} + $\alpha$ norm.}}} &
\includegraphics[width=\linewidth]{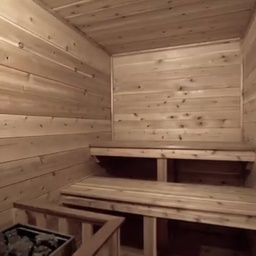} &
\includegraphics[width=\linewidth]{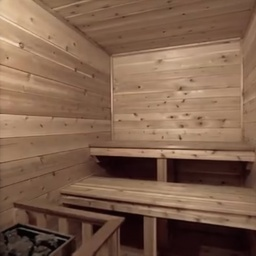} &
\includegraphics[width=\linewidth]{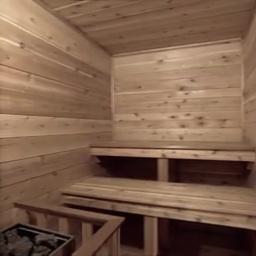} & 
\includegraphics[width=\linewidth]
{supps/Figures/alpha_norm_vis/09b505bb829c1d12/depthsplat_rendered_16views_TrueAlpha.jpg} \\

\hline[dashed, wd=0.5pt] 
\SetRow{belowsep=4pt}

\raisebox{35pt}{\smash{\rotatebox[origin=c]{90}{Ground-truth}}} &  
\includegraphics[width=\linewidth]{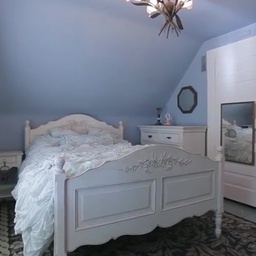} &
\includegraphics[width=\linewidth]{supps/Figures/alpha_norm_vis/308de3d523189c72/gt.jpg} &
\includegraphics[width=\linewidth]{supps/Figures/alpha_norm_vis/308de3d523189c72/gt.jpg} &
\includegraphics[width=\linewidth]{supps/Figures/alpha_norm_vis/308de3d523189c72/gt.jpg} \\

% --- REMOVED BLANK LINES HERE ---
\raisebox{35pt}{\smash{\rotatebox[origin=c]{90}{TranSplat~\cite{zhang2025transplat}}}} &
\includegraphics[width=\linewidth]{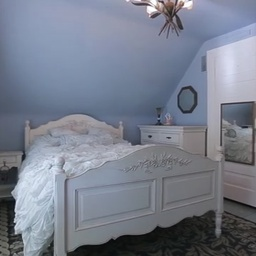} &
\includegraphics[width=\linewidth]{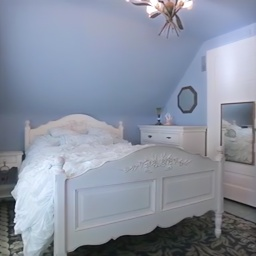} &
\includegraphics[width=\linewidth]{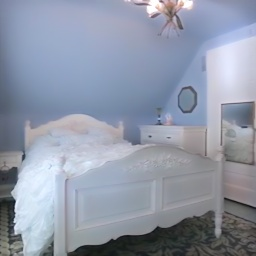} & 
\includegraphics[width=\linewidth]
{supps/Figures/alpha_norm_vis/308de3d523189c72/transplat_rendered_16views_FalseAlpha.jpg} \\

% --- REMOVED BLANK LINES HERE ---
\raisebox{35pt}{\smash{\rotatebox[origin=c]{90}{\cite{zhang2025transplat} + $\alpha$ norm.}}} &
\includegraphics[width=\linewidth]{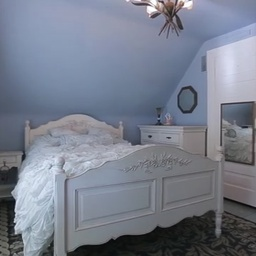} &
\includegraphics[width=\linewidth]{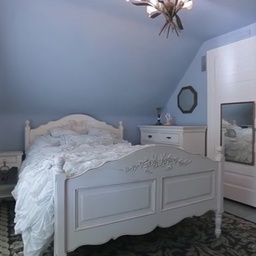} &
\includegraphics[width=\linewidth]{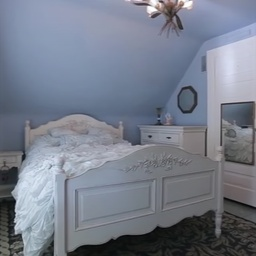} & 
\includegraphics[width=\linewidth]
{supps/Figures/alpha_norm_vis/308de3d523189c72/transplat_rendered_16views_TrueAlpha.jpg}

\end{tblr}
\caption{\textbf{Qualitative results on RealEstate10K dataset}. Here, we apply alpha normalization to existing works~\cite{zhang2025transplat, xu2025depthsplat} \textbf{without retraining}. Prior methods~\cite{zhang2025transplat, xu2025depthsplat} encounter overbrightness issue when the number of input views is greater than two. Integrating alpha normalization ($\alpha$ norm.)
helps to mitigate their overbrightness issues when increasing the number of input views. }
\label{fig:qualitative_result_alpha_norm_1}
\end{figure}

\begin{figure}
\centering
\footnotesize

\begin{tblr}[]{
  width = 0.95\linewidth,
  colsep = 1pt,
  rowsep = 0.0pt, % Set explicitly to 0pt
  stretch = 0.25,  % Turns off default line stretching
  row{2-Z} = {abovesep=0pt, belowsep=0pt}, % Kills inner cell padding for all image rows
  colspec = {Q[wd=4mm,c,m] X[c,m] X[c,m] X[c,m] X[c,m]},
  row{1} = {abovesep=2pt, belowsep=2pt}, % Keeps a normal gap for your text header
  cell{1-Z}{1} = {halign=c, valign=m}, 
  % hline{5} = {dashed, abovesep=0pt, belowsep=0pt},
}

 & 2 views & 4 views & 8 views & 16 views \\

% \smash{\rotatebox[origin=c]{90}{2 views}} &  
% \includegraphics[width=\linewidth]{supps/Figures/alpha_norm_vis/mvsplat_rendered_2views_TrueAlpha.png} &
% \includegraphics[width=\linewidth]{supps/Figures/alpha_norm_vis/depthsplat_rendered_2views_TrueAlpha.png} &
% \includegraphics[width=\linewidth]{supps/Figures/alpha_norm_vis/transplat_rendered_2views_TrueAlpha.png} &
% \includegraphics[width=\linewidth]{supps/Figures/alpha_norm_vis/gt.png} \\

\raisebox{35pt}{\smash{\rotatebox[origin=c]{90}{Ground-truth}}} &  
\includegraphics[width=\linewidth]{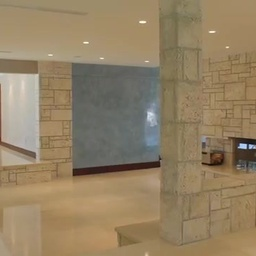} &
\includegraphics[width=\linewidth]{supps/Figures/alpha_norm_vis/28742766eb882cd2/gt.jpg} &
\includegraphics[width=\linewidth]{supps/Figures/alpha_norm_vis/28742766eb882cd2/gt.jpg} &
\includegraphics[width=\linewidth]{supps/Figures/alpha_norm_vis/28742766eb882cd2/gt.jpg} \\

% --- REMOVED BLANK LINES HERE ---
\raisebox{35pt}{\smash{\rotatebox[origin=c]{90}{MVSplat~\cite{chen2024mvsplat}}}} &
\includegraphics[width=\linewidth]{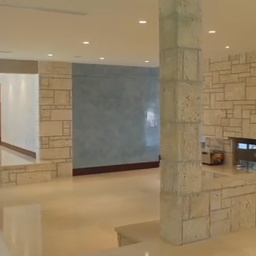} &
\includegraphics[width=\linewidth]{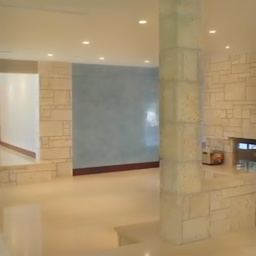} &
\includegraphics[width=\linewidth]{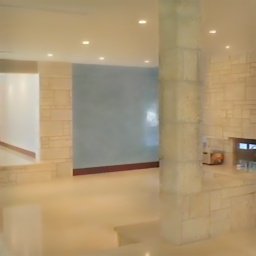} & 
\includegraphics[width=\linewidth]
{supps/Figures/alpha_norm_vis/28742766eb882cd2/mvsplat_rendered_16views_FalseAlpha.jpg} \\

% --- REMOVED BLANK LINES HERE ---
\SetRow{abovesep=2pt}
\raisebox{35pt}{\smash{\rotatebox[origin=c]{90}{\cite{chen2024mvsplat} + $\alpha$ norm.}}} &
\includegraphics[width=\linewidth]{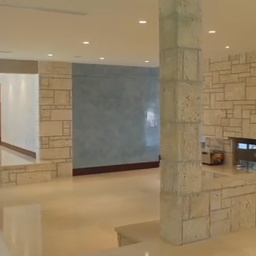} &
\includegraphics[width=\linewidth]{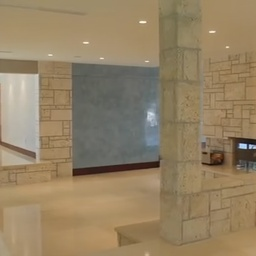} &
\includegraphics[width=\linewidth]{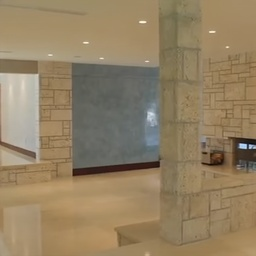} & 
\includegraphics[width=\linewidth]
{supps/Figures/alpha_norm_vis/28742766eb882cd2/mvsplat_rendered_16views_TrueAlpha.jpg} \\

\hline[dashed, wd=0.5pt] 
\SetRow{belowsep=4pt}

\raisebox{35pt}{\smash{\rotatebox[origin=c]{90}{Ground-truth}}} &  
\includegraphics[width=\linewidth]{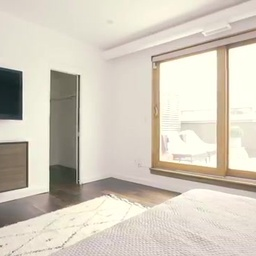} &
\includegraphics[width=\linewidth]{supps/Figures/alpha_norm_vis/e07392b123f6fd77/gt.jpg} &
\includegraphics[width=\linewidth]{supps/Figures/alpha_norm_vis/e07392b123f6fd77/gt.jpg} &
\includegraphics[width=\linewidth]{supps/Figures/alpha_norm_vis/e07392b123f6fd77/gt.jpg} \\

% --- REMOVED BLANK LINES HERE ---
\raisebox{35pt}{\smash{\rotatebox[origin=c]{90}{TranSplat~\cite{zhang2025transplat}}}} &
\includegraphics[width=\linewidth]{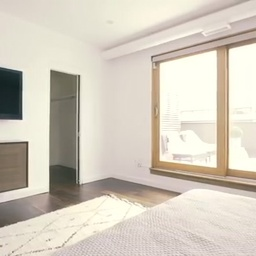} &
\includegraphics[width=\linewidth]{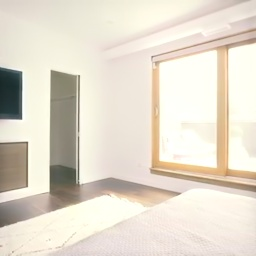} &
\includegraphics[width=\linewidth]{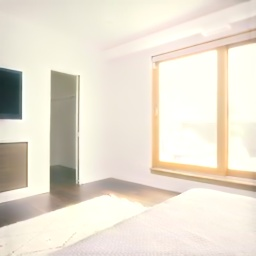} & 
\includegraphics[width=\linewidth]
{supps/Figures/alpha_norm_vis/e07392b123f6fd77/transplat_rendered_16views_FalseAlpha.jpg} \\

% --- REMOVED BLANK LINES HERE ---
\raisebox{35pt}{\smash{\rotatebox[origin=c]{90}{\cite{zhang2025transplat} + $\alpha$ norm.}}} &
\includegraphics[width=\linewidth]{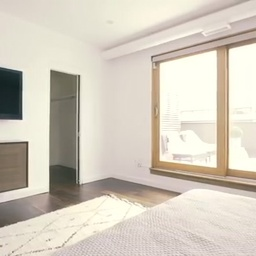} &
\includegraphics[width=\linewidth]{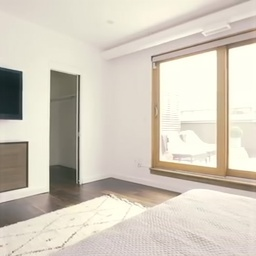} &
\includegraphics[width=\linewidth]{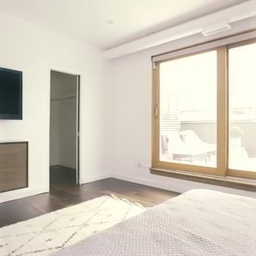} & 
\includegraphics[width=\linewidth]
{supps/Figures/alpha_norm_vis/e07392b123f6fd77/transplat_rendered_16views_TrueAlpha.jpg}

\end{tblr}
\caption{\textbf{Qualitative results on RealEstate10K dataset}. Here, we apply alpha normalization to existing works~\cite{zhang2025transplat, chen2024mvsplat} \textbf{without retraining}. Prior methods~\cite{zhang2025transplat, chen2024mvsplat} encounter overbrightness issue when the number of input views is greater than two. Integrating alpha normalization ($\alpha$ norm.)
helps to mitigate their overbrightness issues when increasing the number of input views. }
\label{fig:qualitative_result_alpha_norm_2}
\end{figure}

\begin{figure}
    \centering
    % Set to 0pt if you want absolutely no gap between the images
    \setlength{\tabcolsep}{1pt} 
    
    \begin{tabular}{ccc}
        % --- Header Row ---
        Ground-truth & DepthSplat~\cite{xu2025depthsplat} & Ours \\

        % --- Row 1 Images ---
        \includegraphics[width=0.32\linewidth]{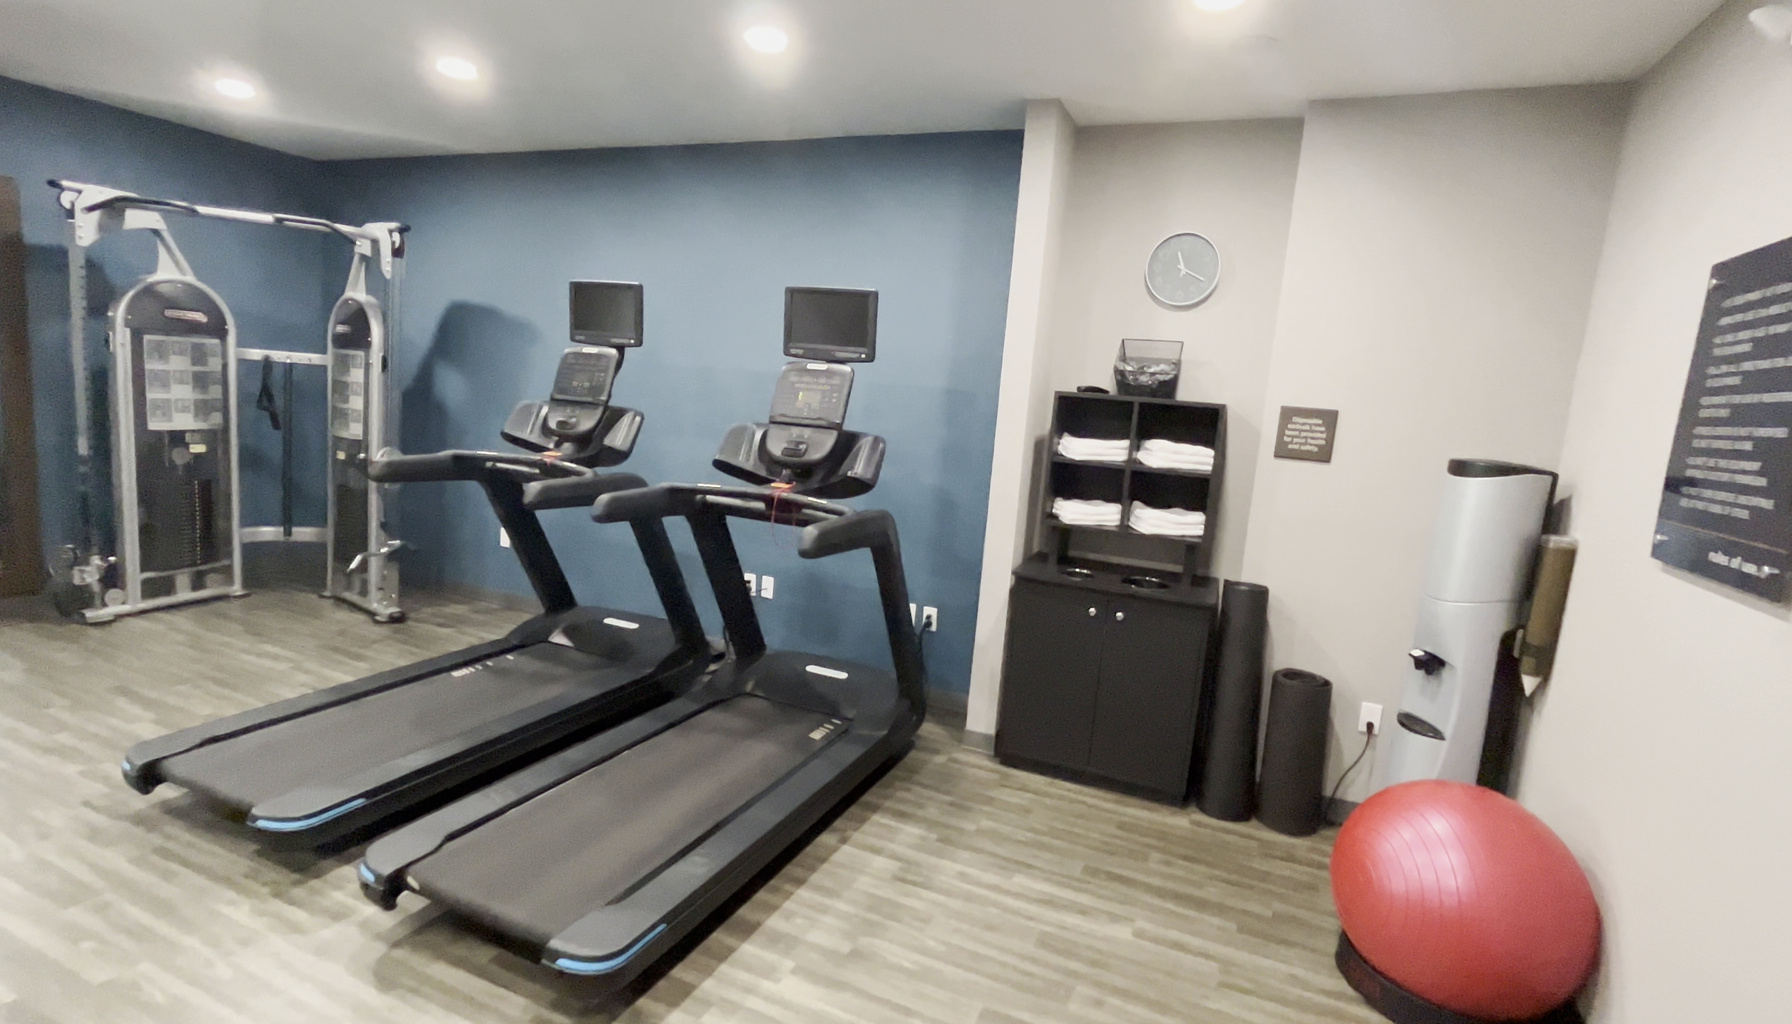} & 
        \includegraphics[width=0.32\linewidth]{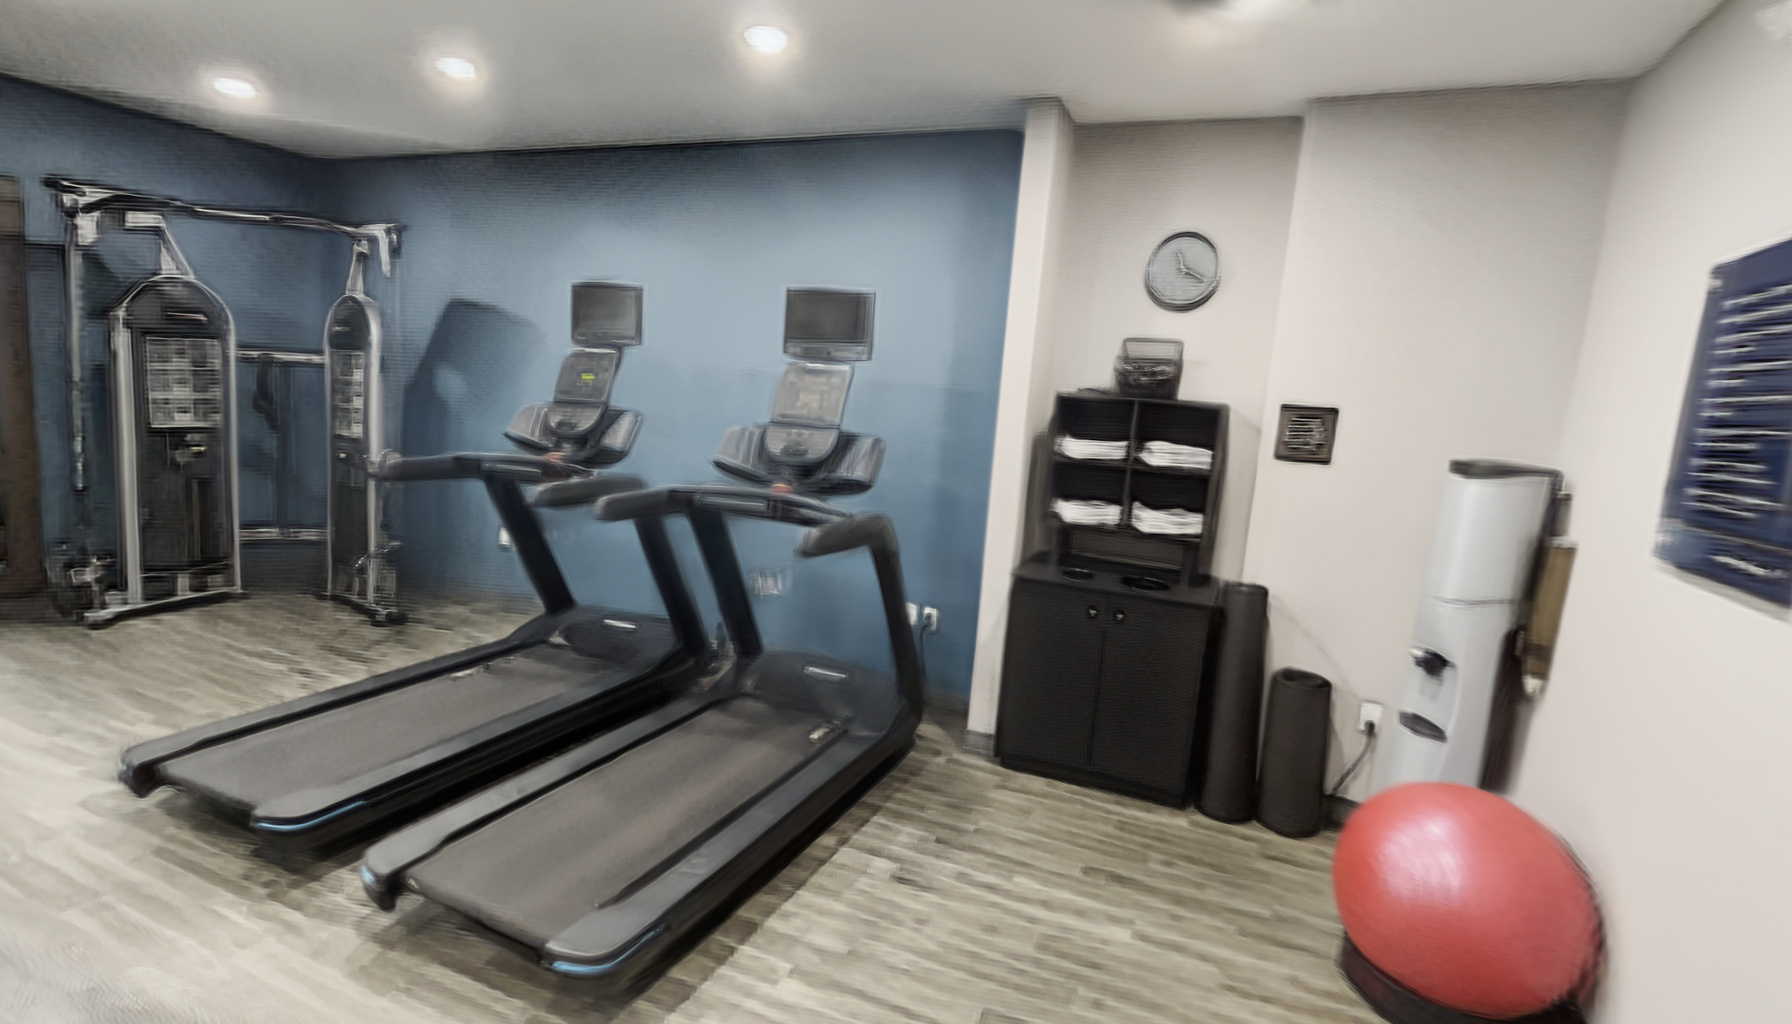} & 
        \includegraphics[width=0.32\linewidth]{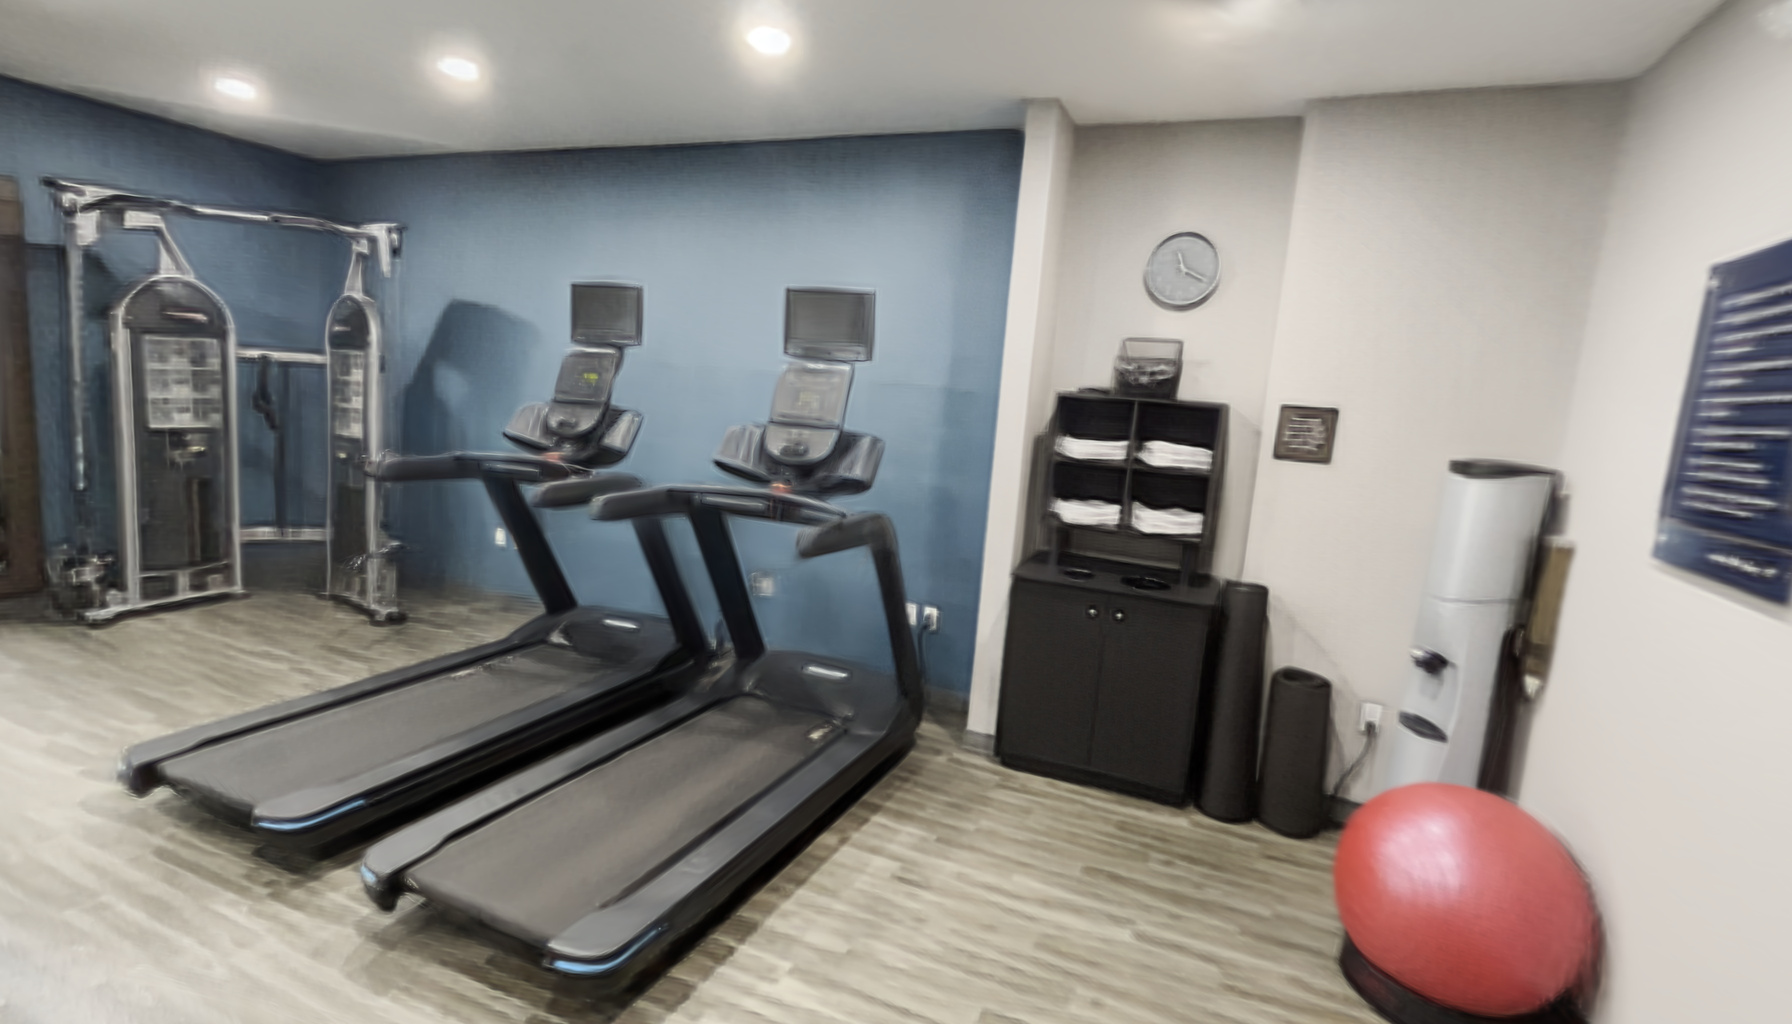} \\

        \includegraphics[width=0.32\linewidth]{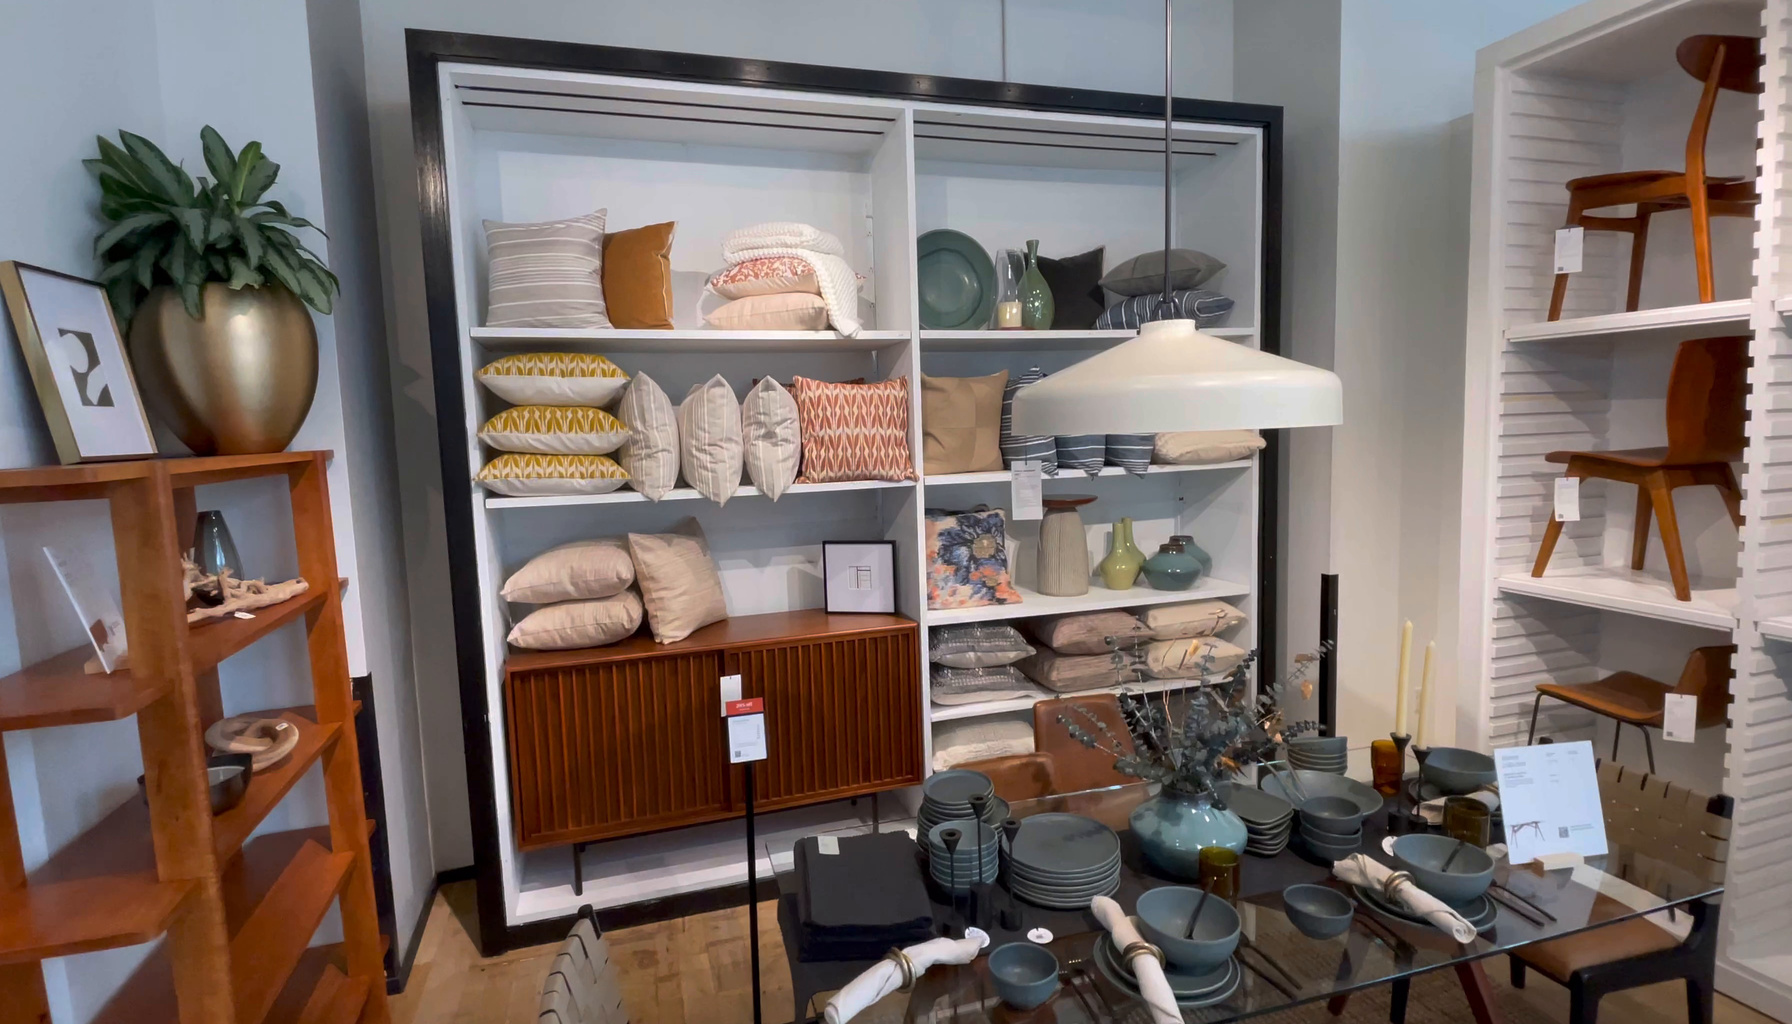} & 
        \includegraphics[width=0.32\linewidth]{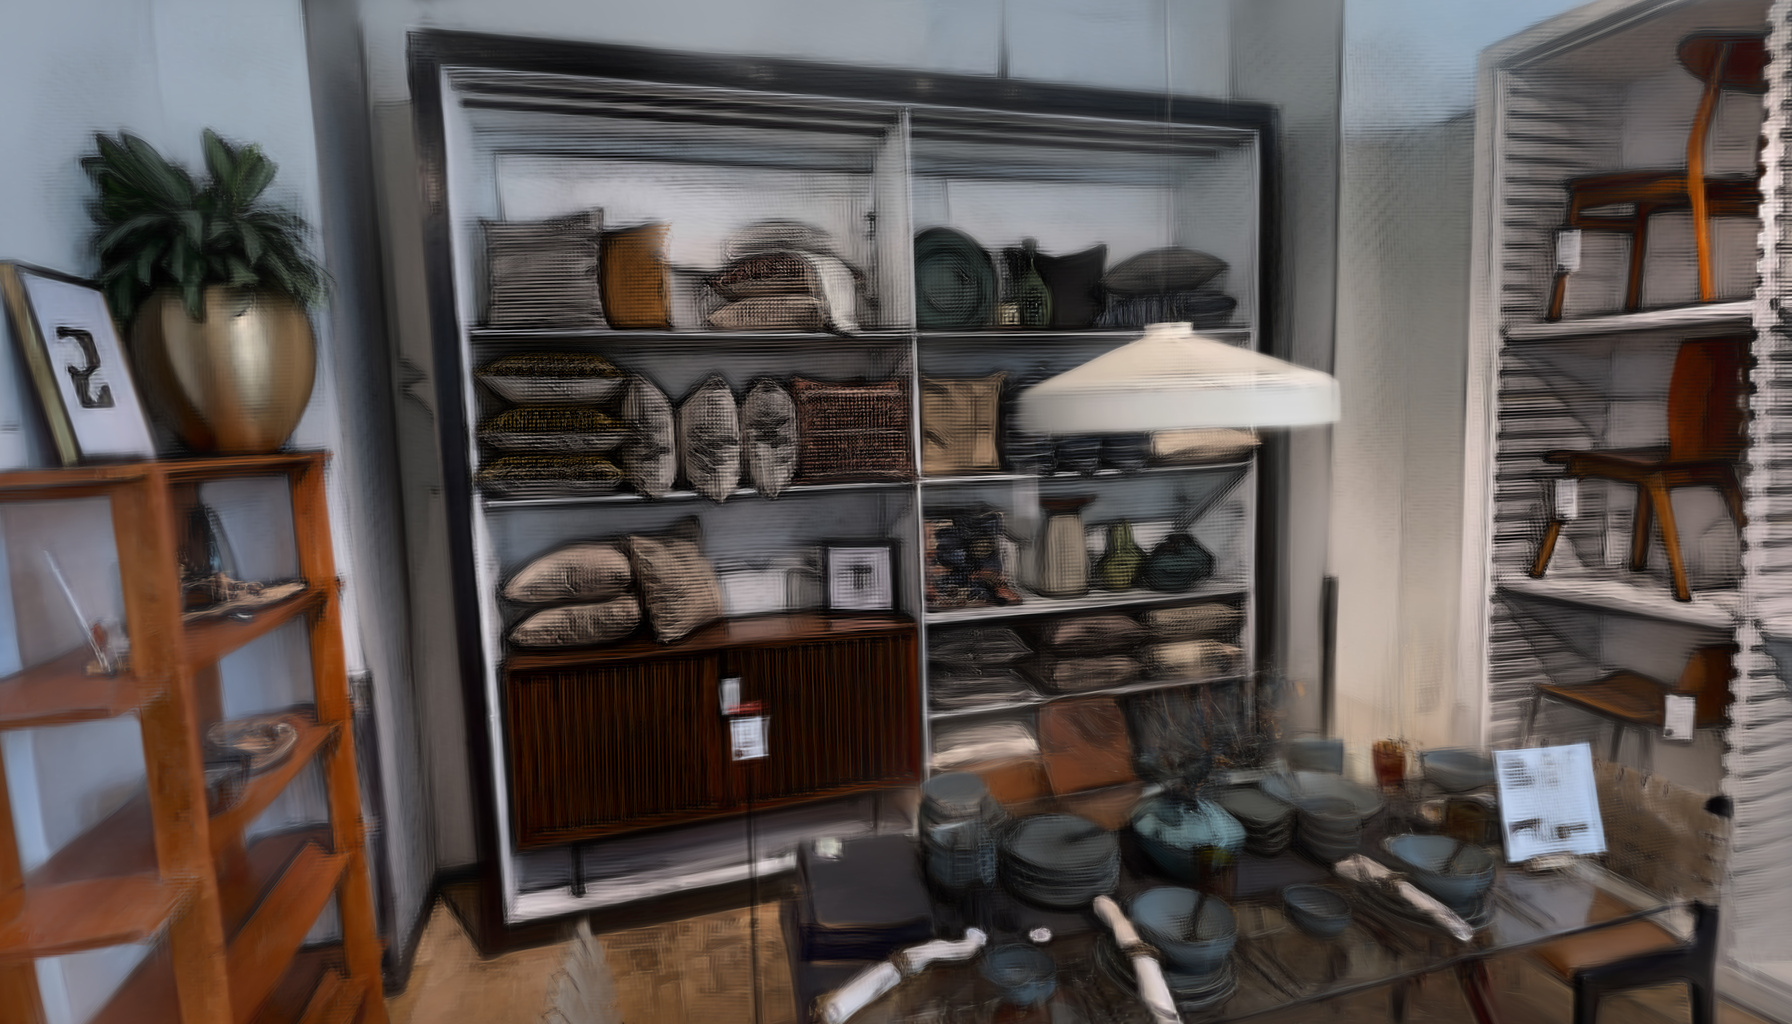} & 
        \includegraphics[width=0.32\linewidth]{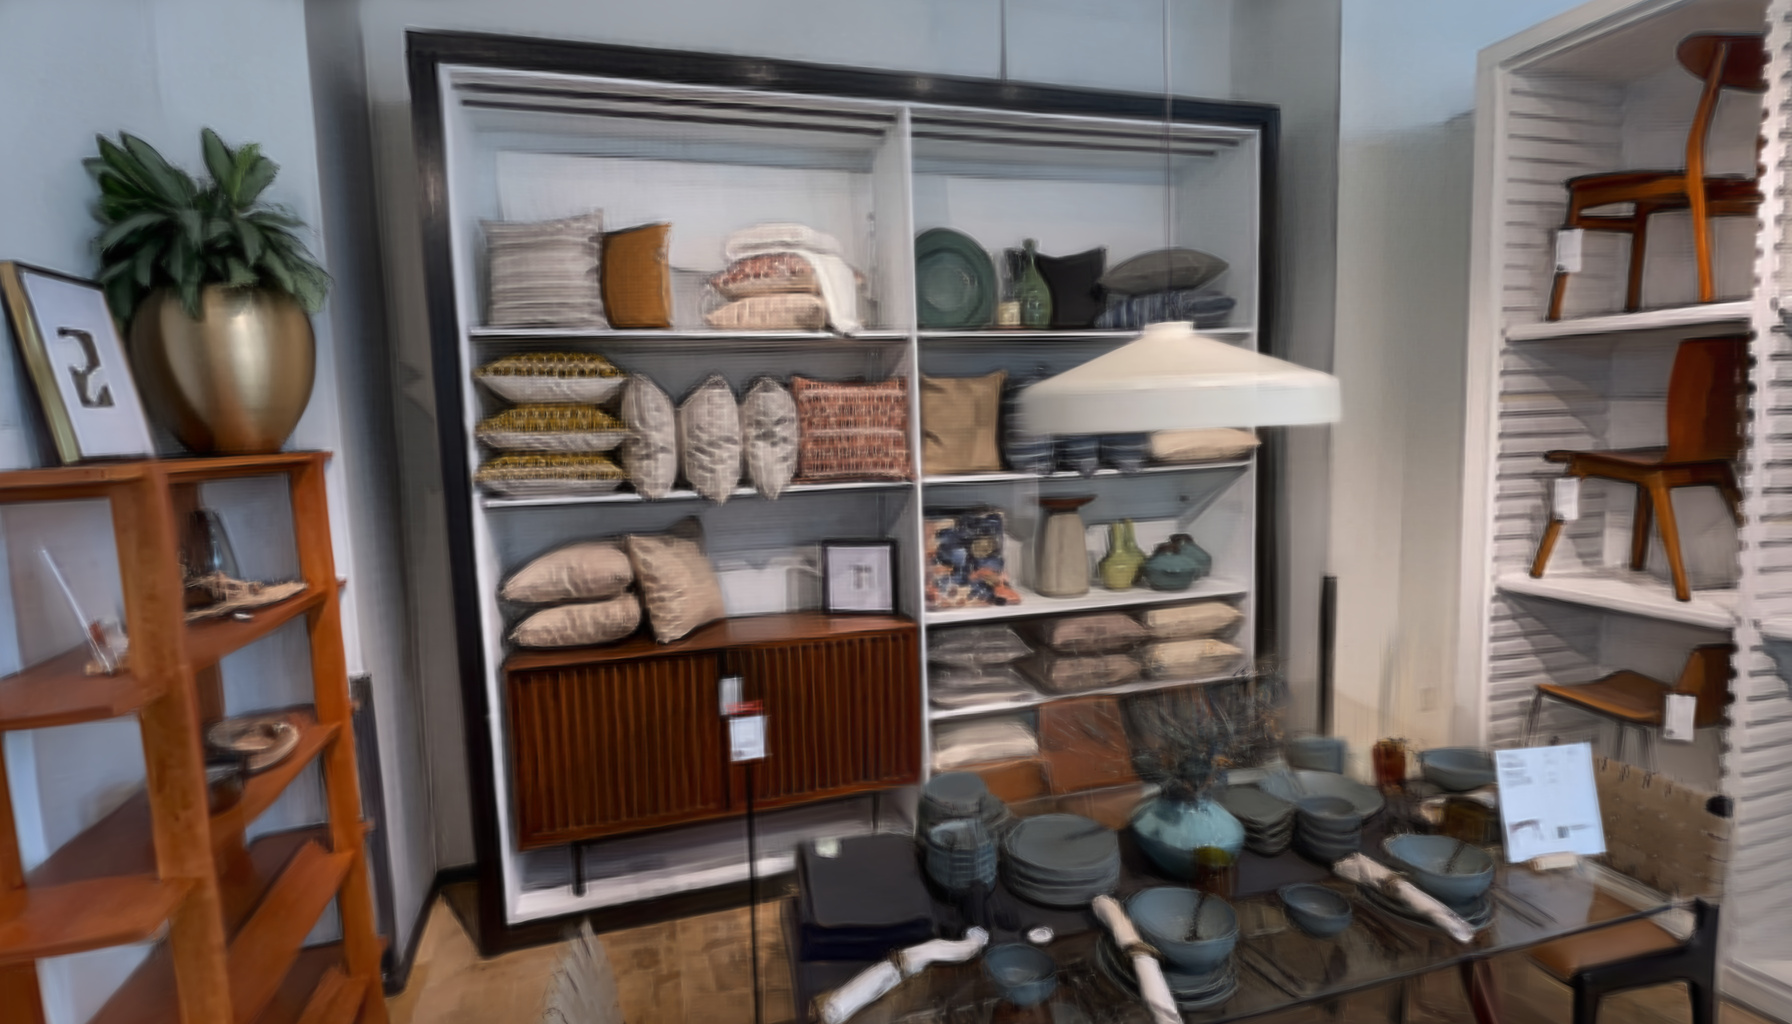} \\

        \includegraphics[width=0.32\linewidth]{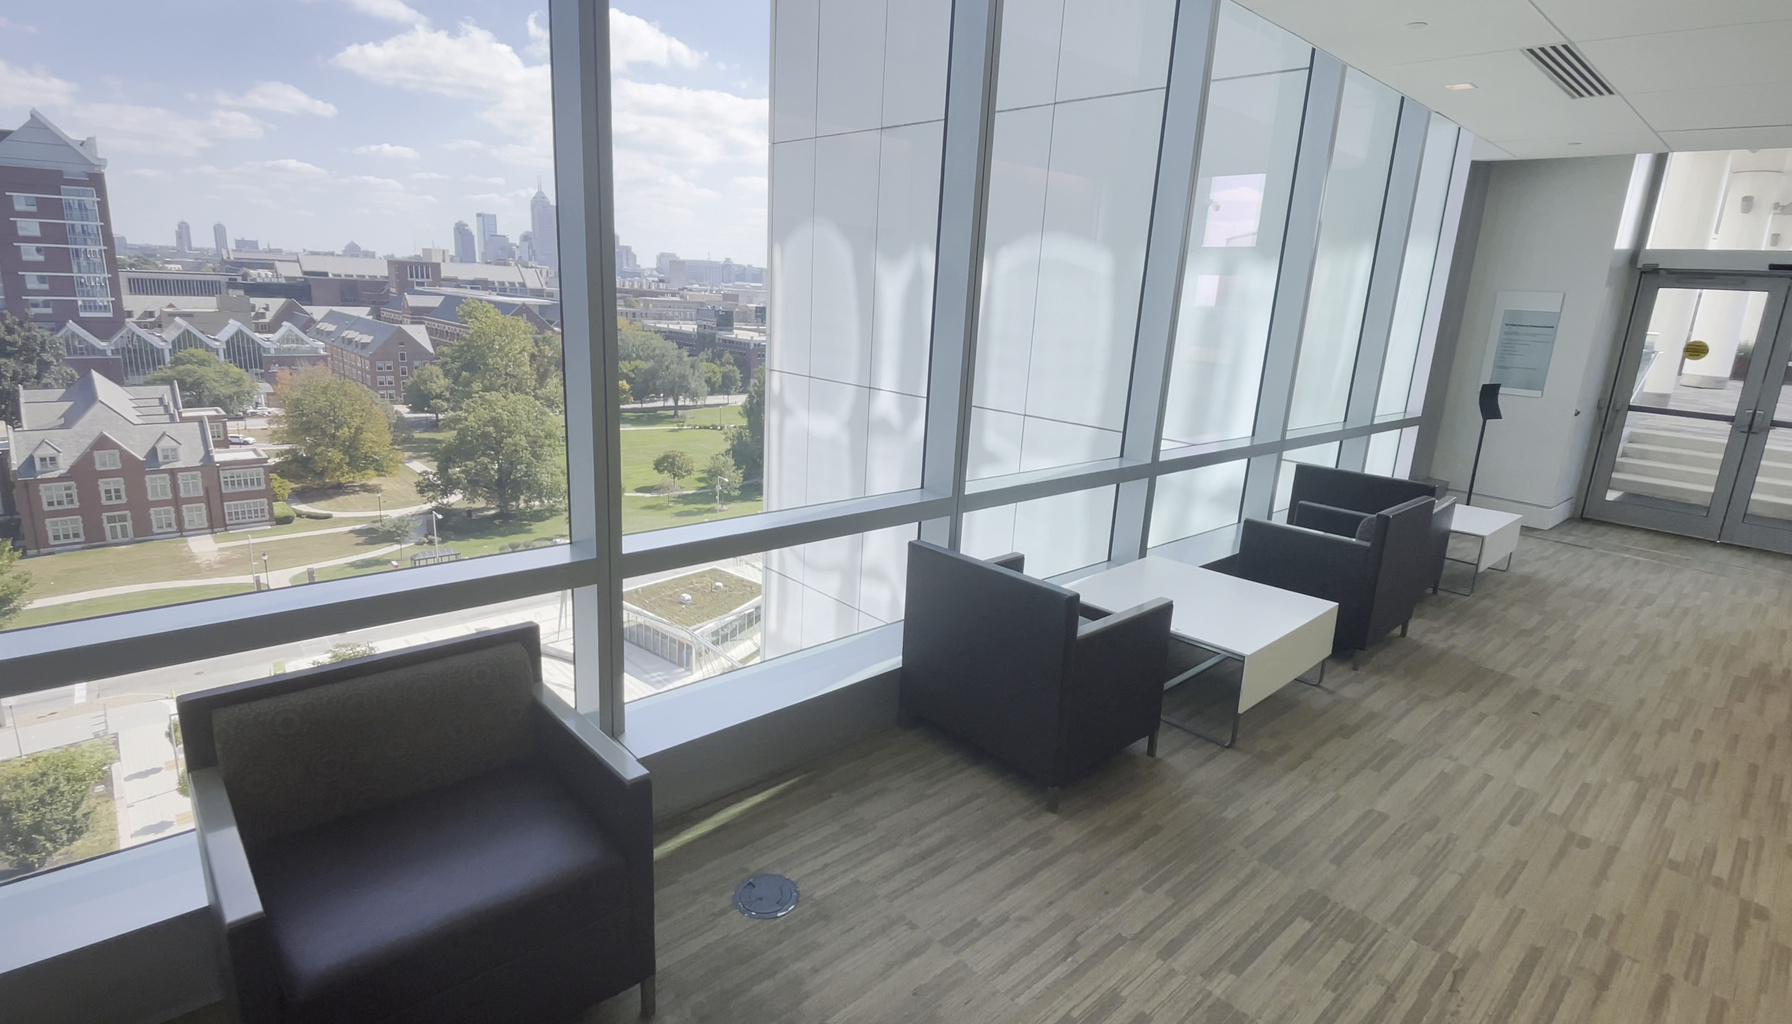} & 
        \includegraphics[width=0.32\linewidth]{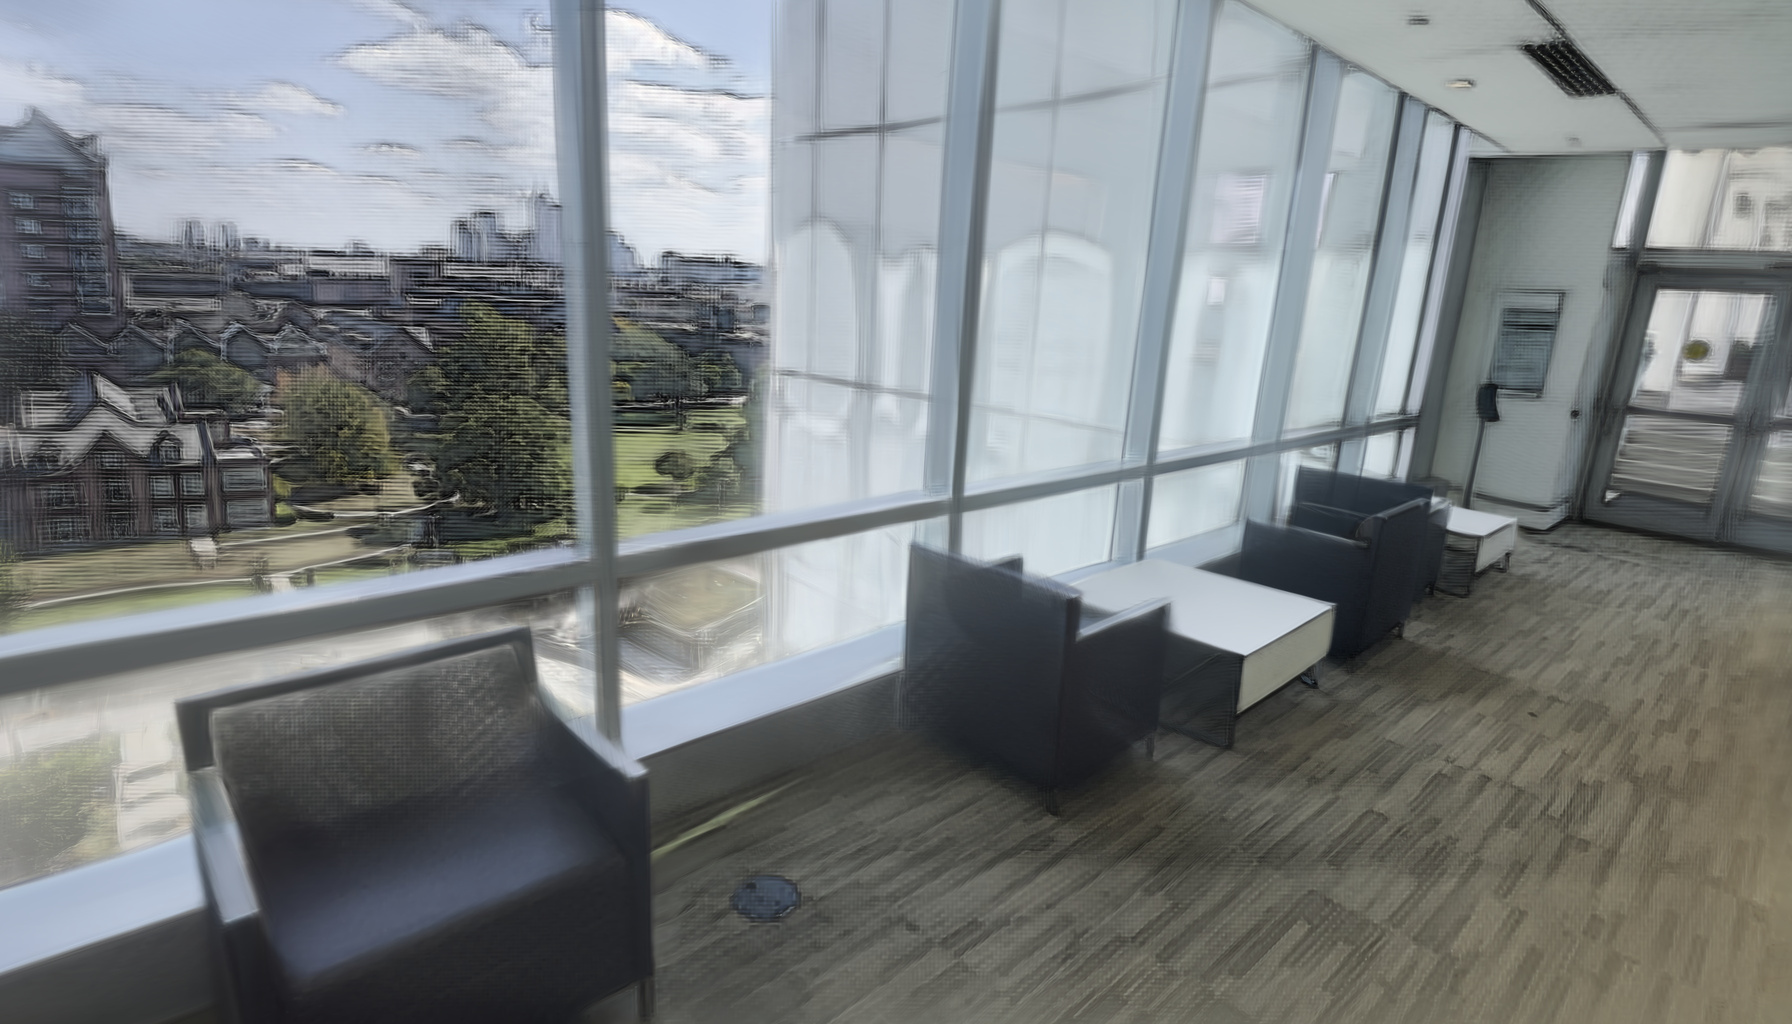} & 
        \includegraphics[width=0.32\linewidth]{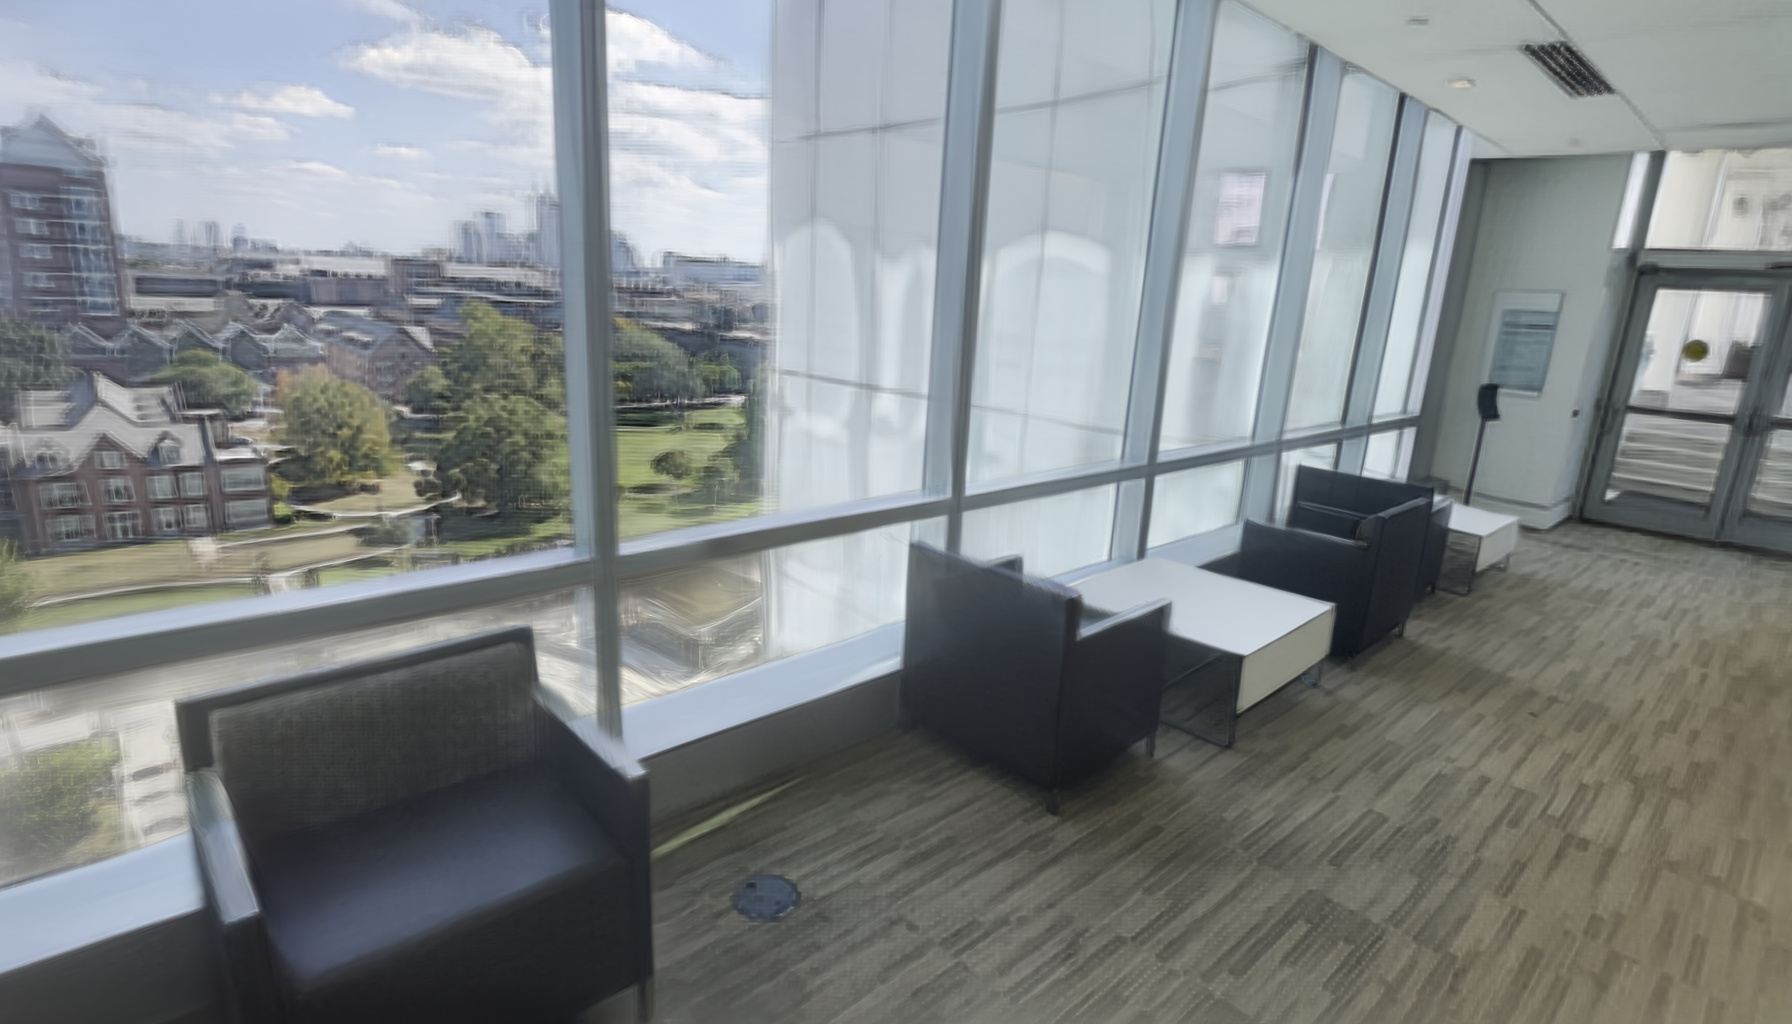} \\

        \includegraphics[width=0.32\linewidth]{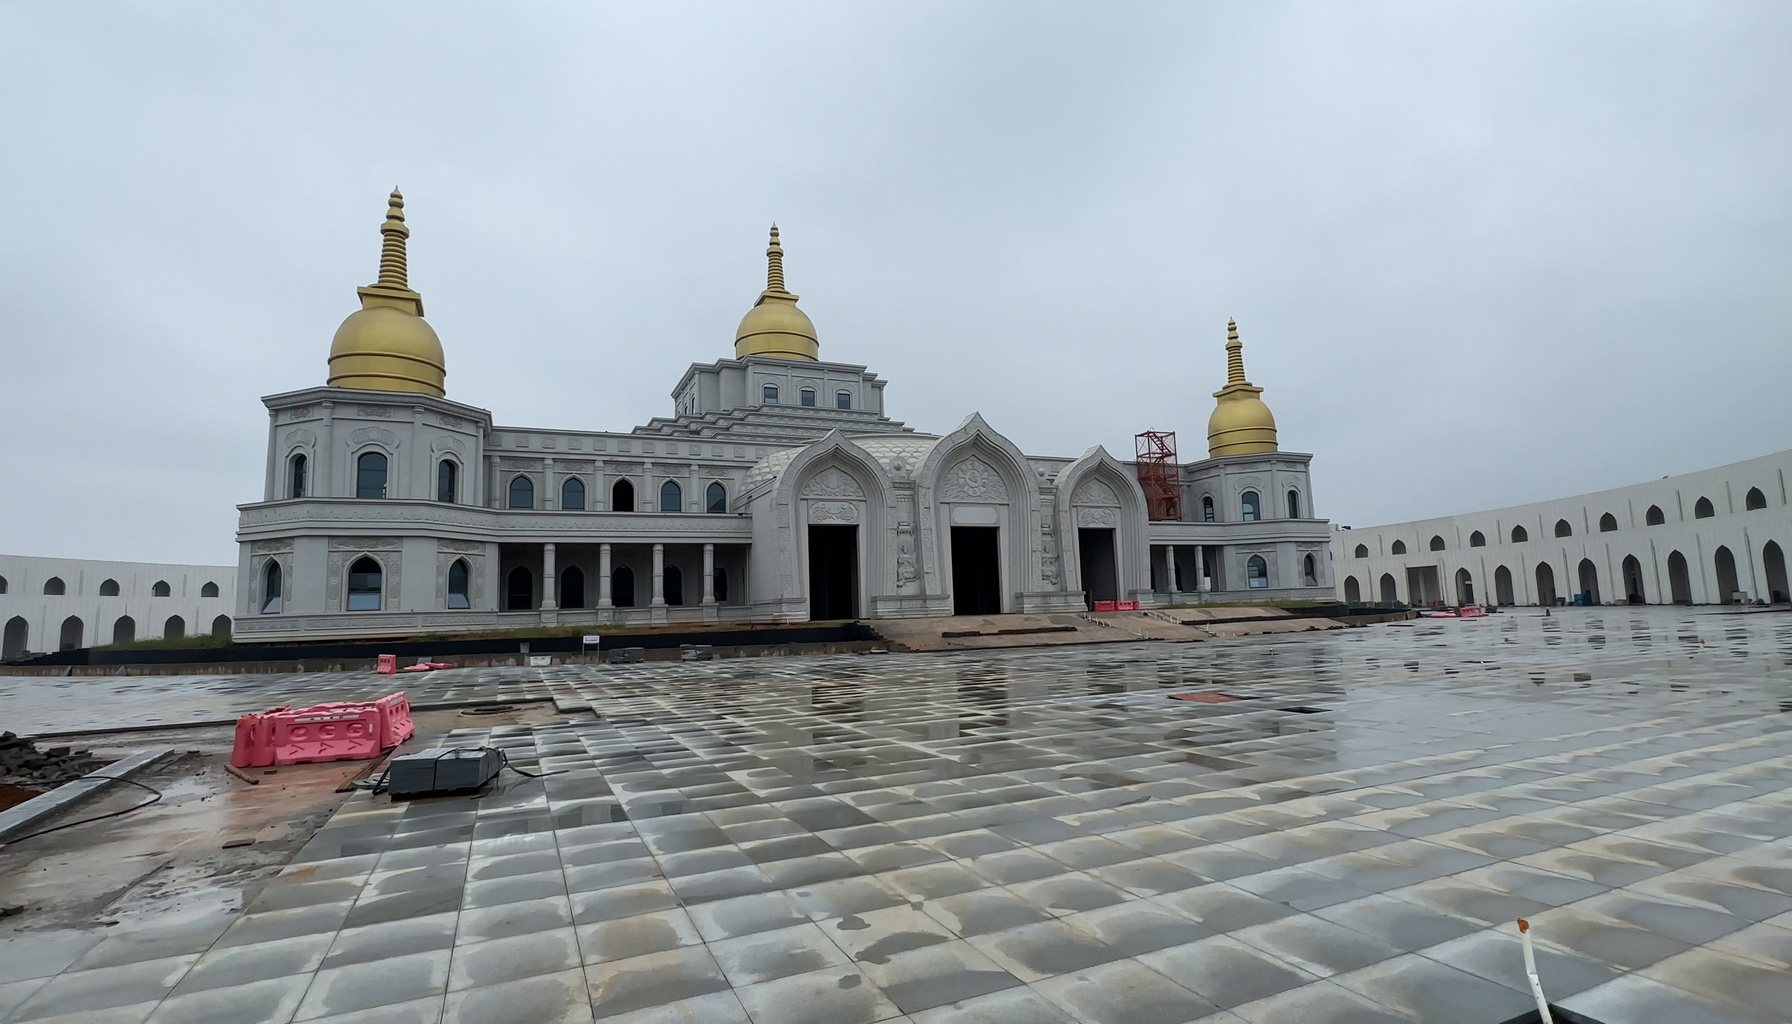} & 
        \includegraphics[width=0.32\linewidth]{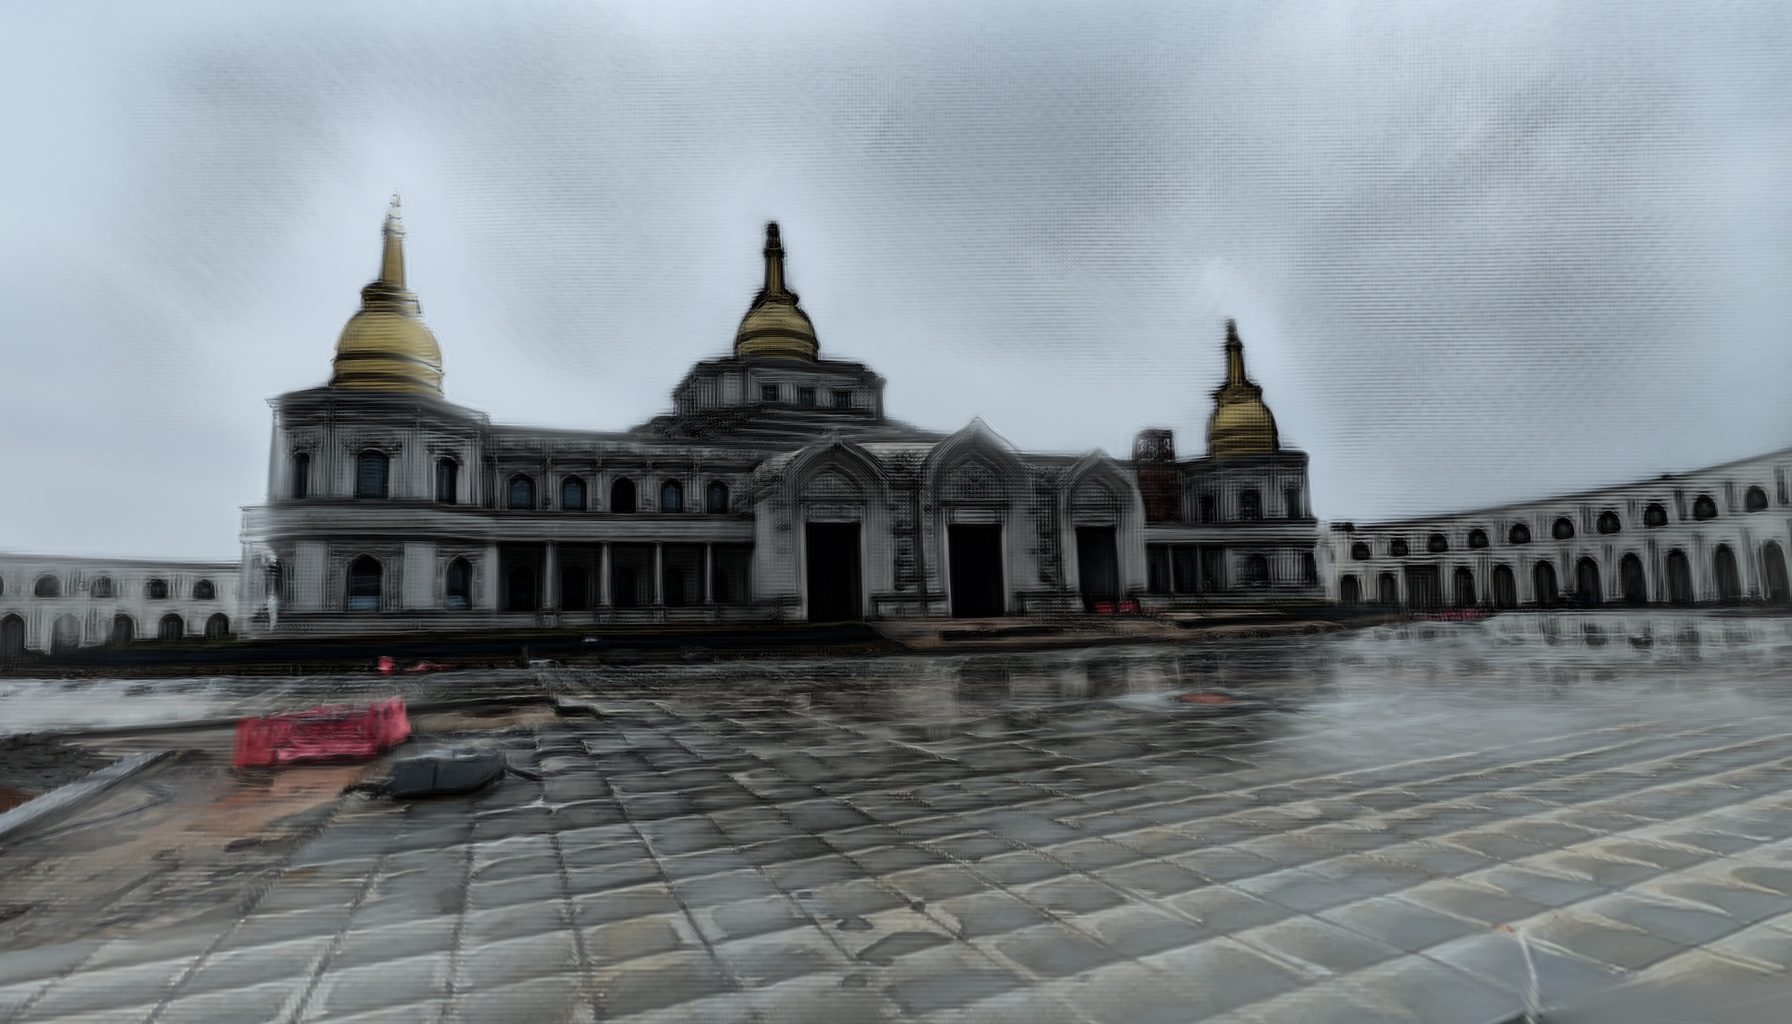} & 
        \includegraphics[width=0.32\linewidth]{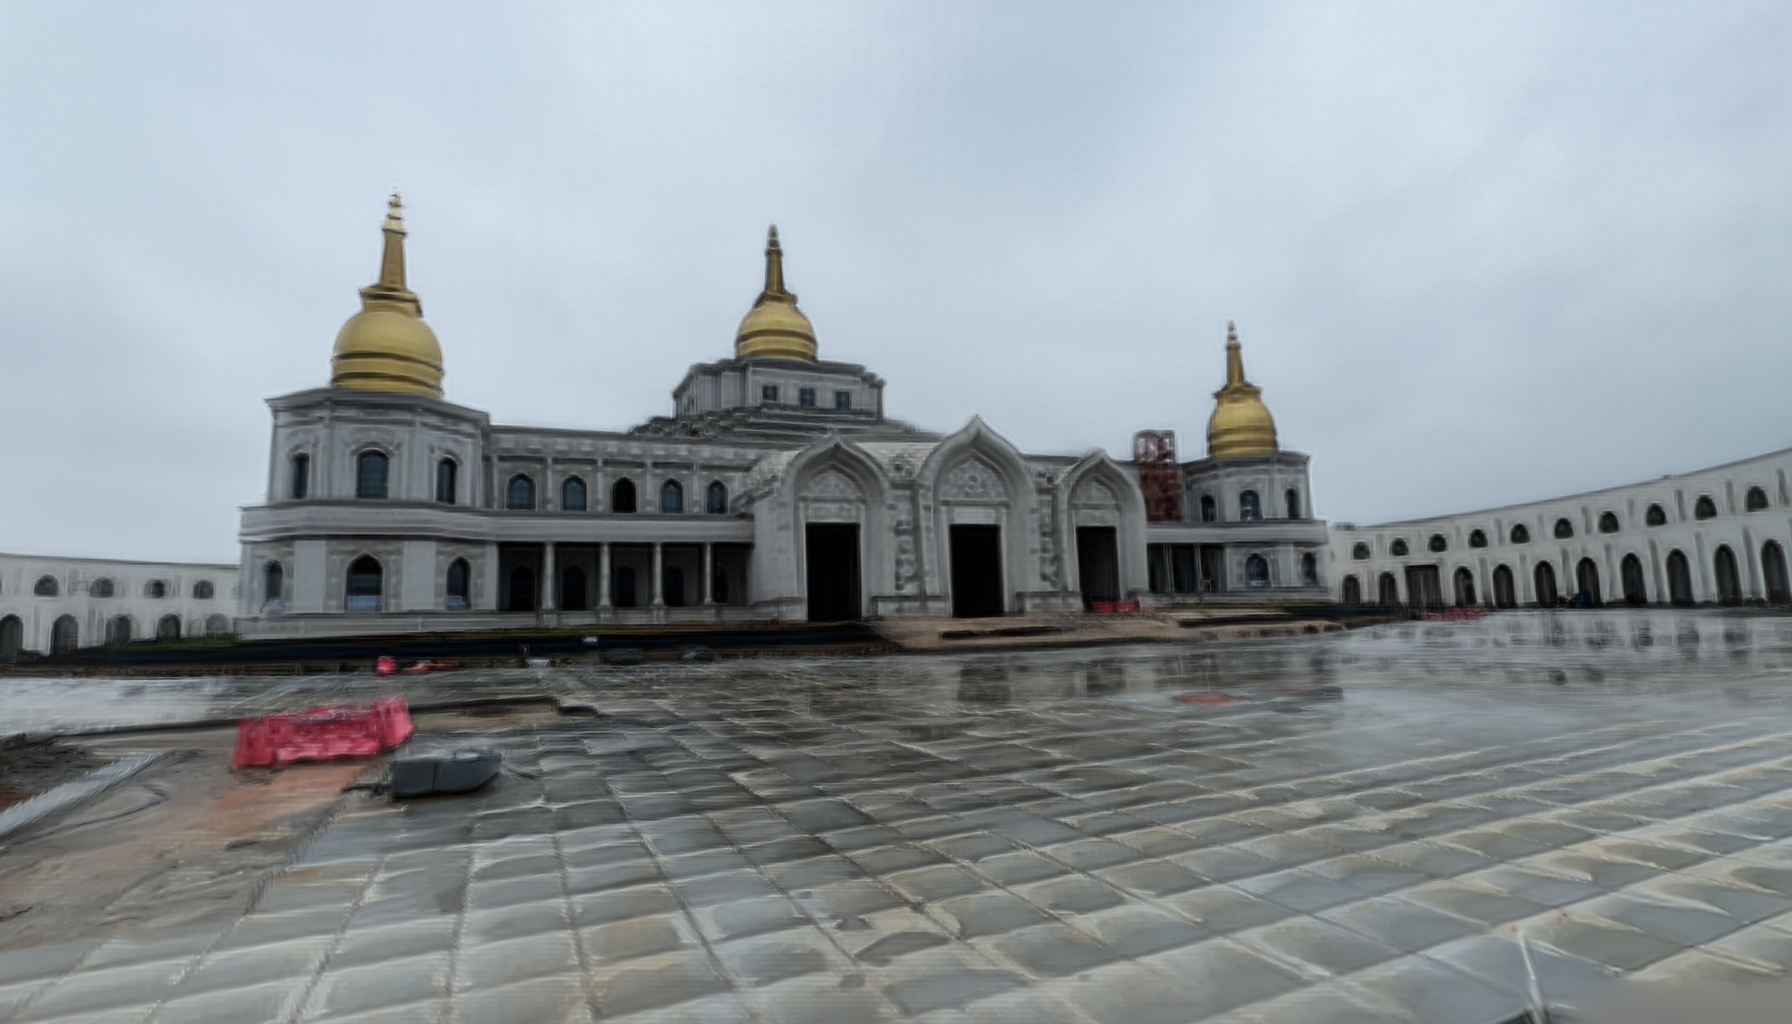} \\

        % --- Row 2 Images ---
        \includegraphics[width=0.32\linewidth]{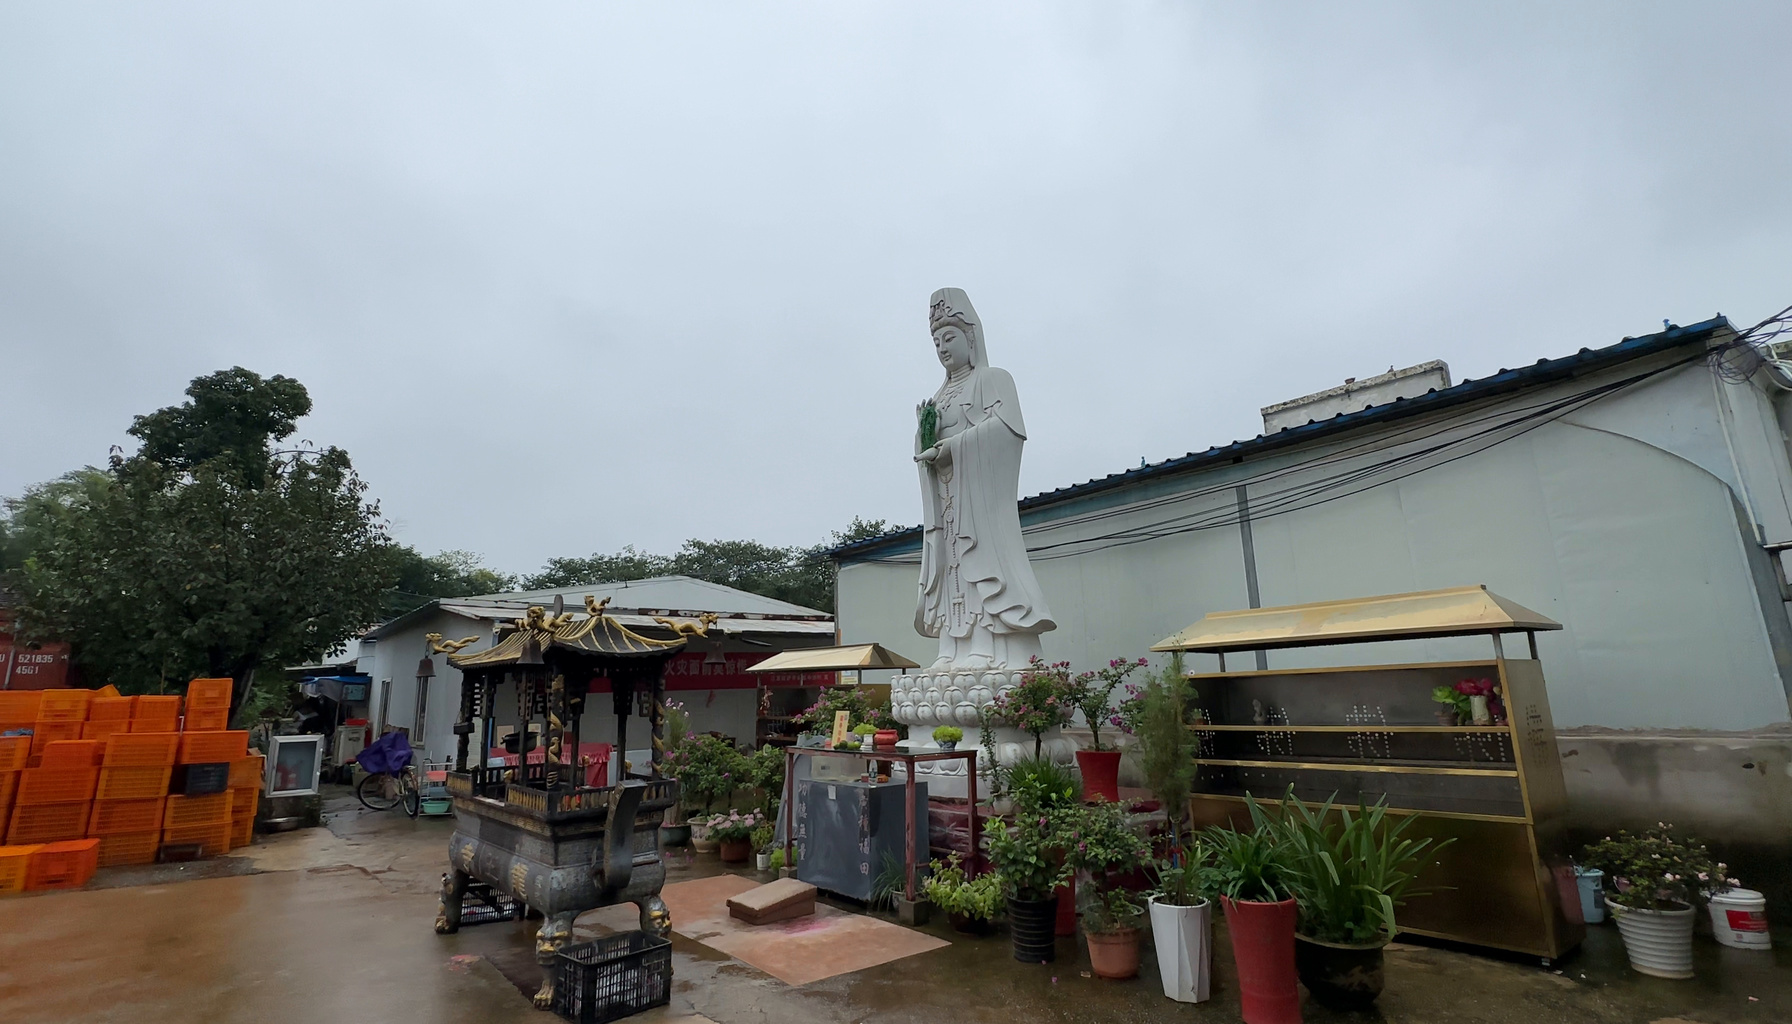} & 
        \includegraphics[width=0.32\linewidth]{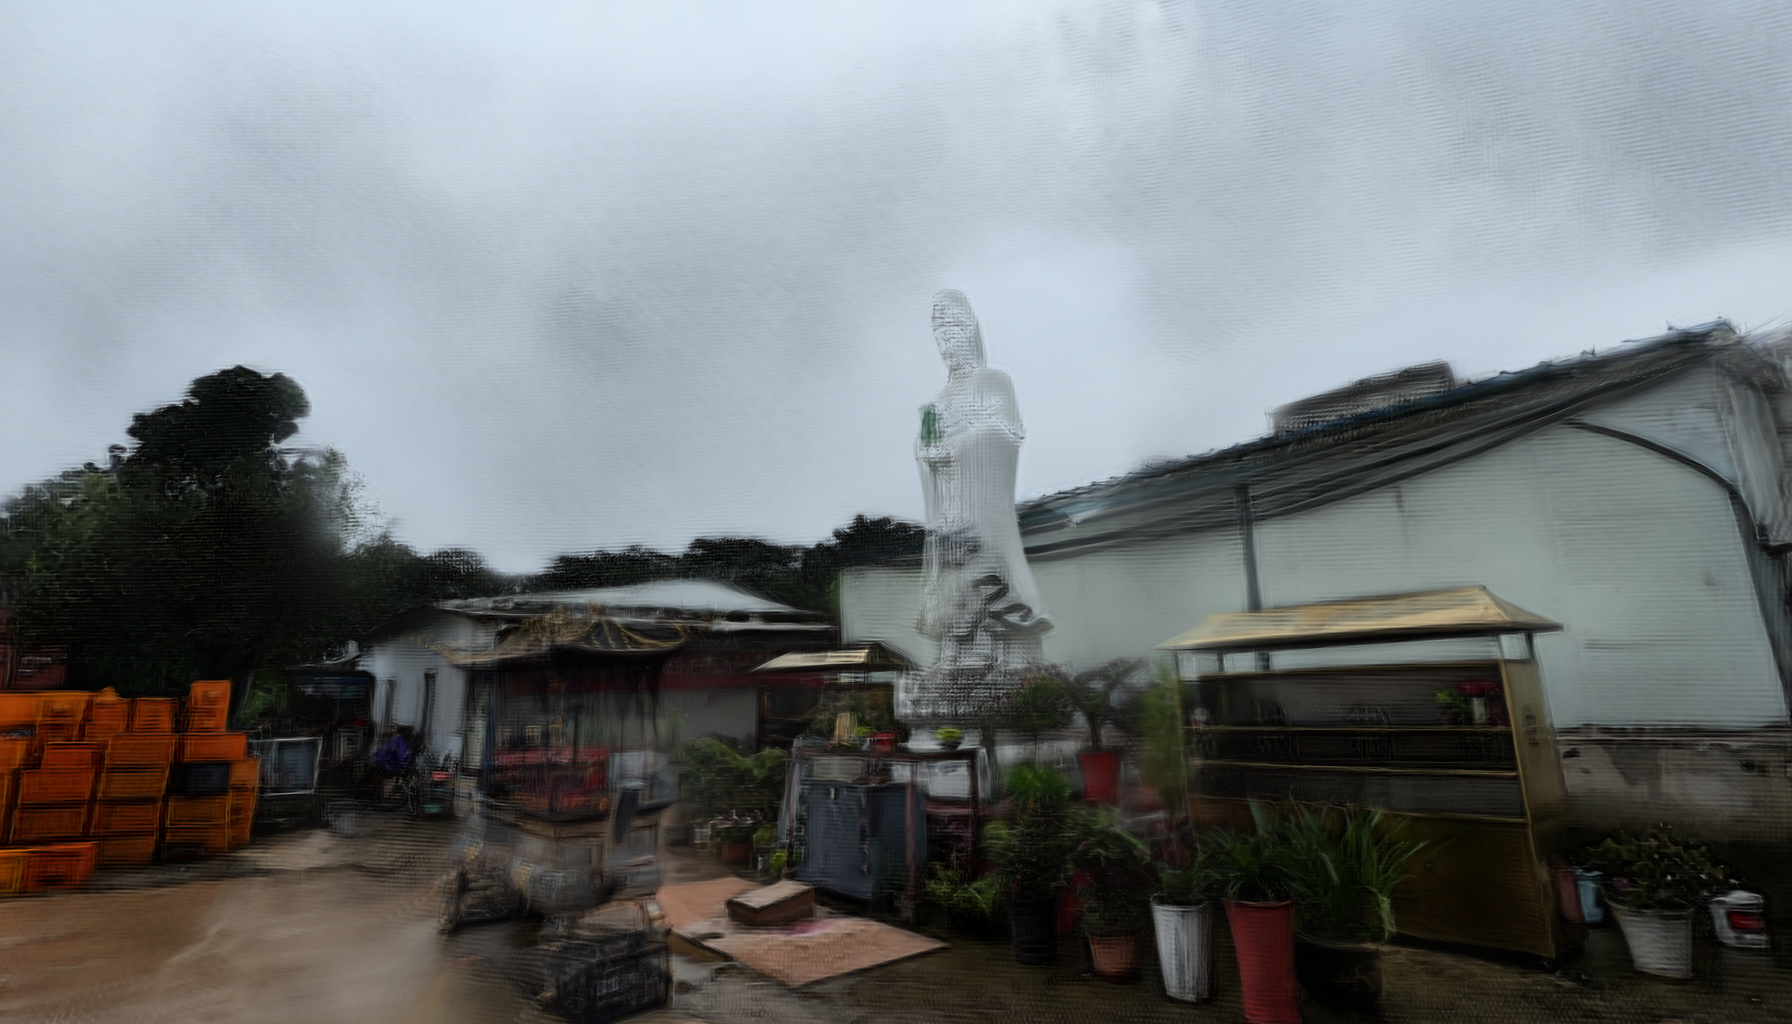} & 
        \includegraphics[width=0.32\linewidth]{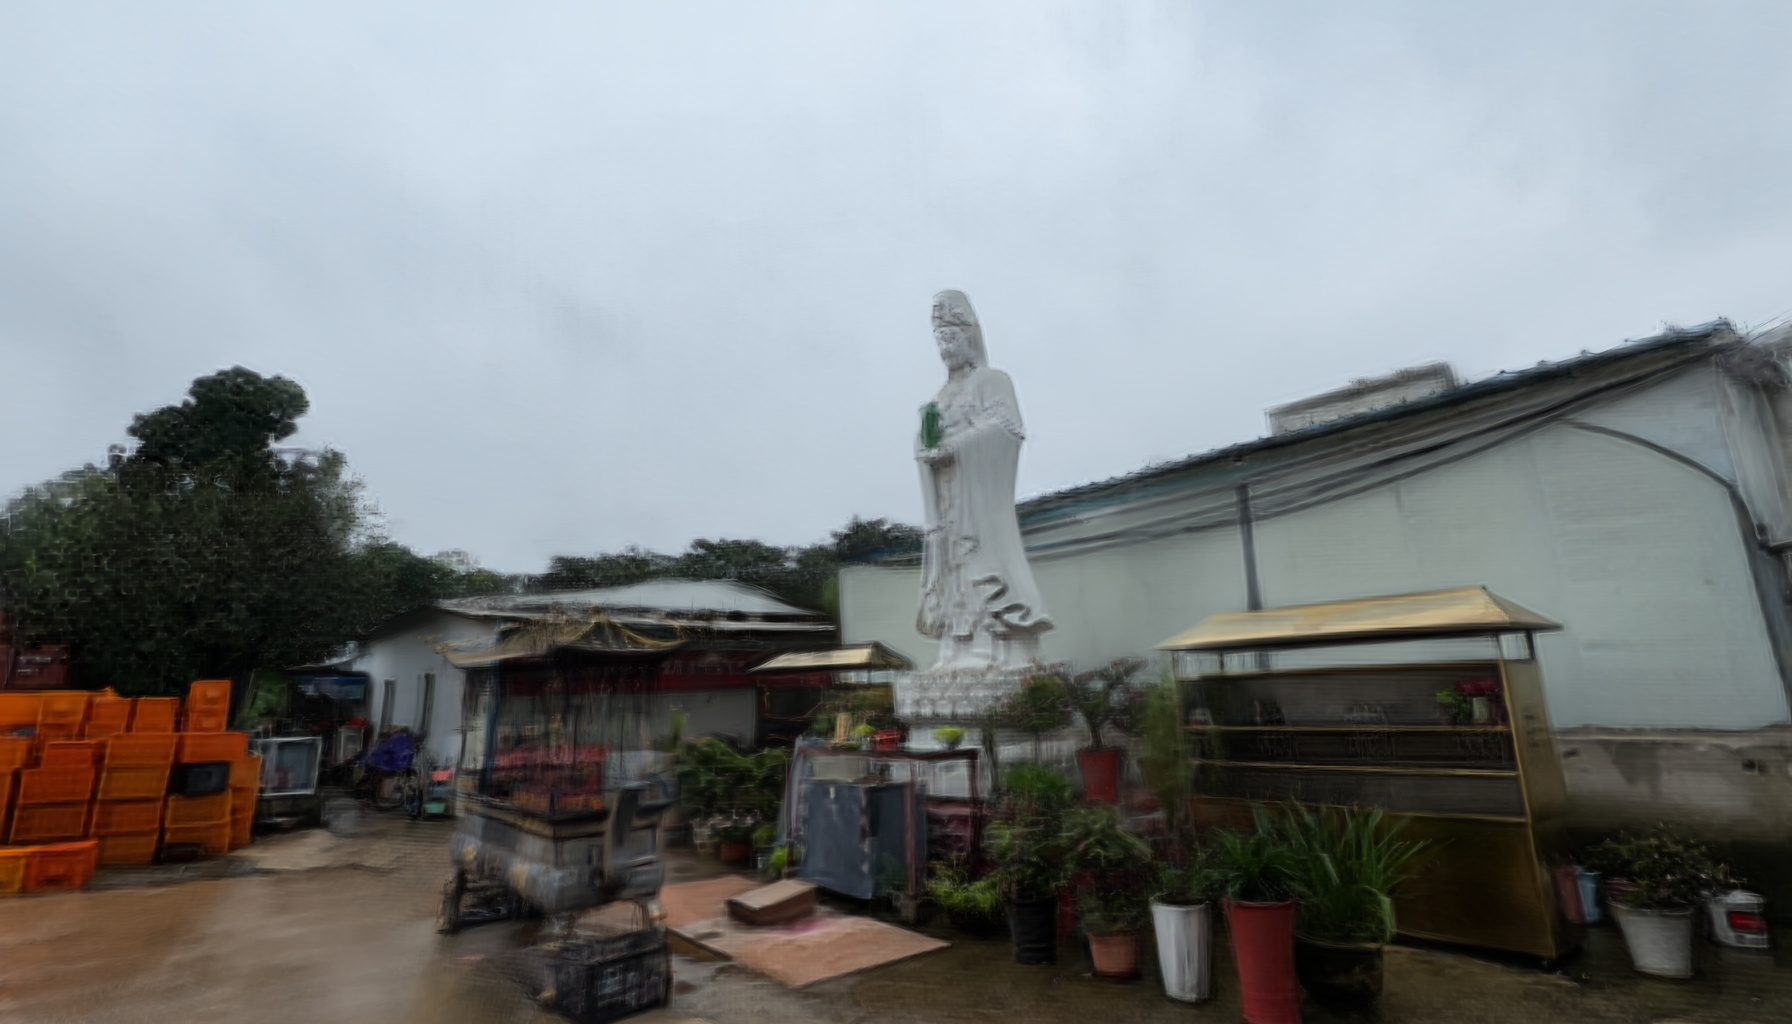} \\
        
        \includegraphics[width=0.32\linewidth]{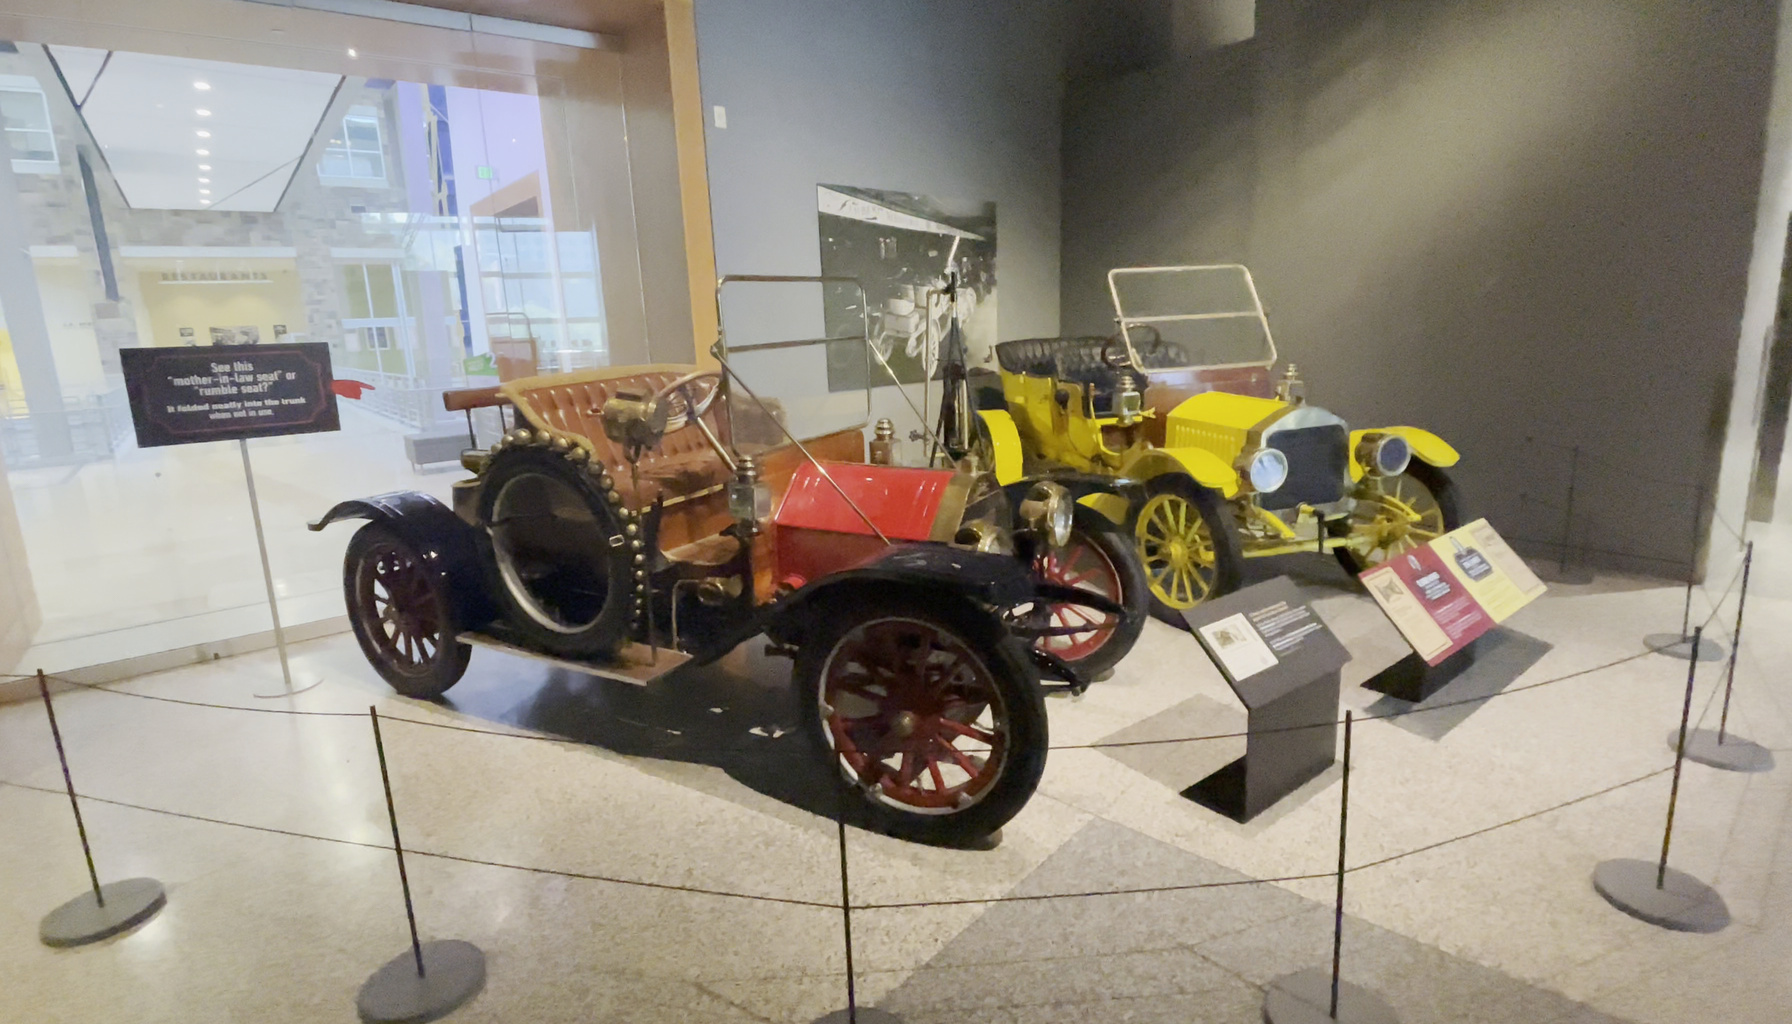} & 
        \includegraphics[width=0.32\linewidth]{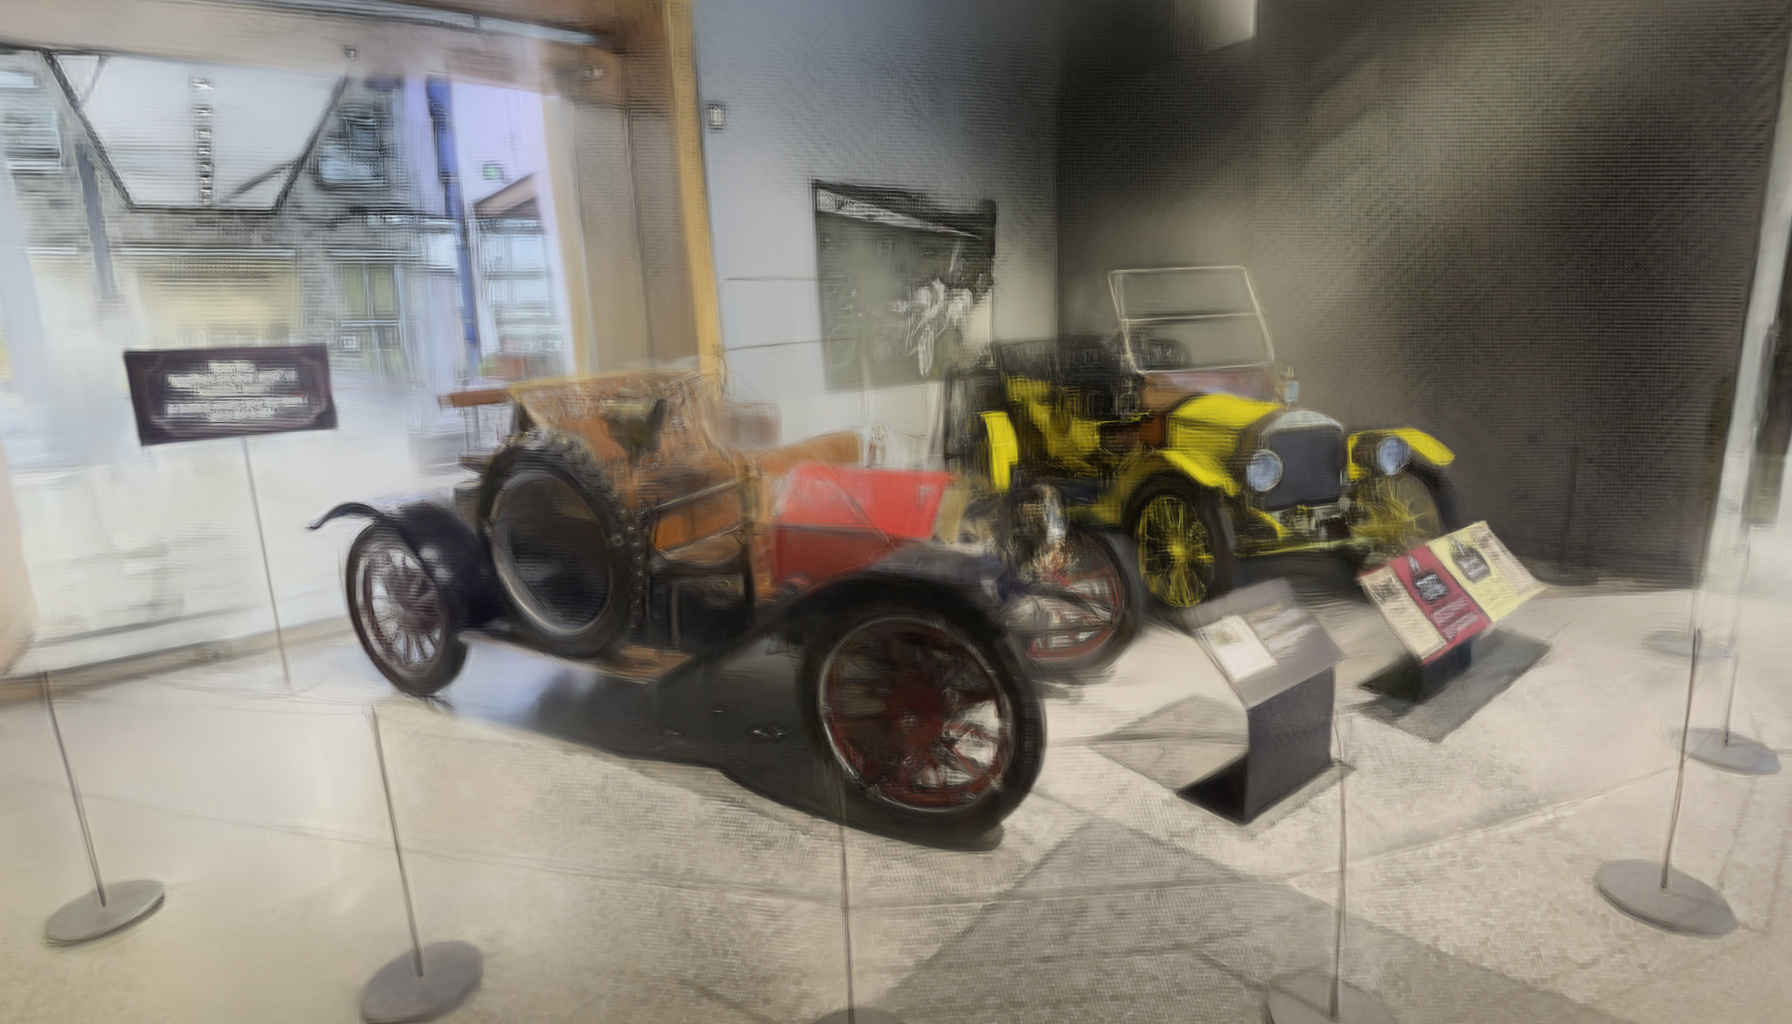} & 
        \includegraphics[width=0.32\linewidth]{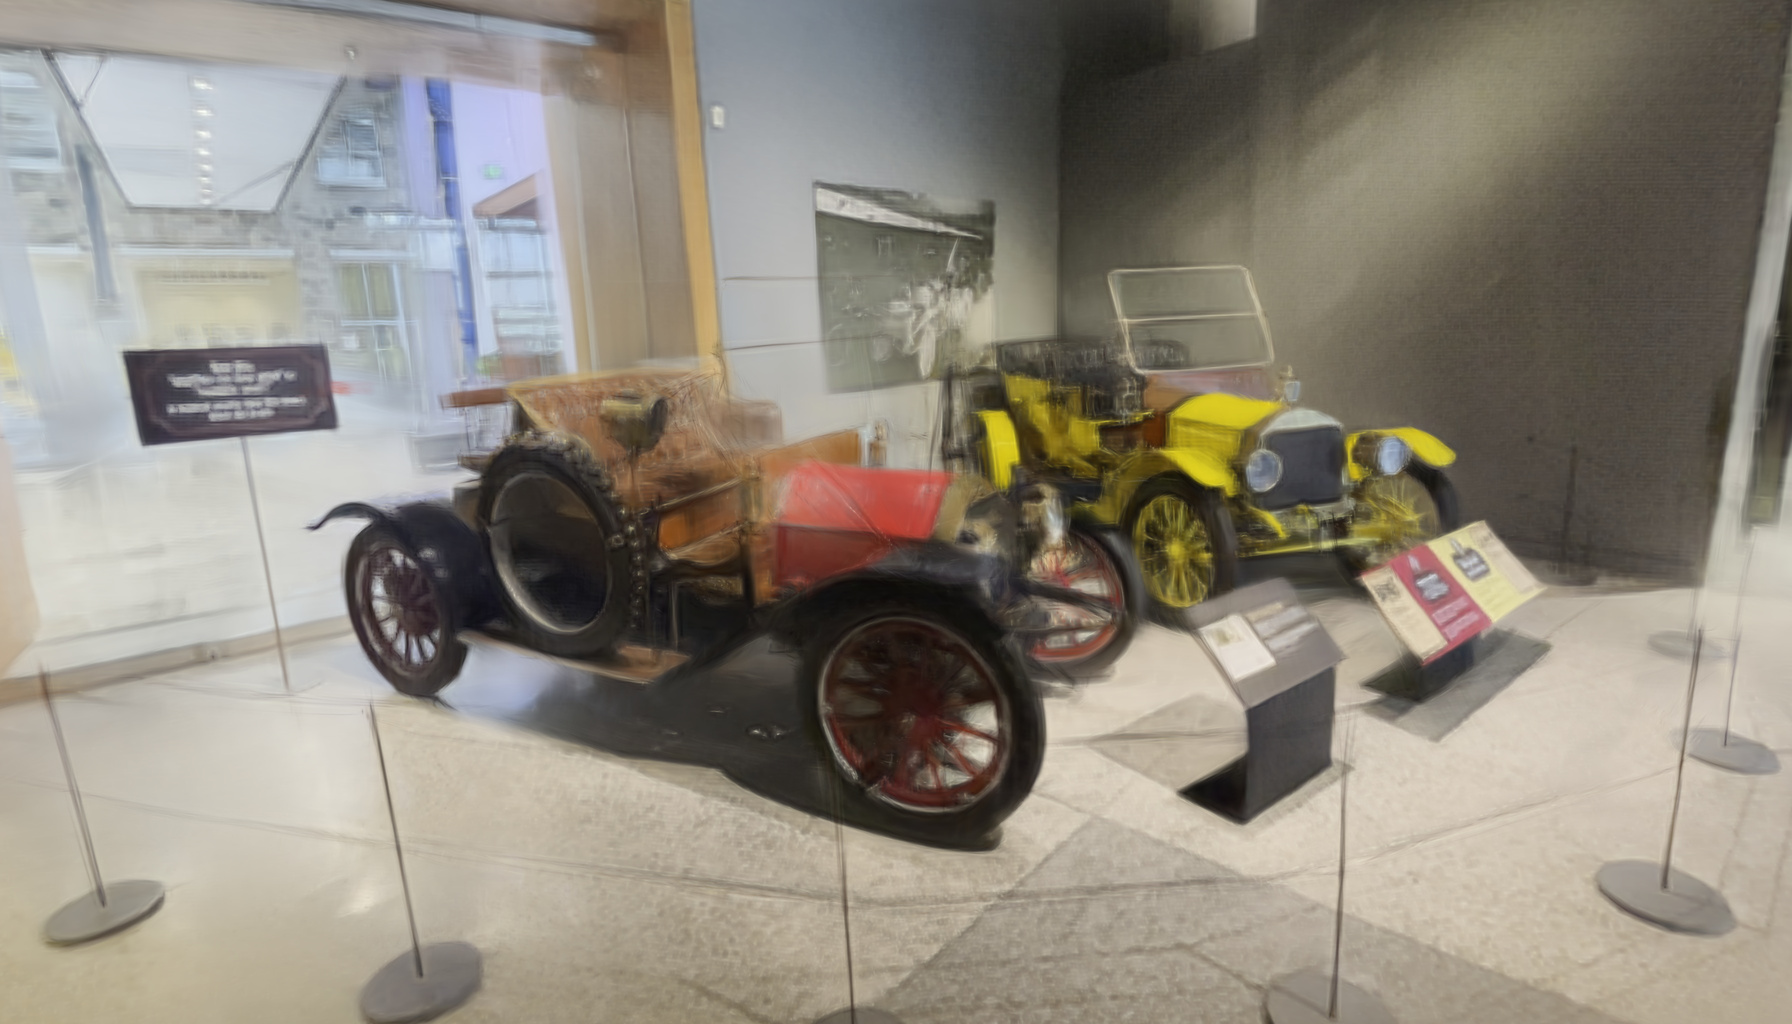} \\

        \includegraphics[width=0.32\linewidth]{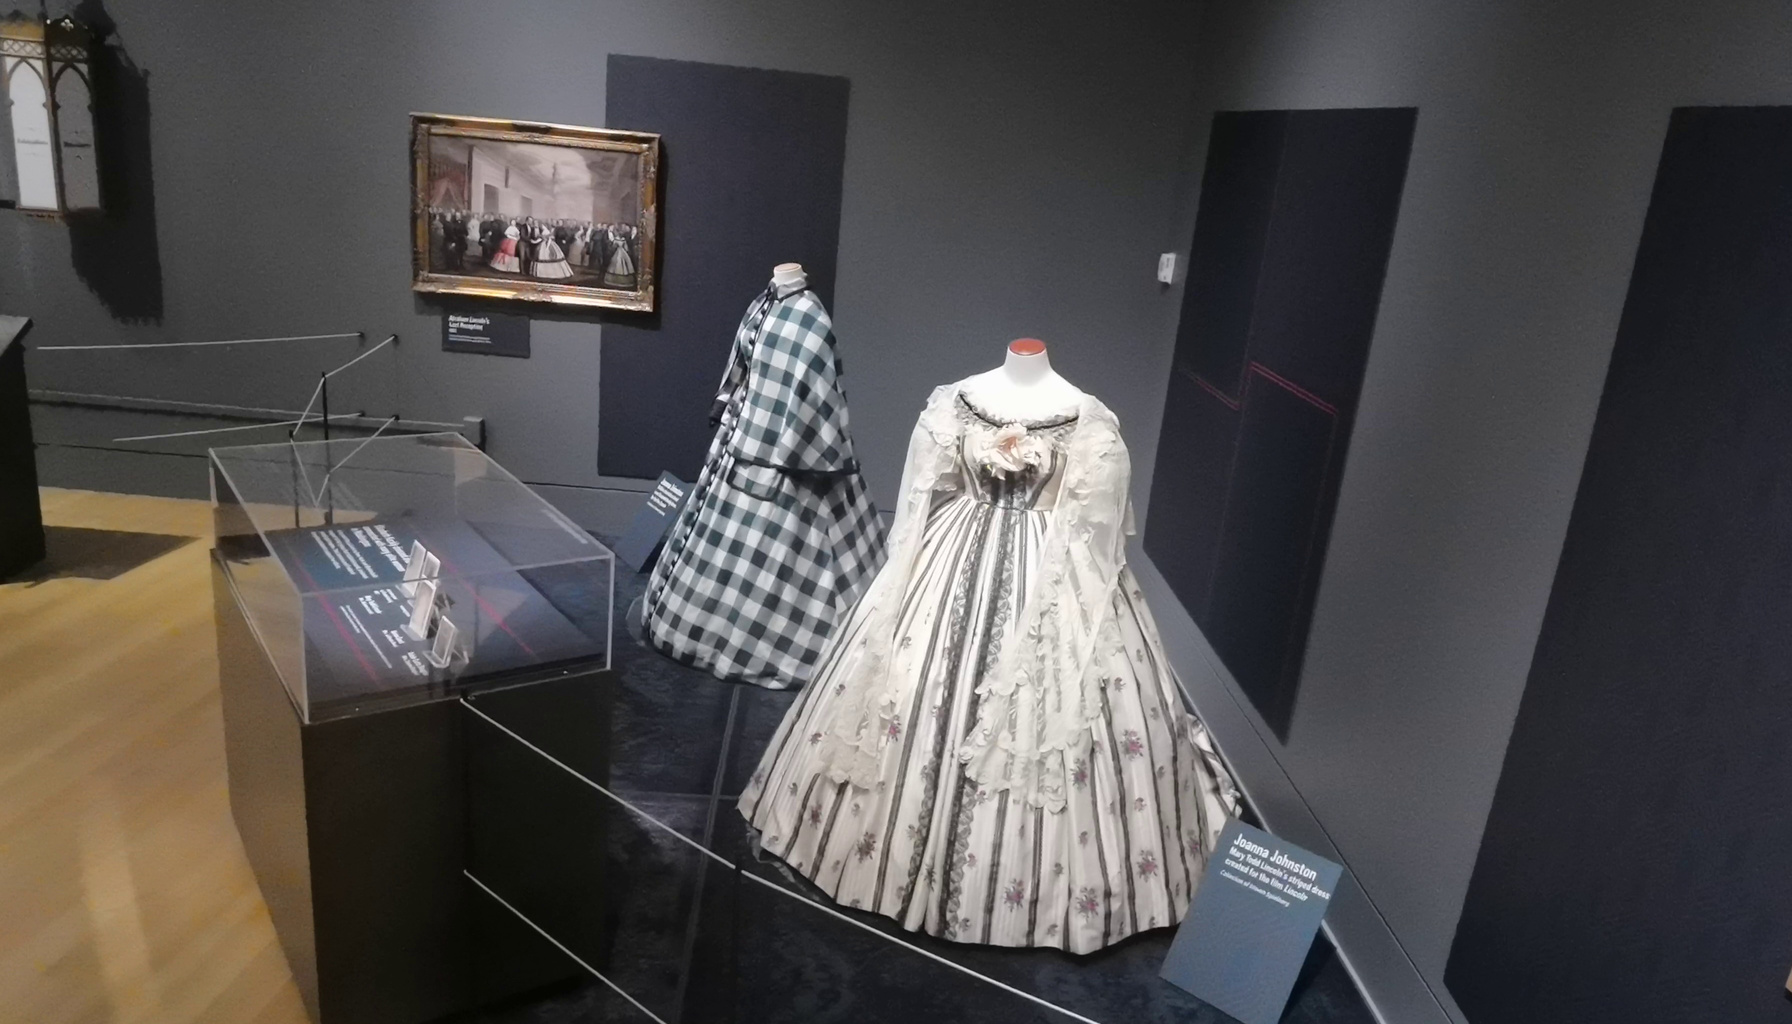} & 
        \includegraphics[width=0.32\linewidth]{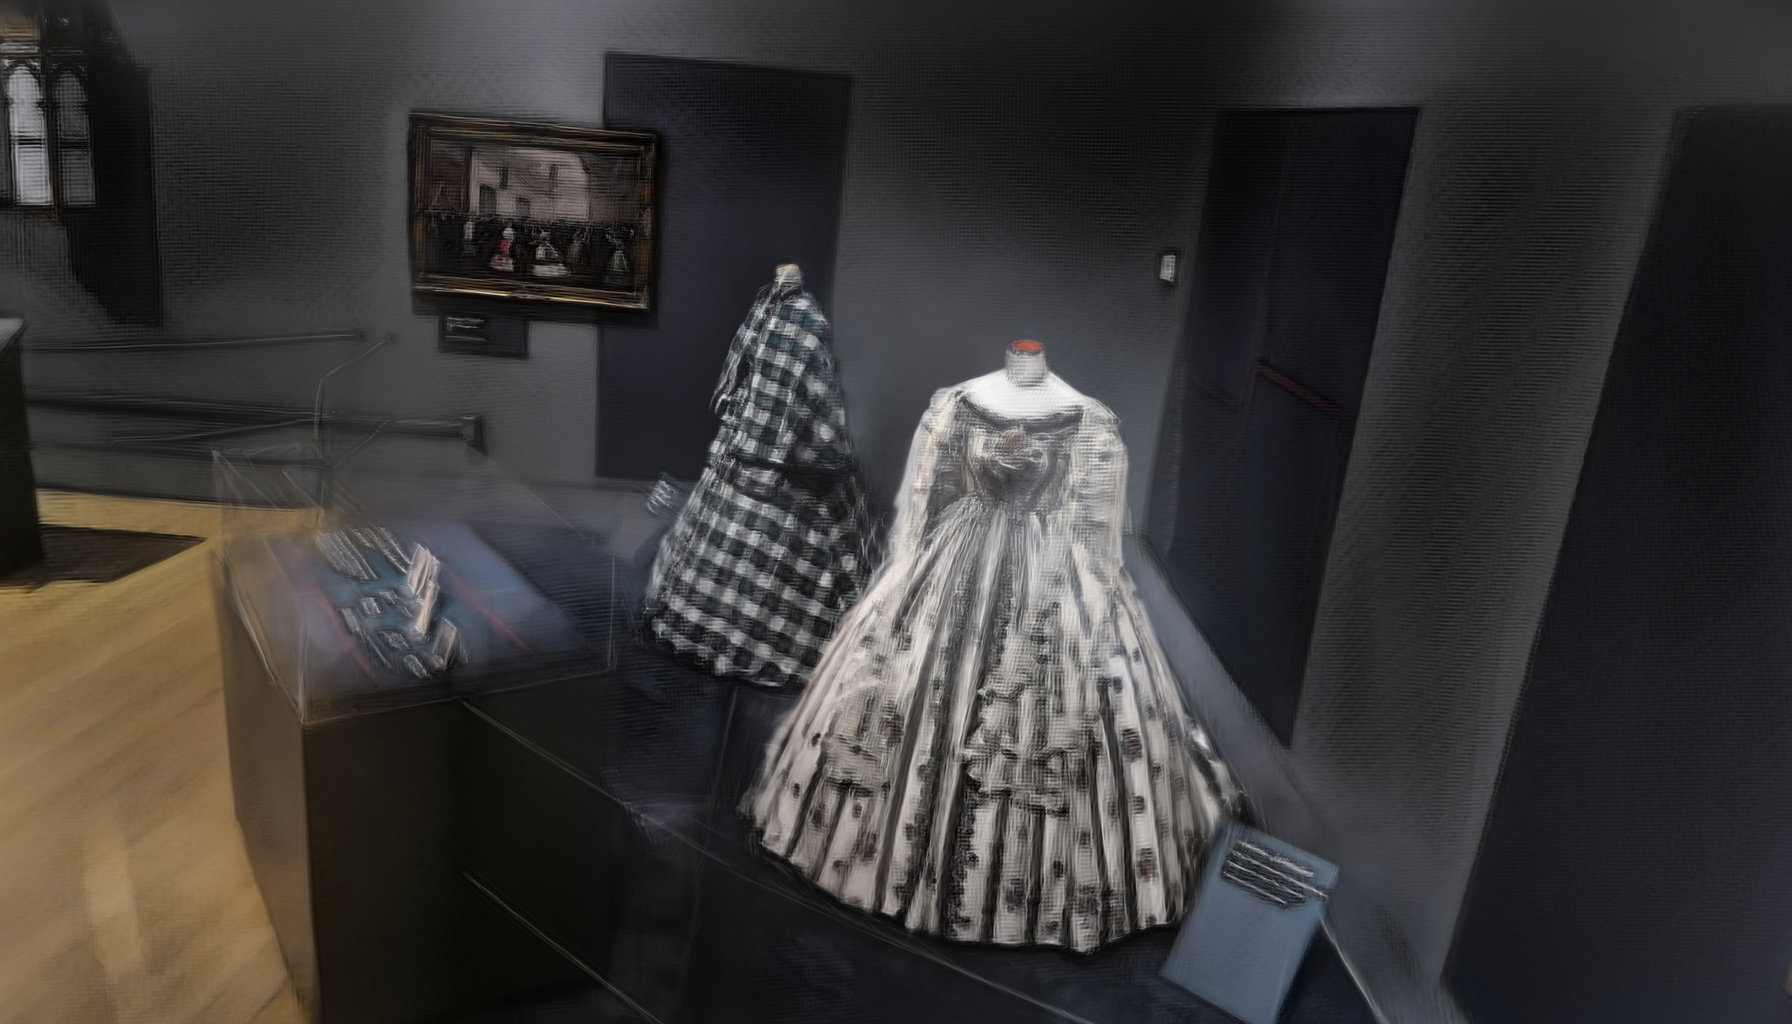} & 
        \includegraphics[width=0.32\linewidth]{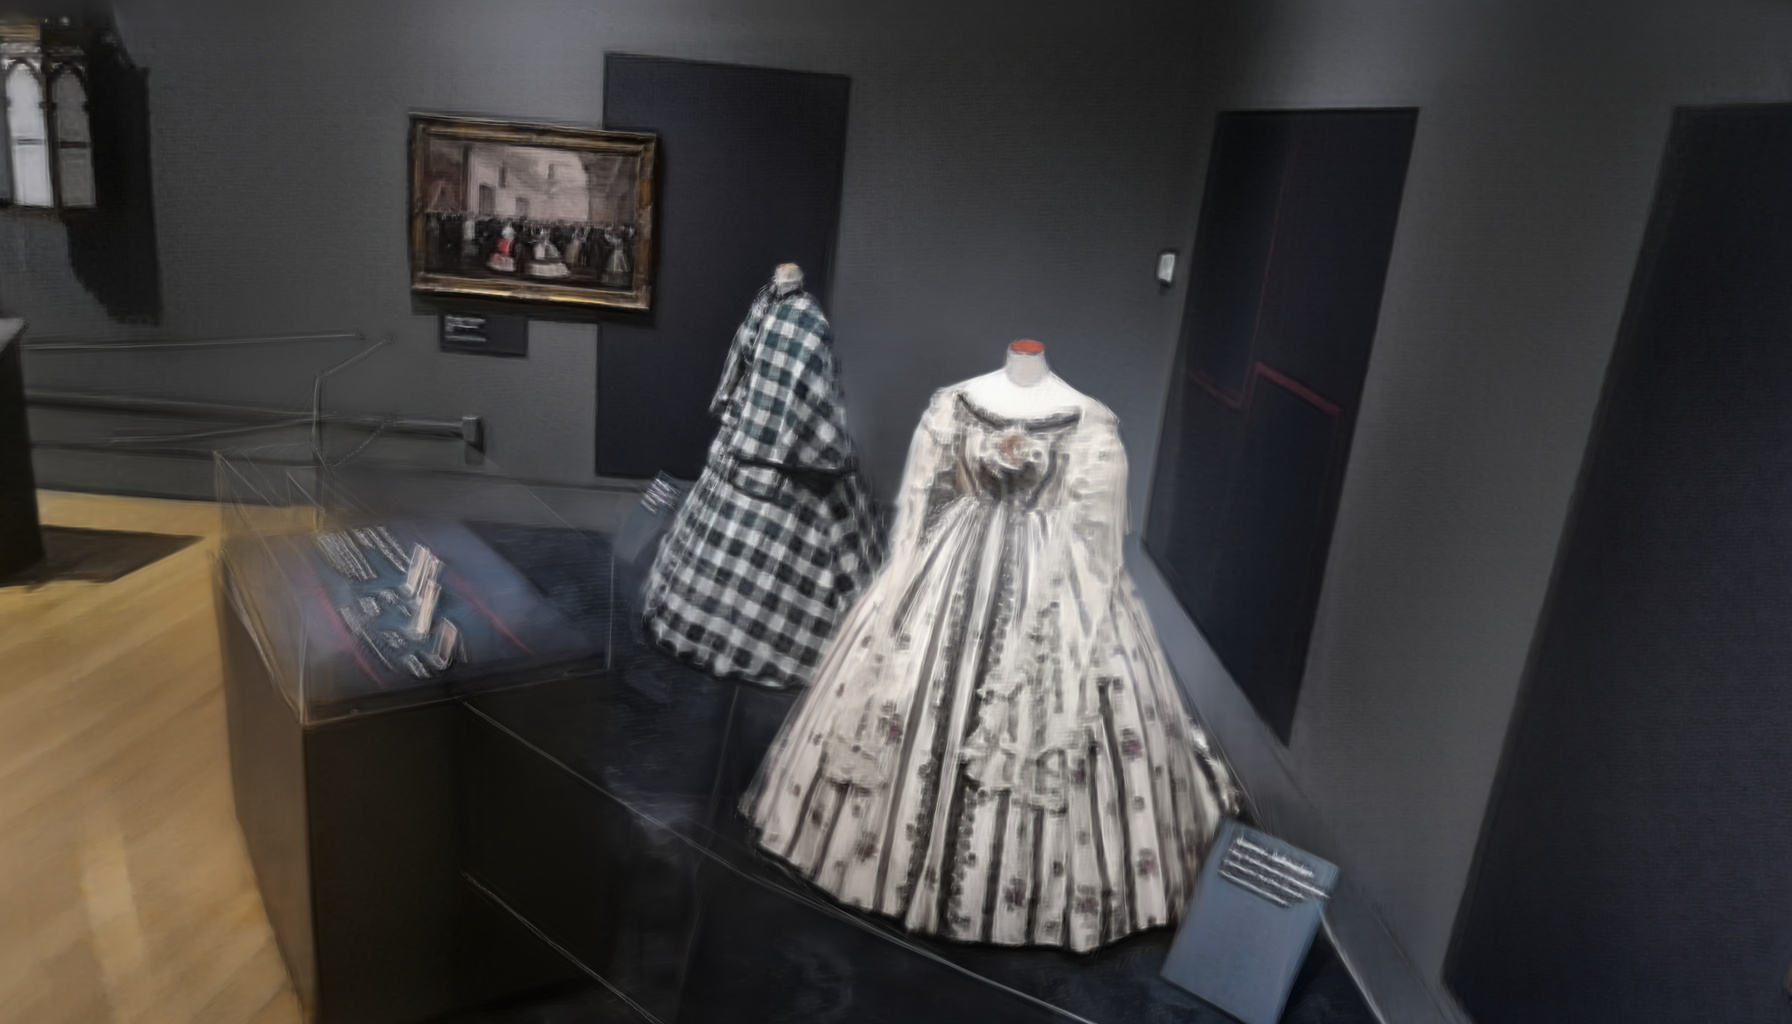} \\
        
    \end{tabular}
    
    \caption{\textbf{High-resolution rendering on DL3DV dataset}. Our method significantly alleviates the holes issues exhibited by DepthSplat~\cite{xu2025depthsplat}. }
    \label{fig:qualitative_result_high_resolution}
\end{figure}
