# Supplementary material for: RoSplat: Robust Feed-Forward Pixel-wise Gaussian Splatting for Varying Input Views and High-Resolution Rendering
Source: arXiv:2605.13093 source file (2026-05-13)
Supplement: Supplementary file 3 [file cross_dataset_evaluation.tex]

\section{Cross-dataset Evaluation}
For cross-dataset evaluation, we follow DepthSplat~\cite{xu2025depthsplat} to train our method on the RealEstate10K dataset by taking two images of resolution $256\times 448$ as inputs. We then evaluate the models on the DL3DV dataset using (1) the same configuration as training, (2) increase the number of input views to 6, (3) increase the rendering resolution to $2048\times 3584$. Tab.~\ref{tab:cross_dataset_evaluation} shows that our method retain similar performance compared to DepthSplat~\cite{xu2025depthsplat} under the same configuration used during training. On the other hand, our method demonstrates superiority when evaluated under test settings that differ from training. Specifically, when increasing the input views or rendering at high resolution, our method consistently achieve better image quality across all metrics compared to DepthSplat. This result further evidents the effectiveness of our proposed alpha normalization and 3D sampling-based regularizer.
