# Supplementary material for: RoSplat: Robust Feed-Forward Pixel-wise Gaussian Splatting for Varying Input Views and High-Resolution Rendering
Source: arXiv:2605.13093 source file (2026-05-13)
Supplement: Supplementary file 4 [file alpha_norm_curve.tex]

\begin{figure}[t]
\centering

    \begin{tabular}{ccc}
    \multicolumn{1}{c}{{MVSplat~\cite{chen2024mvsplat}}} &
    \multicolumn{1}{c}{{TranSplat~\cite{zhang2025transplat}}} &
    \multicolumn{1}{c}{{DepthSplat~\cite{xu2025depthsplat}}} \\
    
    \includegraphics[width=0.32\linewidth]{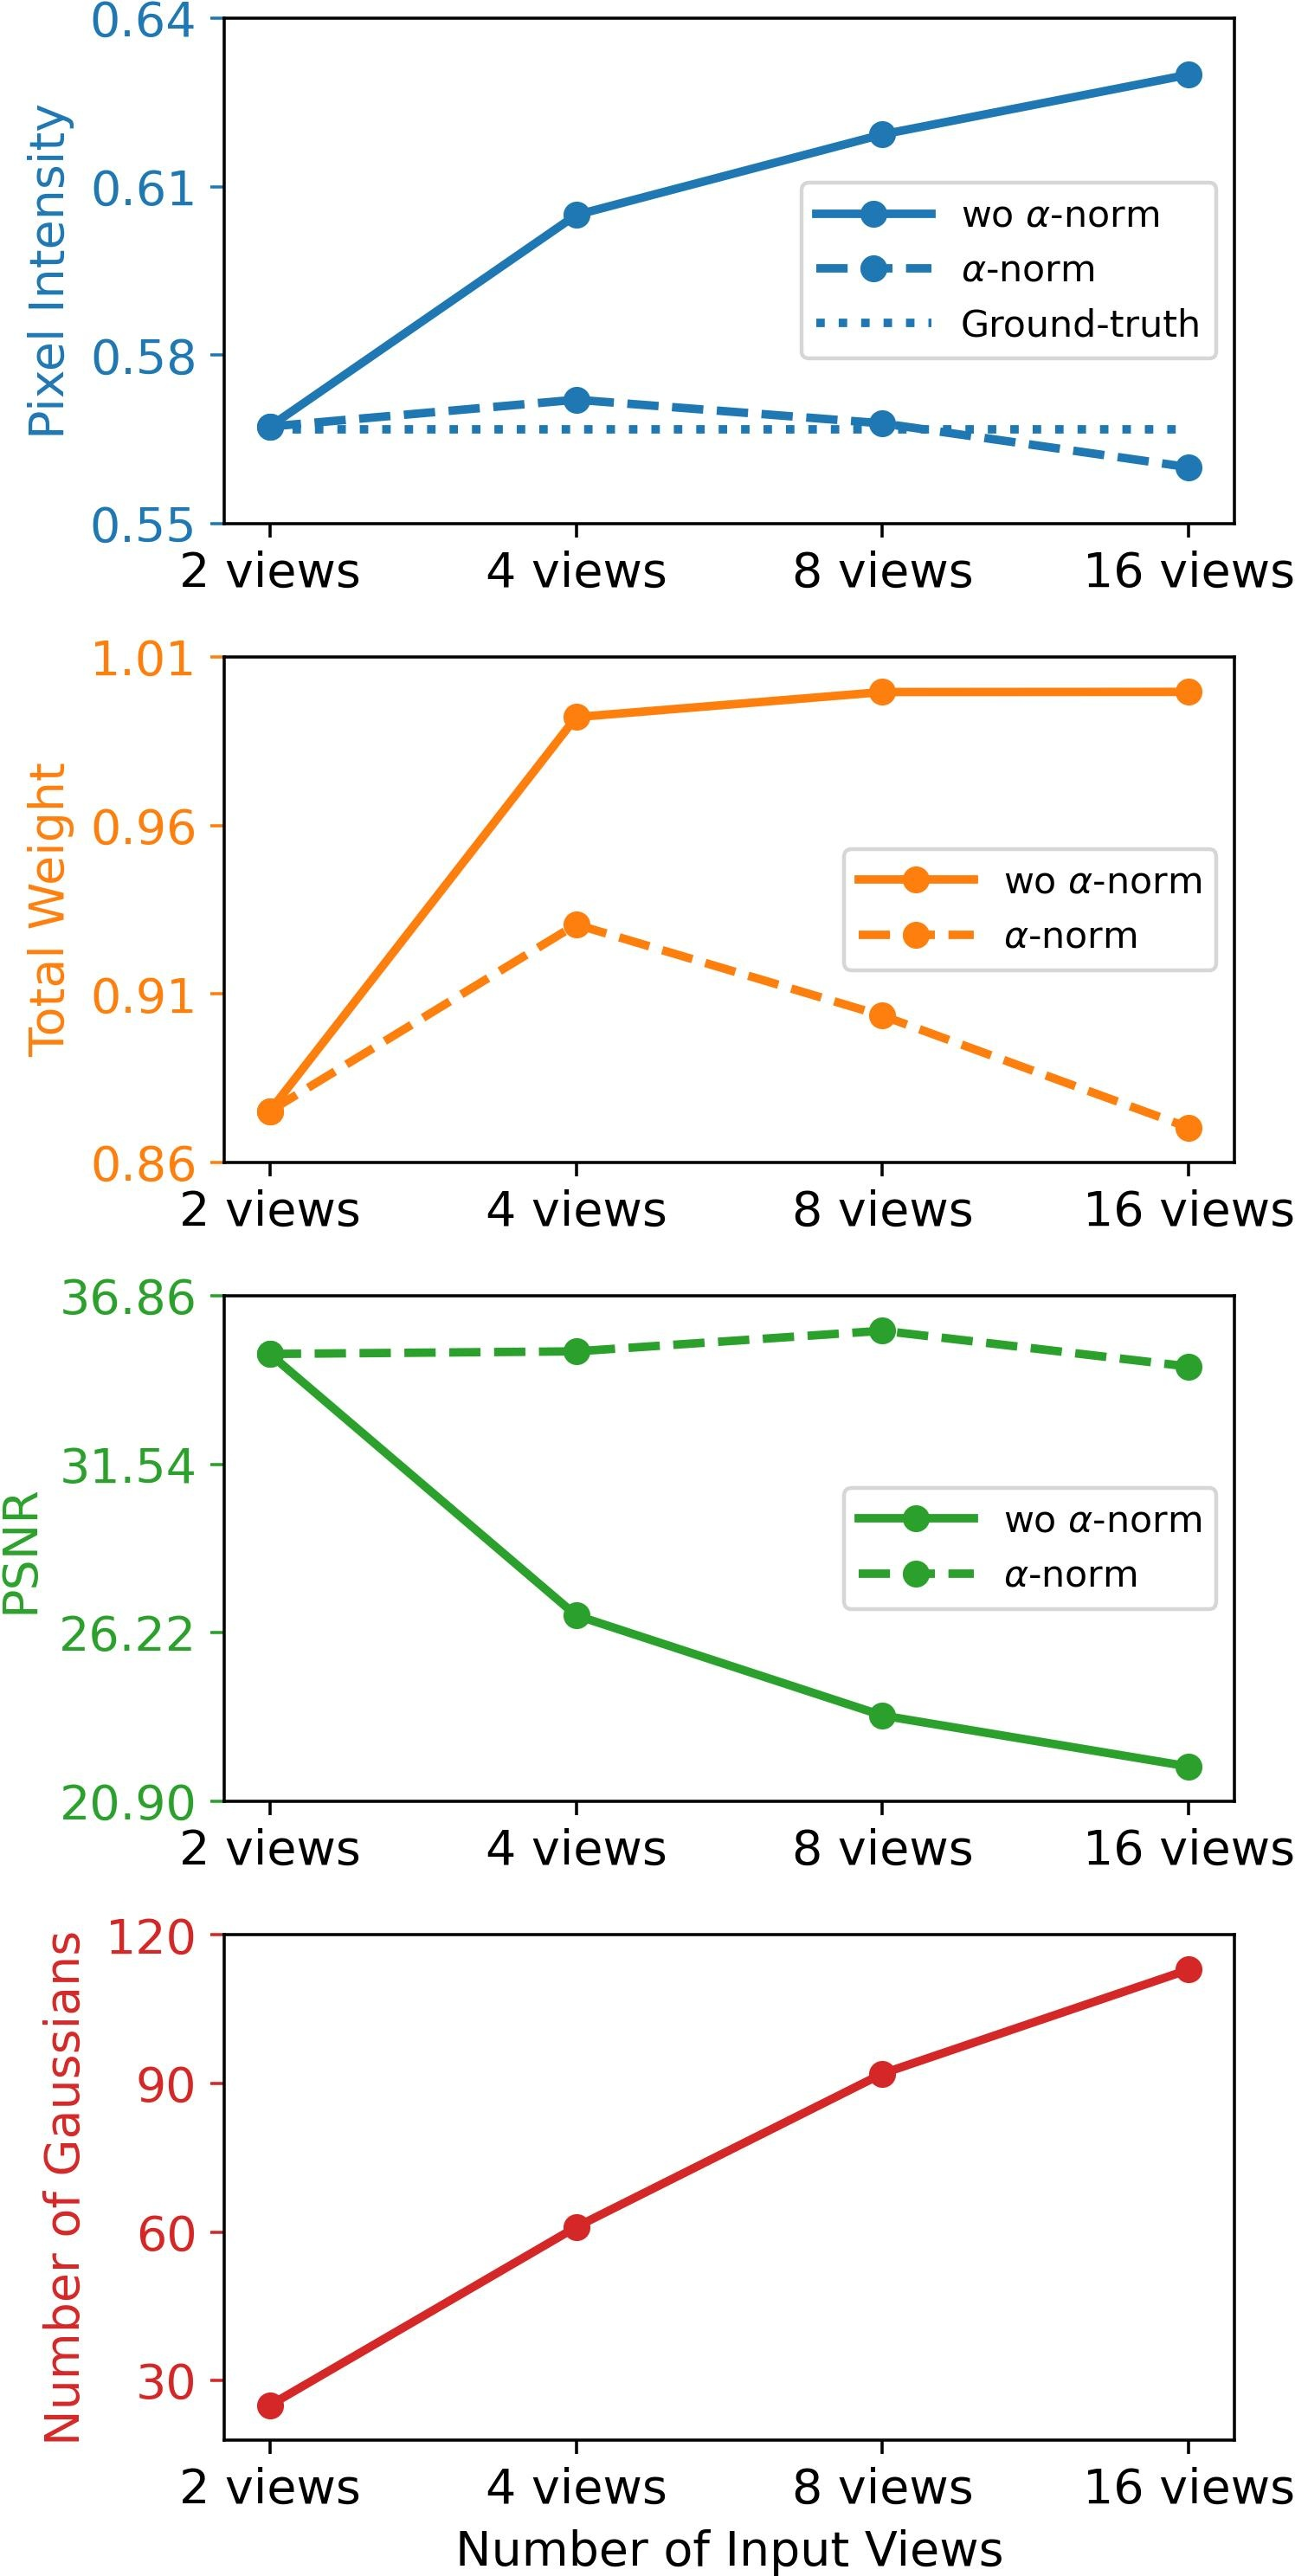} &
    \includegraphics[width=0.32\linewidth]{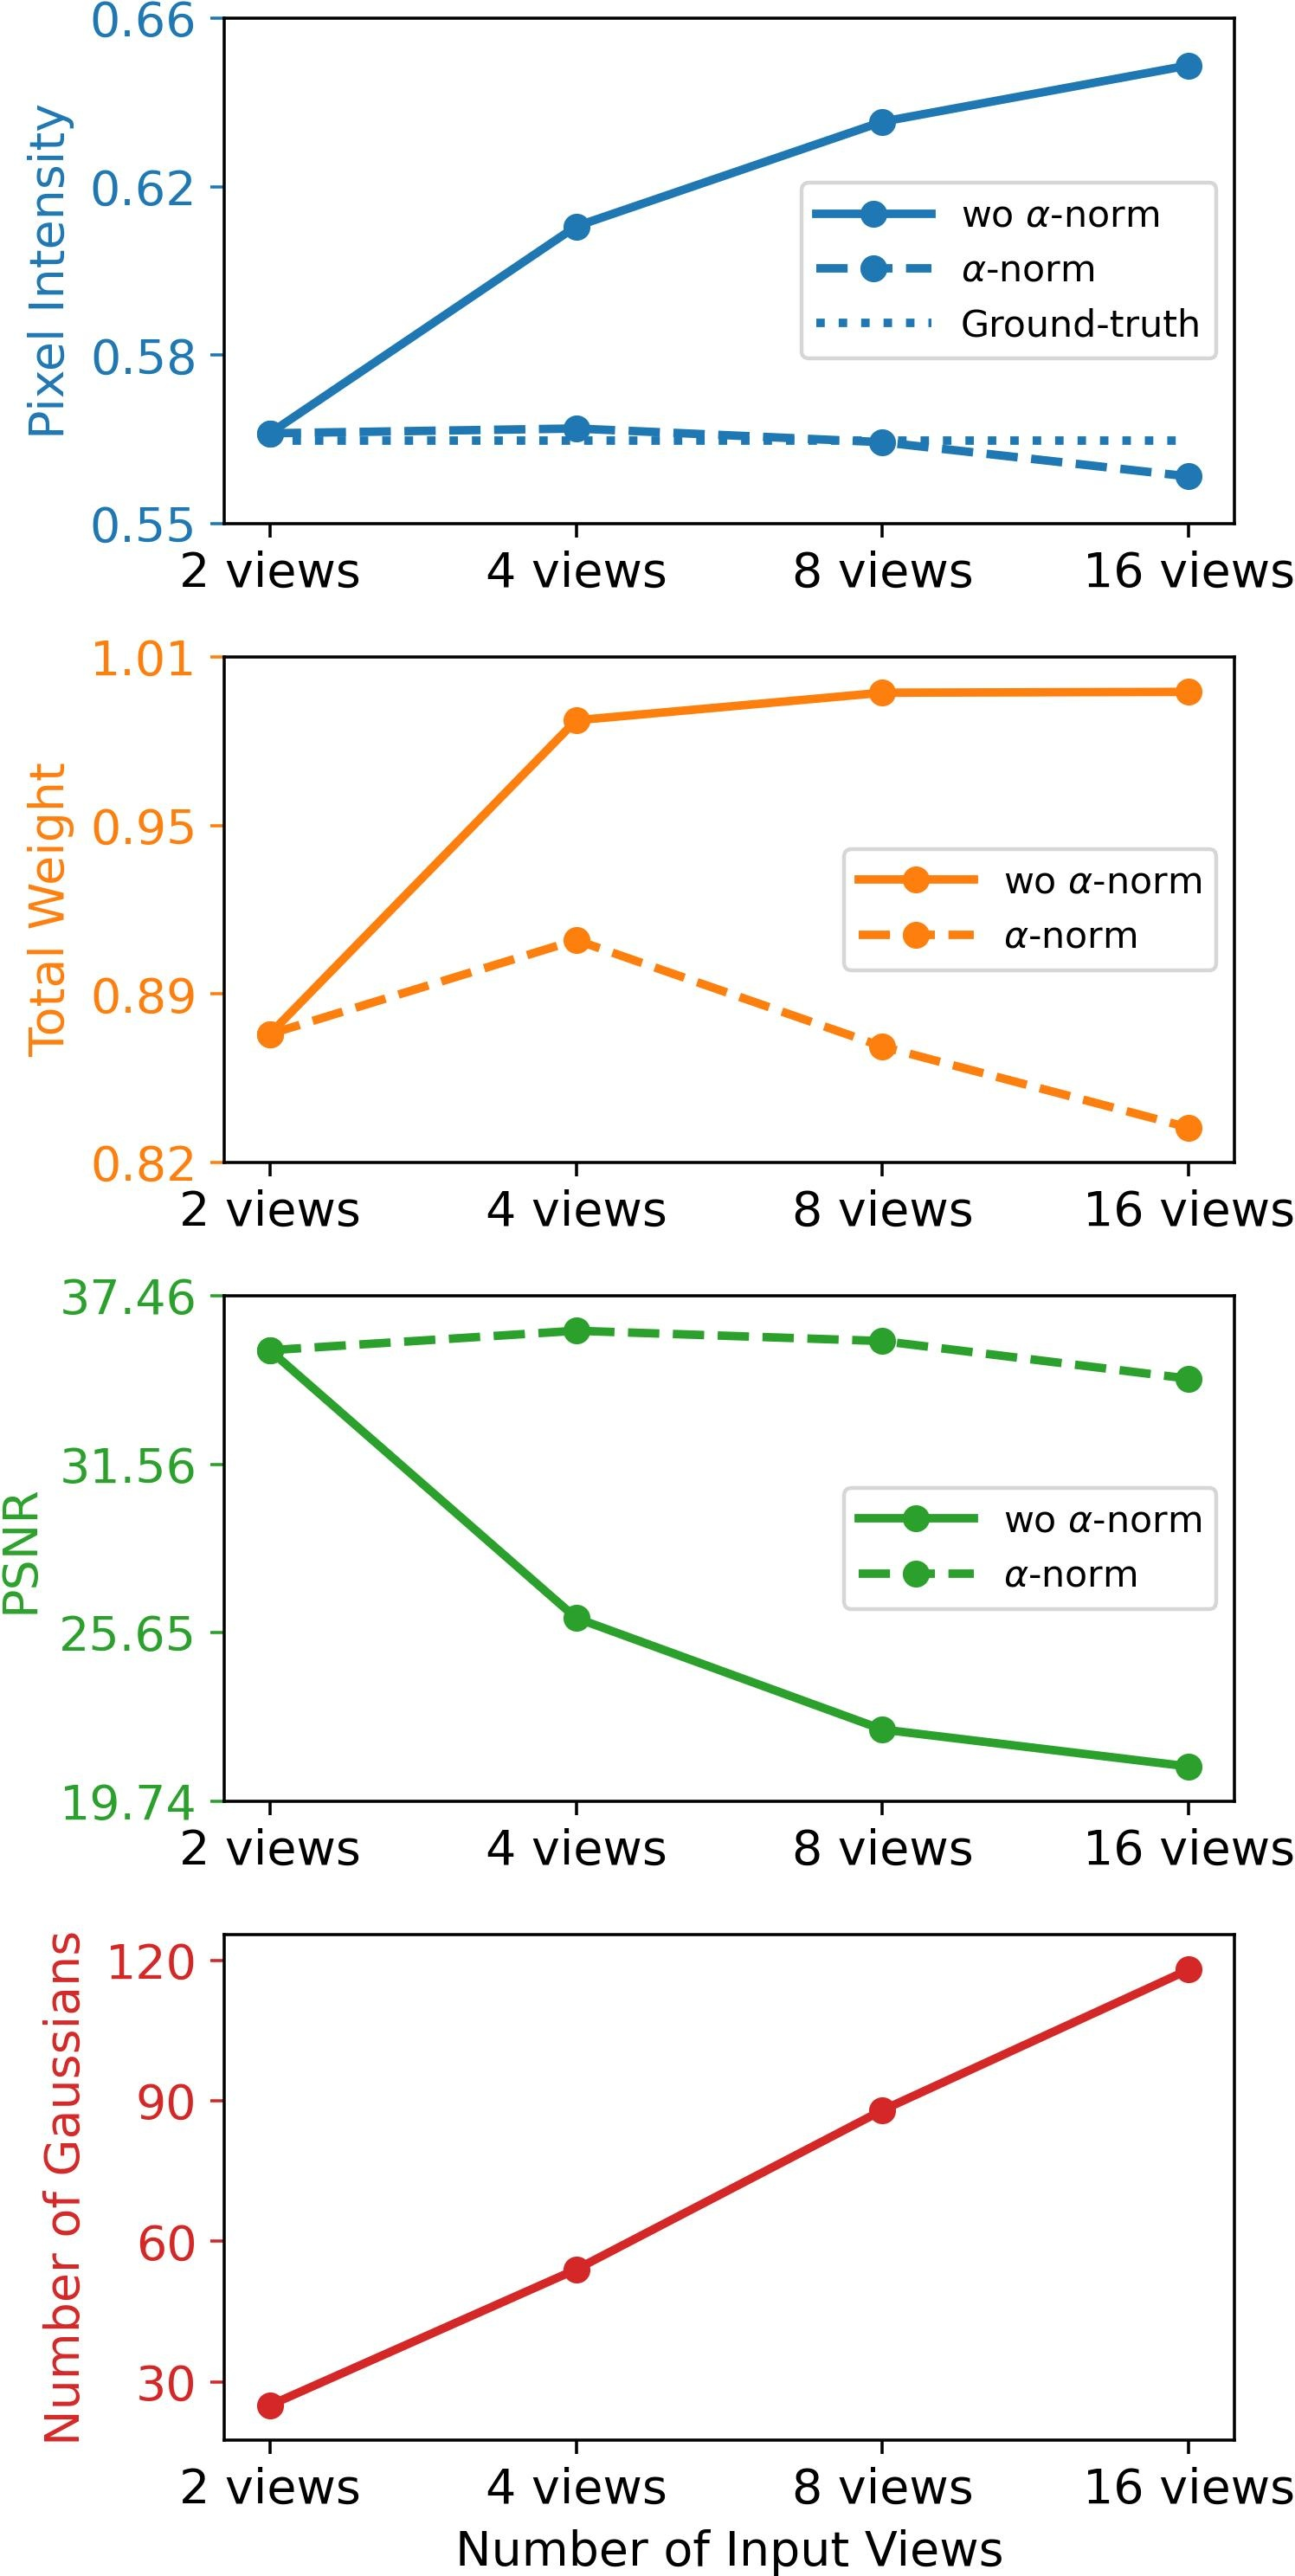} &
    \includegraphics[width=0.32\linewidth]{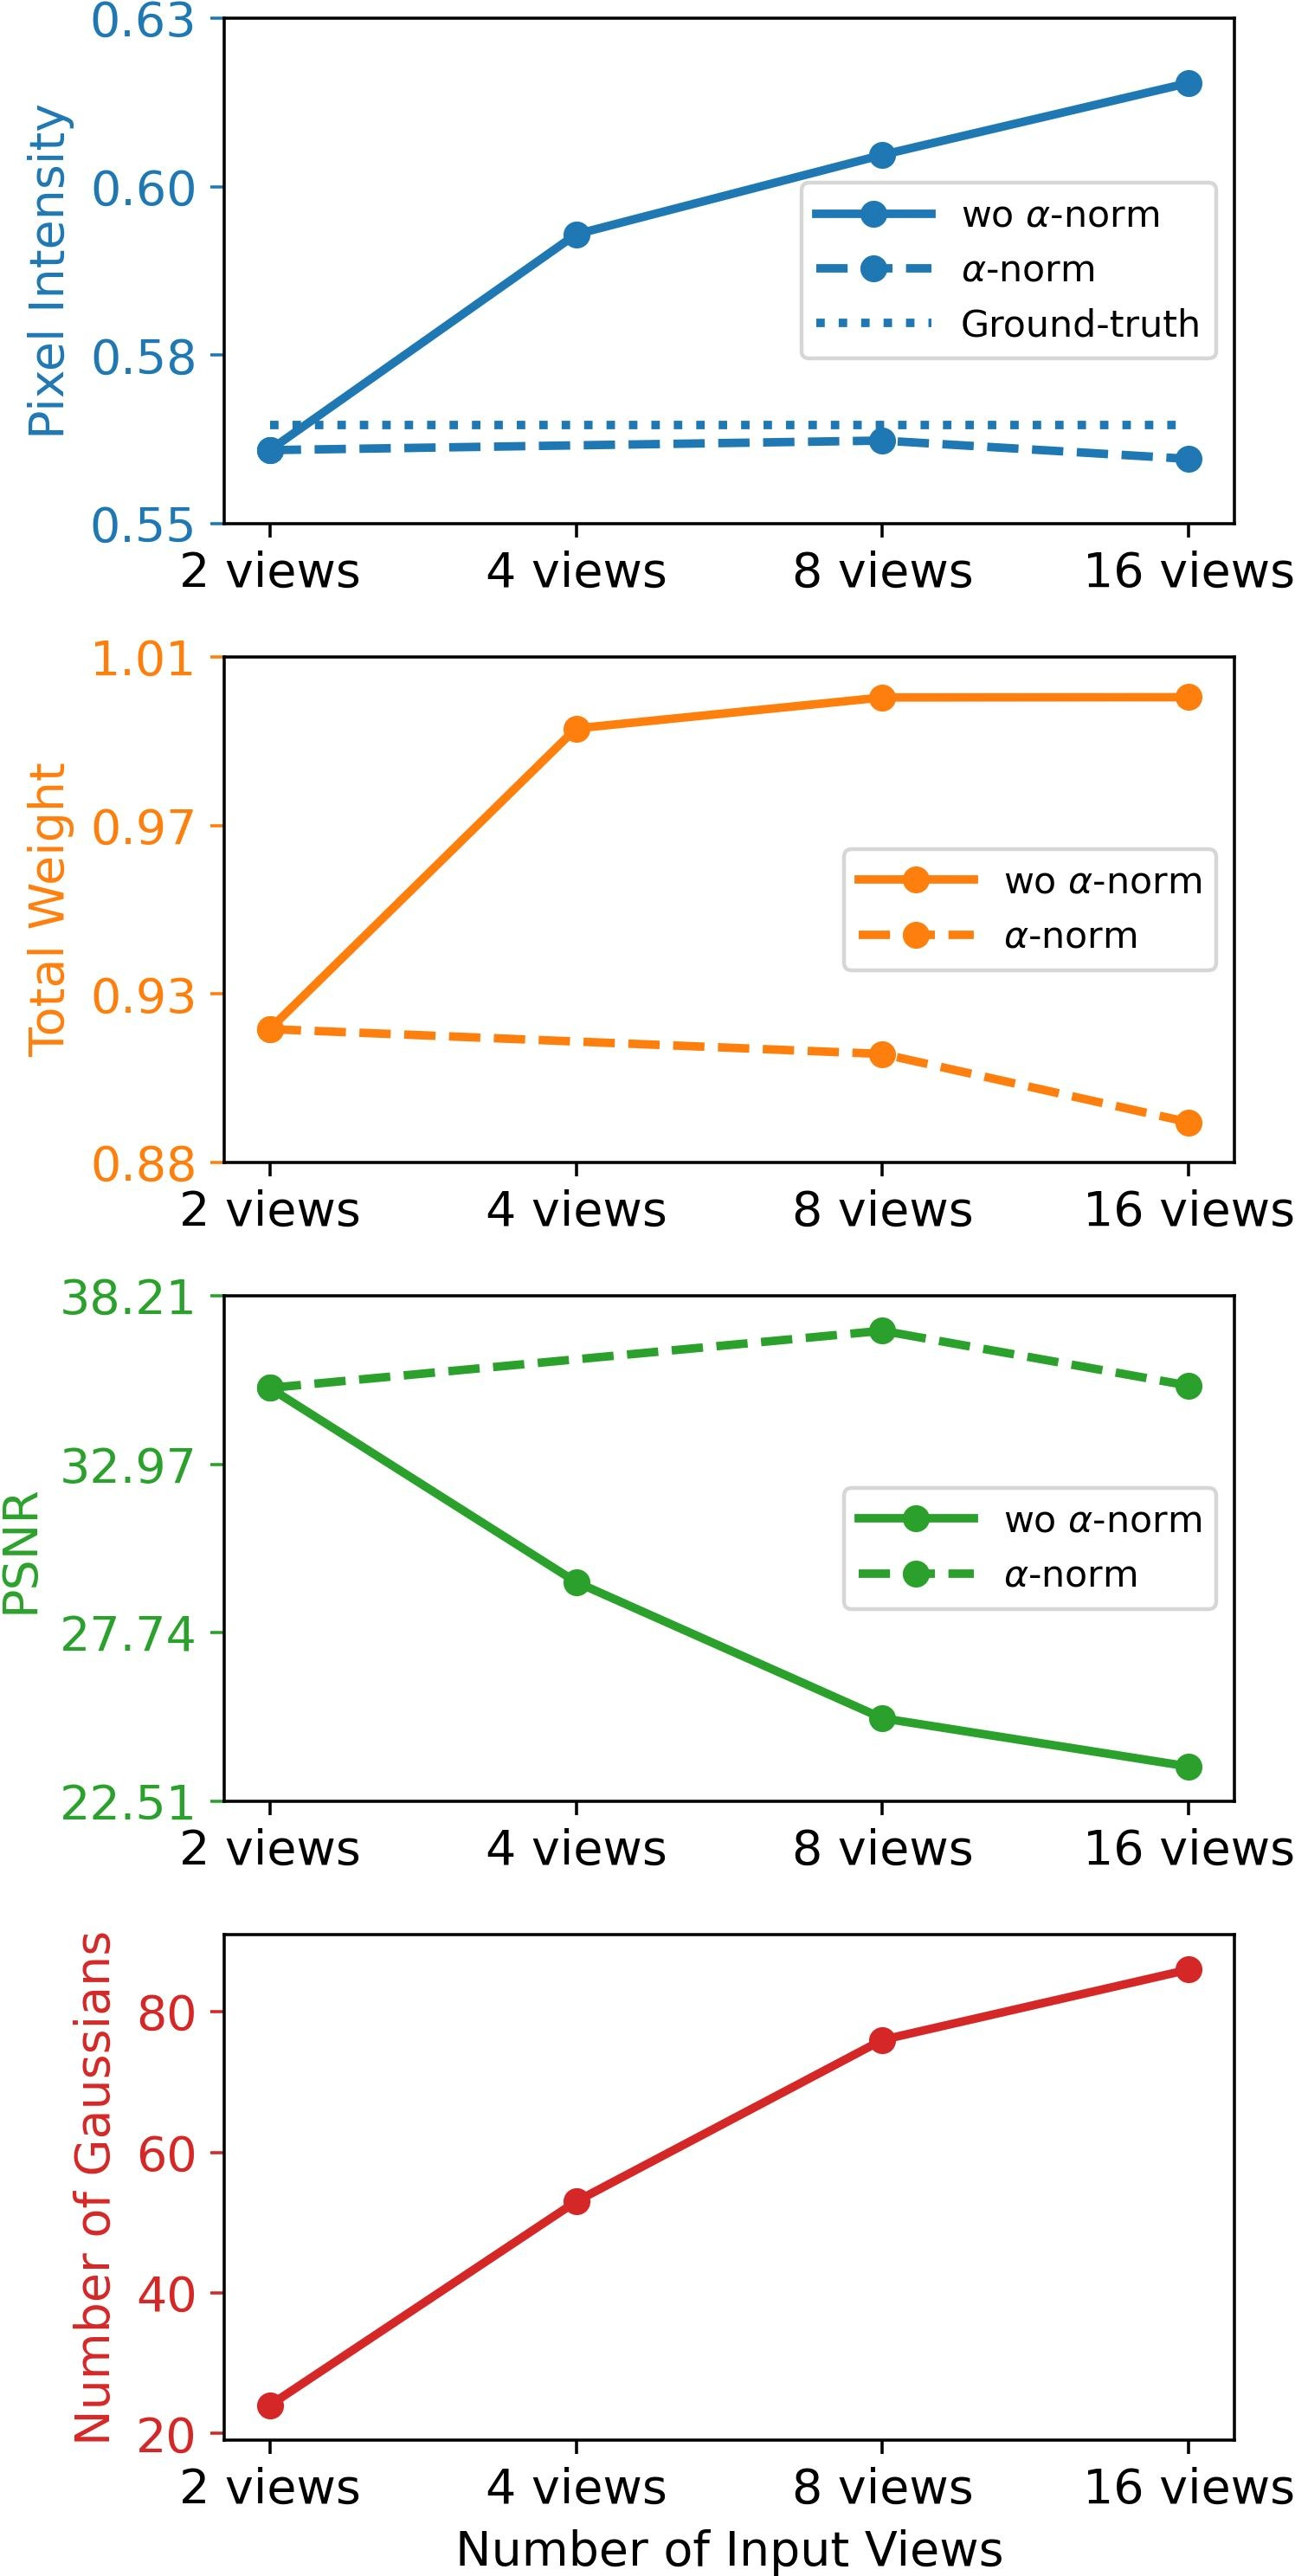} \\
    \end{tabular}
    
    \caption{Pixel intensity, accumulated compositing weight, image quality (PSNR), and number of predicted Gaussians under varying input-view counts. \textbf{First row}: Median gray-scale pixel intensity across the whole image. \textbf{Second row}: Median total accumulated weight across the whole image. \textbf{Third row}: Image quality measured via PSNR. \textbf{Last row}: Median number of Gaussians used for rendering. To compute this, we first obtain the number of Gaussians involve in the rendering process for each pixel, then compute the median value across all pixels. \textbf{Analysis}: Increasing the number of input views causes existing feed-forward Gaussian Splatting methods~\cite{chen2024mvsplat, zhang2025transplat, xu2025depthsplat} to predict more overlapping Gaussians (last row), which increases the accumulated compositing weight $W$ (second row), raises pixel intensity (first row), leading to overbright images and PSNR degradation (third row). Our alpha normalization mitigates this effect by stabilizing $W$, leading to more consistent brightness and improved rendering quality.}
    \label{fig:alpha_norm_curve}
\end{figure}
