# Supplementary material for: RoSplat: Robust Feed-Forward Pixel-wise Gaussian Splatting for Varying Input Views and High-Resolution Rendering
Source: arXiv:2605.13093 source file (2026-05-13)
Supplement: Supplementary file 7 [file depth_sensitivity.tex]

\begin{figure}[t]
    \centering
    \includegraphics[width=\textwidth]{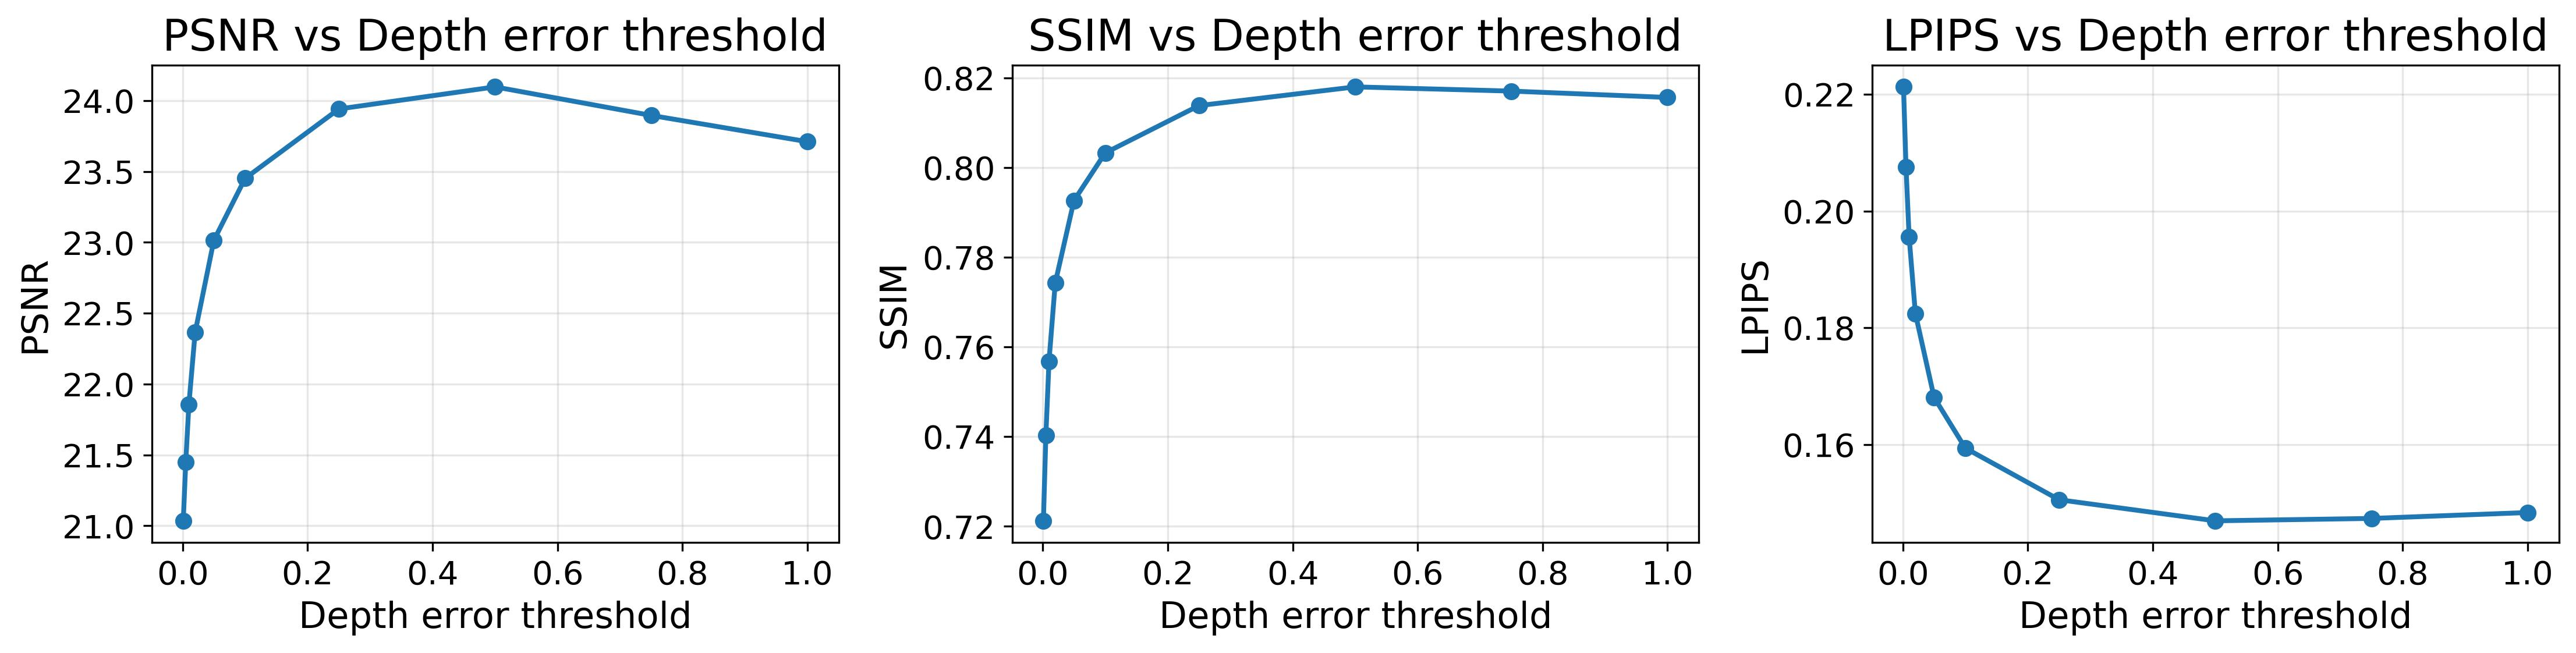}
    \caption{\textbf{Sensitivity to depth error threshold}. Using a threshold of 0.5 results in the best image quality across all metrics.}
    \label{fig:depth_sensitivity}
\end{figure}
