# Supplementary material for: RoSplat: Robust Feed-Forward Pixel-wise Gaussian Splatting for Varying Input Views and High-Resolution Rendering
Source: arXiv:2605.13093 source file (2026-05-13)
Supplement: Supplementary file 8 [file gaussians.tex]

\begin{figure}
    \centering
    \includegraphics[width=0.78\textwidth]{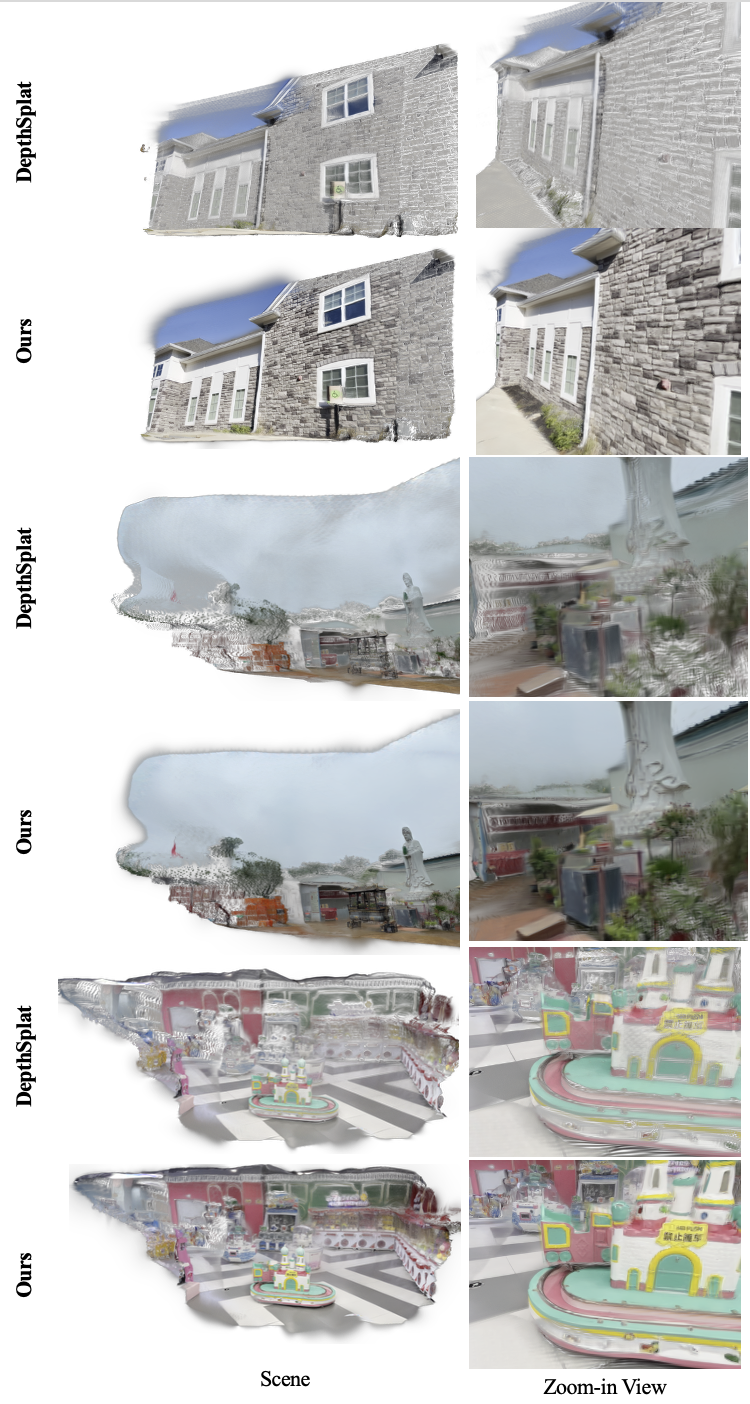}
    \caption{\textbf{Gaussians visualizations on the DL3DV dataset}. We can see that scenes reconstructed by DepthSplat~\cite{xu2025depthsplat} show many hole artifacts in zoom-in views, while ours shows few or even no hole artifacts (white cracked areas in above figures).}
    \label{fig:gaussian_visualization}
\end{figure}
