# Supplementary material for: RoSplat: Robust Feed-Forward Pixel-wise Gaussian Splatting for Varying Input Views and High-Resolution Rendering
Source: arXiv:2605.13093 source file (2026-05-13)
Supplement: Supplementary file 10 [file zoomin_evaluation.tex]

\begin{table}[t]
\centering
\scriptsize
\caption{\textbf{Comparison on the DL3DV dataset under zoom-in rendering}. Our method significantly outperforms DepthSplat, and the performance gaps increases as the zoom-in factor increases.}
\resizebox{\textwidth}{!}{%
\begin{tblr}{
  colsep  = 1.5pt,
  rowsep  = 1pt,
  column{even} = {c},
  column{3} = {c},
  column{5} = {c},
  column{7} = {c},
  column{9} = {c},
  column{11} = {c},
  column{13} = {c},
  cell{1}{2} = {c=3}{},
  cell{1}{6} = {c=3}{},
  cell{1}{9} = {c=3}{},
  cell{1}{12} = {c=3}{},
  cell{3}{2} = {font=\bfseries},
  cell{3}{3} = {font=\bfseries},
  cell{3}{4} = {font=\bfseries},
  cell{4}{6} = {font=\bfseries},
  cell{4}{7} = {font=\bfseries},
  cell{4}{8} = {font=\bfseries},
  cell{4}{9} = {font=\bfseries},
  cell{4}{10} = {font=\bfseries},
  cell{4}{11} = {font=\bfseries},
  cell{4}{12} = {font=\bfseries},
  cell{4}{13} = {font=\bfseries},
  cell{4}{14} = {font=\bfseries},
  vline{2} = {1}{Black},
  vline{3,6-7,10,13} = {1}{},
  vline{2,5-6,9,12} = {1-5}{Black},
  hline{3} = {1,4,6,8,11,14}{},
  hline{3} = {2-3,7,9-10,12-13}{Black},
  hline{5} = {1,4,6,8,11,14}{},
  hline{5} = {2-3,7,9-10,12-13}{Black}
}
           & $1\times$ zoom-in &        &       &   & $2\times$ zoom-in  &       &        & $4\times$ zoom-in  &       &        & $8\times$ zoom-in  &       &        \\
           & PSNR $\uparrow$        & SSIM $\uparrow$  & LPIPS $\downarrow$ & ~ & PSNR $\uparrow$           & SSIM $\uparrow$ & LPIPS $\downarrow$ & PSNR $\uparrow$            & SSIM $\uparrow$ & LPIPS $\downarrow$ & PSNR $\uparrow$           & SSIM $\uparrow$  & LPIPS  $\downarrow$  \\
DepthSplat & 24.17 & 0.819 & 0.145 & & 19.95 & 0.676 & 0.272 & 17.05 & 0.528 & 0.436 & 16.07 & 0.512 & 0.511  \\
Ours        & 24.10 & 0.818 & 0.147 & & 20.84 & 0.692 & 0.263 & 18.79 & 0.587 & 0.398 & \textbf{18.19} & \textbf{0.586} & \textbf{0.477}  \\
~           & \textcolor{orange}{-0.07} & \textcolor{orange}{-0.001} & \textcolor{orange}{+0.002} & & \textcolor{Green}{+0.89} & \textcolor{Green}{+0.016} & \textcolor{Green}{-0.009} & \textcolor{Green}{+1.74} & \textcolor{Green}{+0.059} & \textcolor{Green}{-0.038} & \textcolor{Green}{+2.12} & \textcolor{Green}{+0.074} & \textcolor{Green}{-0.034} 
\end{tblr}
}
\label{tab:zoomed_in_comparision}
\end{table}
