# Supplementary material for: RoSplat: Robust Feed-Forward Pixel-wise Gaussian Splatting for Varying Input Views and High-Resolution Rendering
Source: arXiv:2605.13093 source file (2026-05-13)
Supplement: Supplementary file 11 [file zoom_in_evaluation.tex]

\section{Zoom-in Rendering}
Tab.~\ref{tab:zoomed_in_comparision} compares our method with DepthSplat under centered zoom-in rendering. Specifically, we render zoomed-in images by multiplying the focal length by the zoom factor while keeping the principal point fixed at the image center. All zoomed-in images are rendered at the training resolution of $256\times 448$. To construct the corresponding ground-truth images, we center-crop high-resolution images so that they match the same zoom factor. For example, the ground-truth image for $8\times$ zoom-in is obtained by center-cropping the corresponding $8\times$ higher-resolution ground-truth image to a resolution of $256\times 448$. Tab.~\ref{tab:zoomed_in_comparision} shows that our method achieves better image quality than DepthSplat under zoom-in rendering. Moreover, the performance gap increases as the zoom factor increases. These results further demonstrate the effectiveness of our 3D sampling-based strategy for improving Gaussian scale estimation.
